# Supplementary material for: Cognitive Maps in Large Language Models
Source: arXiv:2610.25596 source file (2026-11-06)
Supplement: Supplementary file 1 [file figure_macros.tex]

\newenvironment{figurepanel}[3][0pt]{%
    \begin{minipage}[t]{#3}%
        \raggedright\textbf{#2}\par\smallskip
        \vspace{#1}%
        \centering
}{%
    \end{minipage}%
}

\newcommand{\sixpanelgrid}[7]{%
    \begin{figurepanel}{A}{0.27\textwidth}#1\end{figurepanel}\hfill
    \begin{figurepanel}{C}{0.27\textwidth}#3\end{figurepanel}\hfill
    \begin{figurepanel}{E}{0.27\textwidth}#5\end{figurepanel}
    \par\smallskip
    \begin{figurepanel}{B}{0.27\textwidth}#2\end{figurepanel}\hfill
    \begin{figurepanel}{D}{0.27\textwidth}#4\end{figurepanel}\hfill
    \begin{figurepanel}{F}{0.27\textwidth}#6\end{figurepanel}
    \par\smallskip
    #7
}

\newcommand{\fivepanelgrid}[6]{%
    \begin{figurepanel}{A}{0.27\textwidth}#1\end{figurepanel}\hfill
    \begin{figurepanel}{C}{0.27\textwidth}#3\end{figurepanel}\hfill
    \begin{figurepanel}{E}{0.27\textwidth}#5\end{figurepanel}
    \par\smallskip
    \begin{figurepanel}{B}{0.27\textwidth}#2\end{figurepanel}\hfill
    \begin{figurepanel}{D}{0.27\textwidth}#4\end{figurepanel}\hfill
    \begin{minipage}[t]{0.27\textwidth}\mbox{}\end{minipage}
    \par\smallskip
    #6
}

\newcommand{\fourpanelrowwithlegend}[5]{%
    \begin{figurepanel}{A}{0.24\textwidth}#1\end{figurepanel}\hfill
    \begin{figurepanel}{B}{0.24\textwidth}#2\end{figurepanel}\hfill
    \begin{figurepanel}{C}{0.24\textwidth}#3\end{figurepanel}\hfill
    \begin{figurepanel}{D}{0.24\textwidth}#4\end{figurepanel}
    \par\smallskip
    #5
}

\newcommand{\twopanelrow}[3]{%
    \begin{figurepanel}{A}{0.24\textwidth}#1\end{figurepanel}\hspace{0.02\textwidth}%
    \begin{figurepanel}{B}{0.24\textwidth}#2\end{figurepanel}
    \par\smallskip
    #3
}

\newcommand{\behaviorpanels}[2]{%
    \begin{figurepanel}{A}{0.38\textwidth}#1\end{figurepanel}\hspace{0.04\textwidth}%
    \begin{figurepanel}[2pt]{B}{0.27\textwidth}#2\end{figurepanel}%
}

\newsavebox{\behaviorplotbox}
\newsavebox{\behaviorlegendbox}
\newcommand{\behaviorpanelswithlegend}[3]{%
    \sbox{\behaviorplotbox}{#2}%
    \sbox{\behaviorlegendbox}{#3}%
    \begin{figurepanel}{A}{0.5\textwidth}#1\end{figurepanel}%
    \begin{minipage}[t]{0.49\textwidth}
        \raggedright\textbf{B}\par\smallskip
        \raisebox{-2pt}[\ht\behaviorplotbox][\dp\behaviorplotbox]{%
            \usebox{\behaviorplotbox}}%
        \hspace{2pt}%
        \raisebox{\dimexpr(\ht\behaviorplotbox-\ht\behaviorlegendbox)/2\relax}{%
            \usebox{\behaviorlegendbox}}%
    \end{minipage}%
}

\newcommand{\erasurepanels}[5]{%
    \begin{figurepanel}{A}{0.31\textwidth}#1\end{figurepanel}
    \begin{figurepanel}[7pt]{B}{0.21\textwidth}#2\end{figurepanel} \hspace{10pt}
    \begin{figurepanel}{C}{0.42\textwidth}#3\end{figurepanel}
    \par\medskip
    \begin{figurepanel}{D}{0.35\textwidth}#4\end{figurepanel}
    \begin{figurepanel}{E}{0.35\textwidth}#5\end{figurepanel}
}

\newcommand{\fourpaneltable}[4]{%
    \begingroup
    \setlength{\tabcolsep}{0pt}%
    \begin{tabular}{@{}cccc@{}}
        \makebox[0.25\textwidth][l]{\textbf{A}} &
        \makebox[0.25\textwidth][l]{\textbf{B}} &
        \makebox[0.25\textwidth][l]{\textbf{C}} &
        \makebox[0.25\textwidth][l]{\textbf{D}} \\[3pt]
        #1 & #2 & #3 & #4
    \end{tabular}%
    \endgroup
}
