# Supplementary material for: Cognitive Maps in Large Language Models
Source: arXiv:2610.25596 source file (2026-11-06)
Supplement: Supplementary file 2 [file references.tex]

%apsrev4-2.bst 2019-01-14 (MD) hand-edited version of apsrev4-1.bst
%Control: key (0)
%Control: author (72) initials jnrlst
%Control: editor formatted (1) identically to author
%Control: production of article title (-1) disabled
%Control: page (0) single
%Control: year (1) truncated
%Control: production of eprint (0) enabled
\begin{thebibliography}{14}%
\makeatletter
\providecommand \@ifxundefined [1]{%
 \@ifx{#1\undefined}
}%
\providecommand \@ifnum [1]{%
 \ifnum #1\expandafter \@firstoftwo
 \else \expandafter \@secondoftwo
 \fi
}%
\providecommand \@ifx [1]{%
 \ifx #1\expandafter \@firstoftwo
 \else \expandafter \@secondoftwo
 \fi
}%
\providecommand \natexlab [1]{#1}%
\providecommand \enquote  [1]{``#1''}%
\providecommand \bibnamefont  [1]{#1}%
\providecommand \bibfnamefont [1]{#1}%
\providecommand \citenamefont [1]{#1}%
\providecommand \href@noop [0]{\@secondoftwo}%
\providecommand \href [0]{\begingroup \@sanitize@url \@href}%
\providecommand \@href[1]{\@@startlink{#1}\@@href}%
\providecommand \@@href[1]{\endgroup#1\@@endlink}%
\providecommand \@sanitize@url [0]{\catcode `\\12\catcode `\$12\catcode
  `\&12\catcode `\#12\catcode `\^12\catcode `\_12\catcode `\%12\relax}%
\providecommand \@@startlink[1]{}%
\providecommand \@@endlink[0]{}%
\providecommand \url  [0]{\begingroup\@sanitize@url \@url }%
\providecommand \@url [1]{\endgroup\@href {#1}{\urlprefix }}%
\providecommand \urlprefix  [0]{URL }%
\providecommand \Eprint [0]{\href }%
\providecommand \doibase [0]{https://doi.org/}%
\providecommand \selectlanguage [0]{\@gobble}%
\providecommand \bibinfo  [0]{\@secondoftwo}%
\providecommand \bibfield  [0]{\@secondoftwo}%
\providecommand \translation [1]{[#1]}%
\providecommand \BibitemOpen [0]{}%
\providecommand \bibitemStop [0]{}%
\providecommand \bibitemNoStop [0]{.\EOS\space}%
\providecommand \EOS [0]{\spacefactor3000\relax}%
\providecommand \BibitemShut  [1]{\csname bibitem#1\endcsname}%
\let\auto@bib@innerbib\@empty
%</preamble>
\bibitem [{\citenamefont {Vaswani}\ \emph {et~al.}(2017)\citenamefont
  {Vaswani}, \citenamefont {Shazeer}, \citenamefont {Parmar}, \citenamefont
  {Uszkoreit}, \citenamefont {Jones}, \citenamefont {Gomez}, \citenamefont
  {Kaiser},\ and\ \citenamefont {Polosukhin}}]{SI-vaswani_2017_transformer}%
  \BibitemOpen
  \bibfield  {author} {\bibinfo {author} {\bibfnamefont {A.}~\bibnamefont
  {Vaswani}}, \bibinfo {author} {\bibfnamefont {N.}~\bibnamefont {Shazeer}},
  \bibinfo {author} {\bibfnamefont {N.}~\bibnamefont {Parmar}}, \bibinfo
  {author} {\bibfnamefont {J.}~\bibnamefont {Uszkoreit}}, \bibinfo {author}
  {\bibfnamefont {L.}~\bibnamefont {Jones}}, \bibinfo {author} {\bibfnamefont
  {A.~N.}\ \bibnamefont {Gomez}}, \bibinfo {author} {\bibfnamefont
  {{\L}.}~\bibnamefont {Kaiser}},\ and\ \bibinfo {author} {\bibfnamefont
  {I.}~\bibnamefont {Polosukhin}},\ }in\ \href
  {https://papers.nips.cc/paper/2017/hash/3f5ee243547dee91fbd053c1c4a845aa-Abstract.html}
  {\emph {\bibinfo {booktitle} {Advances in Neural Information Processing
  Systems}}},\ Vol.~\bibinfo {volume} {30}\ (\bibinfo  {publisher} {Curran
  Associates, Inc.},\ \bibinfo {year} {2017})\BibitemShut {NoStop}%
\bibitem [{\citenamefont {Gershman}\ \emph {et~al.}(2025)\citenamefont
  {Gershman}, \citenamefont {Fiete},\ and\ \citenamefont
  {Irie}}]{SI-gershman_2025_key_value_memory}%
  \BibitemOpen
  \bibfield  {author} {\bibinfo {author} {\bibfnamefont {S.~J.}\ \bibnamefont
  {Gershman}}, \bibinfo {author} {\bibfnamefont {I.}~\bibnamefont {Fiete}},\
  and\ \bibinfo {author} {\bibfnamefont {K.}~\bibnamefont {Irie}},\ }\href
  {https://doi.org/10.1016/j.neuron.2025.02.029} {\bibfield  {journal}
  {\bibinfo  {journal} {Neuron}\ }\textbf {\bibinfo {volume} {113}},\ \bibinfo
  {pages} {1694} (\bibinfo {year} {2025})}\BibitemShut {NoStop}%
\bibitem [{\citenamefont {{Gemma Team}}(2025)}]{SI-gemma_2025_gemma3}%
  \BibitemOpen
  \bibfield  {author} {\bibinfo {author} {\bibnamefont {{Gemma Team}}},\ }\href
  {https://doi.org/10.48550/arXiv.2503.19786} {\bibinfo {title} {{Gemma 3}
  technical report}} (\bibinfo {year} {2025}),\ \Eprint
  {https://arxiv.org/abs/2503.19786} {arXiv:2503.19786} \BibitemShut {NoStop}%
\bibitem [{\citenamefont {Grattafiori}\ \emph {et~al.}(2024)\citenamefont
  {Grattafiori}, \citenamefont {Dubey}, \citenamefont {Jauhri} \emph
  {et~al.}}]{SI-grattafiori_2024_llama3}%
  \BibitemOpen
  \bibfield  {author} {\bibinfo {author} {\bibfnamefont {A.}~\bibnamefont
  {Grattafiori}}, \bibinfo {author} {\bibfnamefont {A.}~\bibnamefont {Dubey}},
  \bibinfo {author} {\bibfnamefont {A.}~\bibnamefont {Jauhri}}, \emph
  {et~al.},\ }\href {https://doi.org/10.48550/arXiv.2407.21783} {\bibinfo
  {title} {The {Llama 3} herd of models}} (\bibinfo {year} {2024}),\ \Eprint
  {https://arxiv.org/abs/2407.21783} {arXiv:2407.21783} \BibitemShut {NoStop}%
\bibitem [{\citenamefont {Yang}\ \emph {et~al.}(2025)\citenamefont {Yang},
  \citenamefont {Li}, \citenamefont {Yang} \emph {et~al.}}]{SI-yang_2025_qwen3}%
  \BibitemOpen
  \bibfield  {author} {\bibinfo {author} {\bibfnamefont {A.}~\bibnamefont
  {Yang}}, \bibinfo {author} {\bibfnamefont {A.}~\bibnamefont {Li}}, \bibinfo
  {author} {\bibfnamefont {B.}~\bibnamefont {Yang}}, \emph {et~al.},\ }\href
  {https://doi.org/10.48550/arXiv.2505.09388} {\bibinfo {title} {{Qwen3}
  technical report}} (\bibinfo {year} {2025}),\ \Eprint
  {https://arxiv.org/abs/2505.09388} {arXiv:2505.09388} \BibitemShut {NoStop}%
\bibitem [{\citenamefont {Su}\ \emph {et~al.}(2024)\citenamefont {Su},
  \citenamefont {Ahmed}, \citenamefont {Lu}, \citenamefont {Pan}, \citenamefont
  {Wen},\ and\ \citenamefont {Liu}}]{SI-su_2024_roformer}%
  \BibitemOpen
  \bibfield  {author} {\bibinfo {author} {\bibfnamefont {J.}~\bibnamefont
  {Su}}, \bibinfo {author} {\bibfnamefont {M.}~\bibnamefont {Ahmed}}, \bibinfo
  {author} {\bibfnamefont {Y.}~\bibnamefont {Lu}}, \bibinfo {author}
  {\bibfnamefont {S.}~\bibnamefont {Pan}}, \bibinfo {author} {\bibfnamefont
  {B.}~\bibnamefont {Wen}},\ and\ \bibinfo {author} {\bibfnamefont
  {Y.}~\bibnamefont {Liu}},\ }\href
  {https://doi.org/10.1016/j.neucom.2023.127063} {\bibfield  {journal}
  {\bibinfo  {journal} {Neurocomputing}\ }\textbf {\bibinfo {volume} {568}},\
  \bibinfo {pages} {127063} (\bibinfo {year} {2024})}\BibitemShut {NoStop}%
\bibitem [{\citenamefont {Ainslie}\ \emph {et~al.}(2023)\citenamefont
  {Ainslie}, \citenamefont {Lee-Thorp}, \citenamefont {de~Jong}, \citenamefont
  {Zemlyanskiy}, \citenamefont {Lebron},\ and\ \citenamefont
  {Sanghai}}]{SI-ainslie_2023_gqa}%
  \BibitemOpen
  \bibfield  {author} {\bibinfo {author} {\bibfnamefont {J.}~\bibnamefont
  {Ainslie}}, \bibinfo {author} {\bibfnamefont {J.}~\bibnamefont {Lee-Thorp}},
  \bibinfo {author} {\bibfnamefont {M.}~\bibnamefont {de~Jong}}, \bibinfo
  {author} {\bibfnamefont {Y.}~\bibnamefont {Zemlyanskiy}}, \bibinfo {author}
  {\bibfnamefont {F.}~\bibnamefont {Lebron}},\ and\ \bibinfo {author}
  {\bibfnamefont {S.}~\bibnamefont {Sanghai}},\ }in\ \href
  {https://doi.org/10.18653/v1/2023.emnlp-main.298} {\emph {\bibinfo
  {booktitle} {Proceedings of the 2023 Conference on Empirical Methods in
  Natural Language Processing}}}\ (\bibinfo  {publisher} {Association for
  Computational Linguistics},\ \bibinfo {year} {2023})\ pp.\ \bibinfo {pages}
  {4895--4901}\BibitemShut {NoStop}%
\bibitem [{\citenamefont {Feng}\ and\ \citenamefont
  {Steinhardt}(2024)}]{SI-feng2024entities}%
  \BibitemOpen
  \bibfield  {author} {\bibinfo {author} {\bibfnamefont {J.}~\bibnamefont
  {Feng}}\ and\ \bibinfo {author} {\bibfnamefont {J.}~\bibnamefont
  {Steinhardt}},\ }in\ \href@noop {} {\emph {\bibinfo {booktitle}
  {International Conference on Learning Representations}}}\ (\bibinfo {year}
  {2024})\BibitemShut {NoStop}%
\bibitem [{\citenamefont {Norman}\ \emph {et~al.}(2006)\citenamefont {Norman},
  \citenamefont {Polyn}, \citenamefont {Detre},\ and\ \citenamefont
  {Haxby}}]{SI-norman2006beyond}%
  \BibitemOpen
  \bibfield  {author} {\bibinfo {author} {\bibfnamefont {K.~A.}\ \bibnamefont
  {Norman}}, \bibinfo {author} {\bibfnamefont {S.~M.}\ \bibnamefont {Polyn}},
  \bibinfo {author} {\bibfnamefont {G.~J.}\ \bibnamefont {Detre}},\ and\
  \bibinfo {author} {\bibfnamefont {J.~V.}\ \bibnamefont {Haxby}},\ }\href
  {https://doi.org/10.1016/j.tics.2006.07.005} {\bibfield  {journal} {\bibinfo
  {journal} {Trends in Cognitive Sciences}\ }\textbf {\bibinfo {volume} {10}},\
  \bibinfo {pages} {424} (\bibinfo {year} {2006})}\BibitemShut {NoStop}%
\bibitem [{\citenamefont {Paninski}\ \emph {et~al.}(2007)\citenamefont
  {Paninski}, \citenamefont {Pillow},\ and\ \citenamefont
  {Lewi}}]{SI-paninski2007statistical}%
  \BibitemOpen
  \bibfield  {author} {\bibinfo {author} {\bibfnamefont {L.}~\bibnamefont
  {Paninski}}, \bibinfo {author} {\bibfnamefont {J.}~\bibnamefont {Pillow}},\
  and\ \bibinfo {author} {\bibfnamefont {J.}~\bibnamefont {Lewi}},\ }in\ \href
  {https://doi.org/10.1016/S0079-6123(06)65031-0} {\emph {\bibinfo {booktitle}
  {Computational Neuroscience: Theoretical Insights into Brain Function}}},\
  \bibinfo {series} {Progress in Brain Research}, Vol.\ \bibinfo {volume}
  {165},\ \bibinfo {editor} {edited by\ \bibinfo {editor} {\bibfnamefont
  {P.}~\bibnamefont {Cisek}}, \bibinfo {editor} {\bibfnamefont
  {T.}~\bibnamefont {Drew}},\ and\ \bibinfo {editor} {\bibfnamefont {J.~F.}\
  \bibnamefont {Kalaska}}}\ (\bibinfo  {publisher} {Elsevier},\ \bibinfo {year}
  {2007})\ pp.\ \bibinfo {pages} {493--507}\BibitemShut {NoStop}%
\bibitem [{\citenamefont {Jarvik}\ and\ \citenamefont
  {Botstein}(1973)}]{SI-jarvik1973genetic}%
  \BibitemOpen
  \bibfield  {author} {\bibinfo {author} {\bibfnamefont {J.}~\bibnamefont
  {Jarvik}}\ and\ \bibinfo {author} {\bibfnamefont {D.}~\bibnamefont
  {Botstein}},\ }\href {https://doi.org/10.1073/pnas.70.7.2046} {\bibfield
  {journal} {\bibinfo  {journal} {Proceedings of the National Academy of
  Sciences}\ }\textbf {\bibinfo {volume} {70}},\ \bibinfo {pages} {2046}
  (\bibinfo {year} {1973})}\BibitemShut {NoStop}%
\bibitem [{\citenamefont {Olsson}\ \emph {et~al.}(2022)\citenamefont {Olsson},
  \citenamefont {Elhage}, \citenamefont {Nanda}, \citenamefont {Joseph},
  \citenamefont {DasSarma}, \citenamefont {Henighan}, \citenamefont {Mann},
  \citenamefont {Askell}, \citenamefont {Bai}, \citenamefont {Chen},
  \citenamefont {Conerly}, \citenamefont {Drain}, \citenamefont {Ganguli},
  \citenamefont {Hatfield-Dodds}, \citenamefont {Hernandez}, \citenamefont
  {Johnston}, \citenamefont {Jones}, \citenamefont {Kernion}, \citenamefont
  {Lovitt}, \citenamefont {Ndousse}, \citenamefont {Amodei}, \citenamefont
  {Brown}, \citenamefont {Clark}, \citenamefont {Kaplan}, \citenamefont
  {McCandlish},\ and\ \citenamefont {Olah}}]{SI-olsson2022induction}%
  \BibitemOpen
  \bibfield  {author} {\bibinfo {author} {\bibfnamefont {C.}~\bibnamefont
  {Olsson}}, \bibinfo {author} {\bibfnamefont {N.}~\bibnamefont {Elhage}},
  \bibinfo {author} {\bibfnamefont {N.}~\bibnamefont {Nanda}}, \bibinfo
  {author} {\bibfnamefont {N.}~\bibnamefont {Joseph}}, \bibinfo {author}
  {\bibfnamefont {N.}~\bibnamefont {DasSarma}}, \bibinfo {author}
  {\bibfnamefont {T.}~\bibnamefont {Henighan}}, \bibinfo {author}
  {\bibfnamefont {B.}~\bibnamefont {Mann}}, \bibinfo {author} {\bibfnamefont
  {A.}~\bibnamefont {Askell}}, \bibinfo {author} {\bibfnamefont
  {Y.}~\bibnamefont {Bai}}, \bibinfo {author} {\bibfnamefont {A.}~\bibnamefont
  {Chen}}, \bibinfo {author} {\bibfnamefont {T.}~\bibnamefont {Conerly}},
  \bibinfo {author} {\bibfnamefont {D.}~\bibnamefont {Drain}}, \bibinfo
  {author} {\bibfnamefont {D.}~\bibnamefont {Ganguli}}, \bibinfo {author}
  {\bibfnamefont {Z.}~\bibnamefont {Hatfield-Dodds}}, \bibinfo {author}
  {\bibfnamefont {D.}~\bibnamefont {Hernandez}}, \bibinfo {author}
  {\bibfnamefont {S.}~\bibnamefont {Johnston}}, \bibinfo {author}
  {\bibfnamefont {A.}~\bibnamefont {Jones}}, \bibinfo {author} {\bibfnamefont
  {J.}~\bibnamefont {Kernion}}, \bibinfo {author} {\bibfnamefont
  {L.}~\bibnamefont {Lovitt}}, \bibinfo {author} {\bibfnamefont
  {K.}~\bibnamefont {Ndousse}}, \bibinfo {author} {\bibfnamefont
  {D.}~\bibnamefont {Amodei}}, \bibinfo {author} {\bibfnamefont
  {T.}~\bibnamefont {Brown}}, \bibinfo {author} {\bibfnamefont
  {J.}~\bibnamefont {Clark}}, \bibinfo {author} {\bibfnamefont
  {J.}~\bibnamefont {Kaplan}}, \bibinfo {author} {\bibfnamefont
  {S.}~\bibnamefont {McCandlish}},\ and\ \bibinfo {author} {\bibfnamefont
  {C.}~\bibnamefont {Olah}},\ }\href
  {https://doi.org/10.48550/arXiv.2209.11895} {\bibinfo {title} {In-context
  learning and induction heads}} (\bibinfo {year} {2022}),\ \Eprint
  {https://arxiv.org/abs/2209.11895} {arXiv:2209.11895 [cs.LG]} \BibitemShut
  {NoStop}%
\bibitem [{\citenamefont {Webb}\ \emph {et~al.}(2021)\citenamefont {Webb},
  \citenamefont {Sinha},\ and\ \citenamefont {Cohen}}]{SI-webb2021emergent}%
  \BibitemOpen
  \bibfield  {author} {\bibinfo {author} {\bibfnamefont {T.~W.}\ \bibnamefont
  {Webb}}, \bibinfo {author} {\bibfnamefont {I.}~\bibnamefont {Sinha}},\ and\
  \bibinfo {author} {\bibfnamefont {J.~D.}\ \bibnamefont {Cohen}},\ }in\
  \href@noop {} {\emph {\bibinfo {booktitle} {International Conference on
  Learning Representations}}}\ (\bibinfo {year} {2021})\BibitemShut {NoStop}%
\bibitem [{\citenamefont {Wang}\ \emph {et~al.}(2023)\citenamefont {Wang},
  \citenamefont {Variengien}, \citenamefont {Conmy}, \citenamefont
  {Shlegeris},\ and\ \citenamefont {Steinhardt}}]{SI-wang2023interpretability}%
  \BibitemOpen
  \bibfield  {author} {\bibinfo {author} {\bibfnamefont {K.~R.}\ \bibnamefont
  {Wang}}, \bibinfo {author} {\bibfnamefont {A.}~\bibnamefont {Variengien}},
  \bibinfo {author} {\bibfnamefont {A.}~\bibnamefont {Conmy}}, \bibinfo
  {author} {\bibfnamefont {B.}~\bibnamefont {Shlegeris}},\ and\ \bibinfo
  {author} {\bibfnamefont {J.}~\bibnamefont {Steinhardt}},\ }in\ \href
  {https://openreview.net/forum?id=NpsVSN6o4ul} {\emph {\bibinfo {booktitle}
  {The Eleventh International Conference on Learning Representations}}}\
  (\bibinfo {year} {2023})\BibitemShut {NoStop}%
\end{thebibliography}%
