# Supplementary material for: Cognitive Maps in Large Language Models
Source: arXiv:2610.25596 source file (2026-11-06)
Supplement: Supplementary file 3 [file 01_transformer_background.tex]

\section{Transformer Architecture and Notation}

Expanding on the discussion in the main text, we begin with a formal account of information flow through an autoregressive transformer \cite{SI-vaswani_2017_transformer} and introduce notation used throughout the Supplementary Information.

\subsection{General organization of a transformer}

A transformer represents and processes text as a sequence of tokens. We denote the one-hot representation of a token at position $t$ by $\mathbf e_t \in \{0,1\}^{N_{\mathrm{vocab}}}$, where $N_{\mathrm{vocab}}$ is the vocabulary size. Tokens are mapped to vectors via an embedding matrix $W_{\mathrm{embed}} \in \R^{D_{\mathrm{model}} \times N_{\mathrm{vocab}}}$.\footnote{All weight matrices denoted by $W$ are learned and are held fixed in our experiments.} Applying this matrix to a sequence of tokens produces an initial sequence of hidden vectors:
\begin{equation}
    \{\mathbf h_{t,1}\}_{t=1}^{N_{\mathrm{tokens}}}
    =
    \{W_{\mathrm{embed}}\mathbf e_t\}_{t=1}^{N_{\mathrm{tokens}}}.
\end{equation}
In general, we use $\mathbf h_{t,l}\in\mathbb R^{D_{\mathrm{model}}}$ to denote the hidden vector at token position $t$ and layer $l$.

Information processing in a transformer occurs by successively updating the sequence of hidden vectors through a stack of layers. Each layer applies two operations in succession.\footnote{For clarity, we omit normalization steps from the equations throughout, although we describe them briefly below.} The first operation is \textit{self-attention}:
\begin{equation}
    \tilde{\mathbf h}_{t,l}
    =
    \mathbf h_{t,l}
    +
    \mathrm{SelfAttention}_l
    \left(\{\mathbf h_{s,l}\}_{s=1}^{N_{\mathrm{tokens}}}\right)_t.
\end{equation}
As we discuss below, self-attention permits the hidden vector at position $t$ to retrieve information from hidden vectors at positions $s \leq t$. The second operation is the \textit{feedforward} operation:
\begin{equation}
    \mathbf h_{t,l+1}
    =
    \tilde{\mathbf h}_{t,l}
    +
    \mathrm{Feedforward}_l(\tilde{\mathbf h}_{t,l}).
\end{equation}
The feedforward operation acts on the hidden vector at each token position independently. As these two operations are repeated across the stack of layers, the resulting hidden vectors $\mathbf h_{t,l}$ become context-dependent representations of the tokens at their corresponding positions $t$.

After the hidden vectors have passed through the final layer, the sequence of vectors is mapped back to the vocabulary via an unembedding matrix $W_{\mathrm{unembed}} \in \mathbb R^{N_{\mathrm{vocab}} \times D_{\mathrm{model}}}$. This produces a sequence of \textit{logit vectors}:
\begin{equation}
    \{\boldsymbol{\ell}_t\}_{t=1}^{N_{\mathrm{tokens}}}
    =
    \left\{
    W_{\mathrm{unembed}}
    \mathbf h_{t,N_{\mathrm{layers}}+1}
    \right\}_{t=1}^{N_{\mathrm{tokens}}}.
\end{equation}
Each logit vector $\boldsymbol{\ell}_t \in \mathbb R^{N_{\mathrm{vocab}}}$ determines the model's predicted distribution over the next token:
\begin{equation}
    p_t(a)
    =
    \frac{\exp(\ell_{t,a})}
    {\sum_{b=1}^{N_{\mathrm{vocab}}}\exp(\ell_{t,b})},
\end{equation}
where $p_t(a)$ is the predicted probability of token $a$ following position $t$. Consequently, differences between logits equal log probability ratios.

\subsection{Self-attention}

We next define the \textit{self-attention} operation. Self-attention operates on a sequence of hidden vectors $\{\mathbf h_t\}_{t=1}^{N_{\mathrm{tokens}}}$ and allows each vector to retrieve information from preceding vectors. Its output is:\footnote{In this subsection and the next, we suppress the layer index $l$; the operations and their associated weight matrices should be understood as belonging to a particular layer.}
\begin{equation}
    \mathrm{SelfAttention}(\{\mathbf h_s\})_t
    =
    \sum_{i = 1}^{N_{\mathrm{heads}}} \sum_{s\le t}
    \underbrace{
        A^{(i)}_{t \leftarrow s}
    }_{\substack{\text{retrieval}\\\text{weights}}}
    \,\cdot\,
    \underbrace{
        W_O^{(i)}W_V^{(i)}\mathbf{h}_s
    }_{\substack{\text{retrieved}\\\text{information}}}.
\end{equation}
As observed in prior work \cite{SI-gershman_2025_key_value_memory}, self-attention can be viewed as a set of parallel \textit{key--value memory systems}, each associated with an ``attention head'' (here indexed by $i = 1, \ldots, N_{\mathrm{heads}}$). The characteristic feature of a key--value memory system is a separation between what information is retrieved and where that information is retrieved from. Here, the product of the two matrices $W_O^{(i)} \in \R^{D_{\mathrm{model}}\times D_{\mathrm{head}}}$ and $W_V^{(i)} \in \R^{D_{\mathrm{head}}\times D_{\mathrm{model}}}$ determines what information can be retrieved from each position.\footnote{$D_{\mathrm{head}}$ is typically chosen so that $N_{\mathrm{heads}}D_{\mathrm{head}}$ is of order $D_{\mathrm{model}}$, so that the product $W_O^{(i)}W_V^{(i)}$ is low-rank.} The source of the retrieved information is determined by the lower-triangular entries of the attention weight matrix $A^{(i)}_{t \leftarrow s}$, which specify, for each position $t$, how strongly each previous position $s$ is accessed.

Each entry of $A^{(i)}_{t \leftarrow s}$ is computed from the hidden vectors $\mathbf h_s$ and $\mathbf h_t$ by applying separate linear transformations to generate a \textit{key} from $\mathbf h_s$ and a \textit{query} from $\mathbf h_t$, taking their dot product, and applying a nonlinearity:
\begin{equation}
    A^{(i)}_{t\leftarrow s}
    =
    \sigma\left(
    \left\langle
    \underbrace{
        W_K^{(i)}\mathbf h_s
    }_{\text{key}},
    \underbrace{
        W_Q^{(i)}\mathbf h_t
    }_{\text{query}}
    \right\rangle
    \right).
\end{equation}
Here, $W_K^{(i)}, W_Q^{(i)} \in \R^{D_{\mathrm{head}}\times D_{\mathrm{model}}}$. Transformers use a scaled softmax for the nonlinearity:
\begin{equation}
    \sigma(z_{ts})
    =
    \frac{
        \exp\!\left(z_{ts}/\xi\right)
    }{
        \sum_{s' \le t}
        \exp\!\left(z_{ts'}/\xi\right)
    },
\end{equation}
where $\xi$ is a scaling factor of order $\sqrt{D_{\mathrm{head}}}$.

Notice that the information retrieved from previous token positions depends on the hidden vectors $\mathbf h_t$ only through the $D_{\mathrm{head}}$-dimensional keys and values:
\begin{equation}
    \mathbf{k}_t^{(i)}
    =
    W_K^{(i)}\mathbf h_t,
    \qquad
    \mathbf{v}_t^{(i)}
    =
    W_V^{(i)}\mathbf h_t.
\end{equation}
In practice, when sampling autoregressively from a transformer, the state retained between successive token-generation steps is the complete collection of keys and values, referred to as the \textit{key--value cache}. In the main text, we call this object the \textit{key--value memory} to emphasize its functional role as the stored information that later tokens can access through attention.

\subsection{Feedforward processing}

For our purposes, only two aspects of the feedforward operation are salient: (1) it acts independently at each token position, and (2) it implements a highly nonlinear transformation containing a large fraction of the model's parameters. For the models we studied here \cite{SI-gemma_2025_gemma3,SI-grattafiori_2024_llama3,SI-yang_2025_qwen3}, the feedforward operation is a gated multilayer perceptron:
\begin{equation}
    \mathrm{Feedforward}(\mathbf h_t)
    =
    W_{\mathrm{down}}
    \left[
        \phi\!\left(W_{\mathrm{gate}}\mathbf h_t\right)
        \odot
        \left(W_{\mathrm{up}}\mathbf h_t\right)
    \right],
\end{equation}
where $W_{\mathrm{gate}},W_{\mathrm{up}}\in\mathbb R^{D_{\mathrm{feedforward}}\times D_{\mathrm{model}}}$ and $W_{\mathrm{down}}\in\mathbb R^{D_{\mathrm{model}}\times D_{\mathrm{feedforward}}}$.\footnote{$D_\mathrm{feedforward}$ is typically chosen to be several times $D_\mathrm{model}$.} Here, $\odot$ denotes element-wise multiplication and $\phi$ is a gating nonlinearity.

\subsection{Architectural variations}

Our description above omits several architectural details of the models we studied \cite{SI-gemma_2025_gemma3,SI-grattafiori_2024_llama3,SI-yang_2025_qwen3}. For completeness, we briefly describe some of these details, though they are not central to the analyses presented in this study.

First, in the models we study, positional information is supplied by \textit{rotary positional embeddings} \cite{SI-su_2024_roformer}, which apply position-dependent rotations to the queries and keys:
\begin{equation}
    \widetilde{\mathbf q}_t^{(i)}
    =
    R_t \mathbf q_t^{(i)},
    \qquad
    \widetilde{\mathbf k}_t^{(i)}
    =
    R_t \mathbf k_t^{(i)}.
\end{equation}
Here, each $R_t \in \R^{D_\mathrm{head} \times D_\mathrm{head}}$ is a block diagonal rotation matrix. Attention weights are then computed from the rotated queries and keys.

Second, the self-attention and feedforward operations are interleaved with normalization steps that rescale the inputs to these operations. In some of the models we study, additional normalization is applied to the outputs of these operations, and/or to the query and key vectors before attention weights are computed. 

Third, the models we study use \textit{grouped-query attention} \cite{SI-ainslie_2023_gqa}. In this architecture, attention heads are divided into groups whose members share the same keys and values but generate distinct queries.

Fourth, some models use \textit{local attention} in some layers, restricting information flow to a fixed window of preceding positions. Because all prompts we use in this study are shorter than this window, this detail does not affect our analyses. 
