# Supplementary material for: Cognitive Maps in Large Language Models
Source: arXiv:2610.25596 source file (2026-11-06)
Supplement: Supplementary file 4 [file 02_mosaic_experiments.tex]

\section{Mosaic Experiments}
\label{SI-sec:mosaic_experiments}

In this section, we describe the basic logic and structure of a mosaic experiment. We begin by re-defining the two objects of study introduced in the main text: the activation tensor $\A$ and the key--value memory $\M$. We then formalize the account of information flow through these two objects developed in the main text by expressing the model's computation as a composition of encoding, projection, and readout operations. We next explain how mosaic experiments allow us to study the organization of information in $\A$ and $\M$. Finally, we describe some advantages of experiments of this form.

\subsection{Gross structure of information flow}

We now give a perspective on the gross structure of information flow through an autoregressive transformer as it processes the prompts used in this study. To develop this perspective, we consider how information flows through the representations generated by the three segments of each prompt: the instructions, the relationship statements, and the query. Each segment generates a distinct subset of the hidden vectors $\mathbf h_{tl}$ and key–value pairs $(\mathbf k_{tl}^{(i)}, \mathbf v_{tl}^{(i)})$, whose dependence on the other segments is constrained by the model’s causal architecture. These constraints allow us to associate each subset with a distinct computational role:
\begin{enumerate}
\item Hidden vectors and key--value pairs generated by the instruction segment (e.g., ``Read the context describing a series of relationships\ldots'') can depend on the instructions themselves, but not on the specific instance of the task introduced later in the prompt. Therefore, their natural computational role is to store information about the task and condition how subsequently presented information is processed.
\item Hidden vectors and key--value pairs generated by the relationship statements (e.g., \texttt{Alice has daughter Beth. Beth has daughter Carol.}) incorporate information about the specific task instance presented in the prompt. Their natural computational role is to carry this instance-specific information forward for use in subsequent computation. As in the main text, we refer to these collections of hidden vectors and key--value pairs as the \textit{activation tensor} and \textit{key--value memory}, respectively, and define them formally below.
\item Hidden vectors generated by the query segment (e.g., \texttt{Question: Who is Carol's grandmother? Answer:}) depend on the query itself and, through the representations described above, on the preceding relationship statements. Their natural computational role is therefore to integrate information from the query with information retrieved from the relational context to compute an answer.
\end{enumerate}

To formalize these ideas, we now write the model's input--output map as the composition of encoding, projection, and readout operations. To begin, as in the main text, we define the activation tensor, $\A$, as the collection of hidden vectors generated by the relationship statements:
\begin{equation}
\A
=
\Big\{
\mathbf{h}_{t, l}
\Big\}
_{\begin{subarray}{l}
t=t_{\mathrm{start}},\ldots,t_{\mathrm{end}} \\
l=1,\ldots,N_{\mathrm{layers}}
\end{subarray}}
\in \R^{T_\mathrm{rel} \times N_\mathrm{layers} \times D_\mathrm{model}},
\end{equation}
and we define the key--value memory, $\M$, as the associated collection of key--value pairs\footnote{Because $D_{\mathrm{head}}$ is typically chosen so that $N_{\mathrm{heads}}D_{\mathrm{head}}$ is of order $D_{\mathrm{model}}$, $\A$ and $\M$ have roughly the same number of scalar entries.}:
\begin{equation}
\M
=
\Big\{
(\mathbf{k}_{t, l}^{(i)},
 \mathbf{v}_{t, l}^{(i)})
\Big\}_{\begin{subarray}{l}
t=t_{\mathrm{start}},\ldots,t_{\mathrm{end}} \\
l=1,\ldots,N_{\mathrm{layers}} \\
i=1,\ldots,N_{\mathrm{KV}}
\end{subarray}}
\in \left( \R^{T_\mathrm{rel} \times N_\mathrm{layers} \times N_\mathrm{KV} \times D_\mathrm{head}} \right)^2.
\end{equation}
As in the main text, $N_{\mathrm{KV}}$ denotes the number of key--value pairs per layer. Here, $t_{\mathrm{start}}$ and $t_{\mathrm{end}}$ denote token positions corresponding to the beginning and end of the relationship statements\footnote{This partitioning requires that within each relational reasoning setting, the token positions of the boundaries between the three prompt segments remain fixed. To ensure this, we required that (1) each entity name tokenized to a single token; (2) shorter relationship expressions were padded with space tokens to match the length of longer expressions.}, respectively, and $T_{\mathrm{rel}} = t_{\mathrm{end}} - t_{\mathrm{start}} + 1$.

The activation tensor and key--value memory serve as intermediate representations in a factorization of the model's computation into encoding, projection, and readout operations. The activation tensor is a function only of the names $\mathcal{N}_A, \mathcal{N}_B, \mathcal{N}_C$ and the relationships $\mathcal{R}_{AB}, \mathcal{R}_{BC}$ described by the context:
\begin{equation}
\begin{aligned}
    \mathbf A
    &= \Phi\!\left(
    \mathcal N_A,\mathcal N_{B},\mathcal N_C,
    \mathcal R_{AB},\mathcal R_{BC}
    \right),\\
    \Phi &:\mathrm{Names}^{3}\times\mathrm{Relations}^{2}
    \longrightarrow
    \mathbb R^{T_{\mathrm{rel}}\times N_{\mathrm{layers}}\times D_{\mathrm{model}}}.
\end{aligned}
\end{equation}
Here, $\Phi$ can be interpreted as an \textit{encoder} that maps the relationship statements to an activation tensor.\footnote{The encoding map is also dependent on the instruction segment, but we suppress this dependence in the notation because the instructions are held fixed across task instances.}

The key--value memory, $\M$, is in turn a function of the activation tensor, $\A$:
\begin{equation}
\begin{aligned}
    \M &= \Pi(\A), \\
    \Pi &: \R^{
    T_{\mathrm{rel}} \times N_{\mathrm{layers}} \times D_{\mathrm{model}}}
    \longrightarrow (\R^{
    T_{\mathrm{rel}} \times N_{\mathrm{layers}} \times N_{\mathrm{KV}} \times D_{\mathrm{head}}}
    )^2, \\
    \A &\mapsto \M
    =
    \Big\{
    (\mathbf{k}_{t, l}^{(i)},
     \mathbf{v}_{t, l}^{(i)})
    \Big\}, \quad
    \mathbf k_{t,l}^{(i)}
    =
    R_t W_K^{(i,l)} \mathbf h_{t,l}, \
    \mathbf v_{t,l}^{(i)}
    =
    W_V^{(i,l)} \mathbf h_{t,l}.
\end{aligned}
\label{SI-eq:kv_projection}
\end{equation}
Here, $\Pi$ can be interpreted as a \textit{projector} that generates a key--value memory from the activation tensor. $\Pi$ acts by applying the projection matrices $W_K^{(i,l)}$ and $W_V^{(i,l)}$ to generate key--value pairs, then applying the rotation matrices $R_t$ to the keys to supply positional information. 

Finally, the models' response is a function of both the query segment and the relationship statements. The dependence on the latter is mediated entirely through $\M$:
\begin{equation}
\begin{aligned}
    \boldsymbol{\ell}_{ans} &= \Psi(\mathcal{Q}, \M), \\
    \Psi &: \mathrm{Queries} \times (\R^{
    T_{\mathrm{rel}} \times N_{\mathrm{layers}} \times N_{\mathrm{KV}} \times D_{\mathrm{head}}}
    )^2 \longrightarrow \R^{N_{\mathrm{vocab}}}.
\end{aligned}
\end{equation}
Here, $\Psi$ can be interpreted as a \textit{readout} operation that uses the key-value memory $\M$ to answer the query $\mathcal{Q}$. 

In summary, the models' computation can be expressed as a composition of three operations: (1) encoding the relationship statements into the activation tensor $\A$; (2) constructing the key--value memory $\M$ from $\A$; and (3) using $\M$ to answer the query. More formally, writing the context as $\mathcal C = (\mathcal N_A,\mathcal N_B,\mathcal N_C,\mathcal R_{AB},\mathcal R_{BC})$ and the query as $\mathcal Q$, the model's input--output map can be written in the form:
\begin{equation}
    F(\mathcal Q,\mathcal C)
    =
    \Psi\left(\mathcal Q,\Pi\left(\Phi(\mathcal C)\right)\right).
\end{equation}

\subsection{Structure of a mosaic experiment}

We now describe the structure of a \textit{mosaic experiment}, the experimental approach used in this study to probe the organization of information in $\A$ and $\M$. The basic logic of these experiments is to construct modified representations from those generated by the model, then use the model to read out information from the modified representations. Our approach builds on similar causal interventions used to study ``binding IDs'' \cite{SI-feng2024entities}. For each experiment, we performed the following three steps:

\begin{enumerate}
\item We first recorded the representations generated by a set of source contexts $\mathcal{C}_1, \mathcal{C}_2, \ldots$. Depending on the experiment, we recorded either activation tensors or key--value memories:
\begin{equation}
\begin{aligned}
    \A_1, \A_2, \ldots &= \Phi(\mathcal{C}_1), \Phi(\mathcal{C}_2), \ldots \\
    \M_1, \M_2, \ldots &= \Pi(\Phi(\mathcal{C}_1)), \Pi(\Phi(\mathcal{C}_2)), \ldots .
\end{aligned}
\end{equation}
In practice, we evaluated $\Phi(\mathcal \cdot)$ by generating a prompt that instantiates each source context, then running a forward pass while recording the inputs to each layer at the relevant token positions. Similarly, we evaluated $\Pi(\Phi(\cdot))$ by running a forward pass, then recording the relevant entries of the key--value cache. 
\item Next, we constructed a ``mosaic representation'' by recombining the recorded source representations:
\begin{equation}
\begin{aligned}
    \Amosaic &= f(\A_1, \A_2, \ldots) \\
    \Mmosaic &= f(\M_1, \M_2, \ldots).
\end{aligned}
\end{equation}
The specific transformation $f(\ldots)$ is chosen to test a hypothesis about how information is organized within $\A$ or $\M$. 
\item Finally, we used the model to answer a query using the modified representation:
\begin{equation}
\begin{aligned}
    \boldsymbol{\ell}_{\mathrm{ans}}' &= \Psi(\mathcal{Q}, \Pi(\Amosaic)) \\
    \boldsymbol{\ell}_{\mathrm{ans}}' &= \Psi(\mathcal{Q}, \Mmosaic).
\end{aligned}
\end{equation}
In practice, we evaluated $\Psi(\cdot,\Pi(\A))$ by running a forward pass on a prompt containing the query, while replacing the inputs to each layer at positions corresponding to the relationship statements with the hidden vectors $\mathbf h_{tl}$ from $\A$. Similarly, we evaluated $\Psi(\cdot,\M)$ by appending $\M$ to the key--value cache for the instruction segment, then running the model on the query using the resulting cache.
\end{enumerate}

\subsection{Advantages of experiments of this form}

We now wish to emphasize three advantages of experiments of this general form. 

First, our approach is causal rather than correlational. Specifically, we directly manipulate the internal representations of the model, then use the model to read out the effect of these manipulations. Because the \textit{model itself} is used as the ``decoder'', the representational features identified by our experiments are task-relevant by construction. In comparison, fitting external encoding or decoding models to predict neural representations from task variables or vice versa can reveal the existence of certain representational features \cite{SI-norman2006beyond,SI-paninski2007statistical}, but does not directly demonstrate the causal relevance of these features for behavior.

Second, our approach is well suited to studying representational features distributed across many model components. In particular, because our manipulations extend across attention heads, token positions, and layers, we can test hypotheses about representational format without first isolating a sparse sub-circuit in the model specific to our task. 

Third, our approach facilitates the study of representational format without the reconstruction of the circuits that produce or use it. Although we use the model both to produce source representations and to read out from mosaic representations, we need not understand how it implements these operations to study the organization of $\A$ and $\M$. In practice, we have found that our approach is well suited to formulating specific hypotheses about representational format, then designing experiments whose outcomes distinguish between those hypotheses.
