# Supplementary material for: Cognitive Maps in Large Language Models
Source: arXiv:2610.25596 source file (2026-11-06)
Supplement: Supplementary file 5 [file 03_methods.tex]

\section{Materials and Methods}

\subsection{General experimental procedures}
We performed each mosaic experiment for every combination of model and relational reasoning setting; the full results are provided in the accompanying data. Each experiment was performed 50 times with randomly sampled entity assignments. Entity names were sampled uniformly without replacement from fixed pools selected according to the prompt template and tokenizer family; the complete lists are distributed with the accompanying code. Where source contexts required distinct control and donor entities, we sampled their names jointly without replacement. On each trial, we recorded the source representations, combined them to construct the mosaic, then read out responses to all queries specified by the task template. The figures show an informative subset of these queries; complete results are provided in the accompanying data. We measured responses by extracting the probabilities (normalized over the full vocabulary) of the task's answer tokens from the model's next-token distribution.

\subsection{Models and prompts}

The models we studied are listed in Table~\ref{SI-tab:model_revisions}. The Hugging Face \texttt{Transformers} library was used to load and run the models in \texttt{PyTorch}. Models were loaded in \texttt{bfloat16} precision. For \texttt{Qwen3} models, thinking mode was disabled.

\begin{table}[htbp]
\centering
\scriptsize
\begin{tabular}{@{}lll@{}}
\hline
Model & Hugging Face repository & Recorded revision \\
\hline
Gemma 3 4B
& \texttt{google/gemma-3-4b-it}
& \texttt{093f9f388b31de276ce2de164bdc2081324b9767} \\
Gemma 3 12B
& \texttt{google/gemma-3-12b-it}
& \texttt{96b6f1eccf38110c56df3a15bffe176da04bfd80} \\
Gemma 3 27B
& \texttt{google/gemma-3-27b-it}
& \texttt{005ad3404e59d6023443cb575daa05336842228a} \\
Llama 3.1 8B Instruct
& \texttt{meta-llama/Llama-3.1-8B-Instruct}
& \texttt{0e9e39f249a16976918f6564b8830bc894c89659} \\
Llama 3.1 70B Instruct
& \texttt{meta-llama/Llama-3.1-70B-Instruct}
& \texttt{1605565b47bb9346c5515c34102e054115b4f98b} \\
Qwen3 0.6B
& \texttt{Qwen/Qwen3-0.6B}
& \texttt{c1899de289a04d12100db370d81485cdf75e47ca} \\
Qwen3 1.7B
& \texttt{Qwen/Qwen3-1.7B}
& \texttt{70d244cc86ccca08cf5af4e1e306ecf908b1ad5e} \\
Qwen3 4B
& \texttt{Qwen/Qwen3-4B}
& \texttt{1cfa9a7208912126459214e8b04321603b3df60c} \\
Qwen3 8B
& \texttt{Qwen/Qwen3-8B}
& \texttt{b968826d9c46dd6066d109eabc6255188de91218} \\
Qwen3 14B
& \texttt{Qwen/Qwen3-14B}
& \texttt{40c069824f4251a91eefaf281ebe4c544efd3e18} \\
Qwen3 32B
& \texttt{Qwen/Qwen3-32B}
& \texttt{9216db5781bf21249d130ec9da846c4624c16137} \\
\hline
\end{tabular}
\caption{Models used in the study.}
\label{SI-tab:model_revisions}
\end{table}

For each relational reasoning setting, we defined a prompt template containing an instruction segment, relationship statements, and a query segment. The complete templates are provided in Section~\ref{SI-sec:prompt_templates}. Concrete prompts were generated by substituting entity names and relationships into slots of fixed token length. To preserve token positions across instances of a given template, we used single-token entity names and padded relationship substitutions with trailing space tokens to fill their allotted slots. Prompts were then formatted using each model's chat template. 

\subsection{Recording and reading out from mosaic representations}

To record a source activation tensor $\A = \Phi(\mathcal C)$, we generated a prompt instantiating $\mathcal C$ and ran a forward pass, using \texttt{PyTorch} forward pre-hooks to record the inputs to each transformer decoder block at positions corresponding to the relationship statements. The recorded span extended from the first entity name through the punctuation terminating the final relationship statement. We stacked these inputs along the layer axis to form $\A$. Similarly, to record a source key--value memory $\M = \Pi(\Phi(\mathcal C))$, we recorded and assembled the key--value cache entries over the same token span.

To read out from an activation tensor $\A$, we evaluated $\Psi(\mathcal Q,\Pi(\A))$ using a prompt containing the instruction segment, dummy relationship statements, and the query $\mathcal Q$. During the forward pass, we used \texttt{PyTorch} forward pre-hooks to replace the inputs to each transformer decoder block within the relationship span with the hidden vectors from $\A$, leaving inputs at other positions unmodified.\footnote{An equivalent implementation would explicitly construct $\M = \Pi(\A)$, then read out from the resulting key--value memory.} To read out from a key--value memory $\M$, we initialized a key--value cache using the prompt prefix preceding the relationship statements and appended $\M$. We then generated the query segment corresponding to $\mathcal Q$ and ran the model on this segment using the resulting cache.

\subsection{Construction of mosaics}

Here, we give the exact mosaic constructions used to generate each figure. Because the mosaic experiments defined by the constructions below can be performed for any model and/or prompt template, we give the constructions using the mathematical language developed in Section \ref{SI-sec:mosaic_experiments}. We will write $\A_t$ for the slice of the activation tensor corresponding to token position $t$ (each $\A_t \in \R^{N_\mathrm{layers} \times D_\mathrm{model}}$), and $\mathbf K_{tli}$ and $\mathbf V_{tli}$ for the key and value vector, respectively, at position $t$, layer $l$, and key--value head $i$ (each $\mathbf K_{tli}, \mathbf V_{tli} \in \R^{D_\mathrm{head}}$). Token positions are identified by their slots in the prompt template: for example, $t_{\text{‹B1›}}$ and $t_{\text{‹B2›}}$ denote the first and second occurrences of entity $B$.


\subsubsection{Figure \figref{fig:behavior}.}

For the behavioral measurements in Fig.~\figref{fig:behavior}, we ran ordinary forward passes without recording or modifying internal representations. This is equivalent to reading out from an unmodified activation tensor:
\begin{align}
    &\A = \Phi(\mathcal{N}_A, \mathcal{N}_B, \mathcal{N}_C,
               \mathcal{R}_{AB}, \mathcal{R}_{BC}), \\
    &\Amosaic = \A.
\end{align}


\subsubsection{Figure \figref{fig:separability}.}

We recorded activation tensors from two source contexts:
\begin{equation}
\begin{aligned}
    \Actrl &= \Phi(\mathcal{N}_A, \mathcal{N}_B, \mathcal{N}_C, \mathcal{R}_{AB}, \mathcal{R}_{BC}) \\
    \Adonor &= \Phi(\mathcal{N}_D, \mathcal{N}_E, \mathcal{N}_F, \mathcal{R}_{AB}, \mathcal{R}_{BC}).
\end{aligned}
\end{equation}
The names $\mathcal{N}_A, \mathcal{N}_B, \mathcal{N}_C, \mathcal{N}_D, \mathcal{N}_E, \mathcal{N}_F$ were sampled without replacement. For the mosaic shown in Fig.~\figref{fig:separability}, the replacement was done at the token position corresponding to the first occurrence of the second entity:
\begin{equation}
    (\Amosaic)_t = 
    \begin{cases}
        (\Adonor)_t, & t = t_\text{‹B1›} \\
        (\Actrl)_t, & \text{otherwise}
    \end{cases}.
\end{equation}
Results for analogous substitutions at other entity positions are included in the accompanying data.


\subsubsection{Figure \figref{fig:additivity}.}

We recorded activation tensors from three source contexts:
\begin{equation}
\begin{aligned}
    \Actrl &= \Phi(\mathcal{N}_A, \mathcal{N}_B, \mathcal{N}_C,
                   \mathcal{R}_{AB}, \mathcal{R}_{BC}) \\
    \Adonor^{(1)} &= \Phi(\mathcal{N}_D, \mathcal{N}_E, \mathcal{N}_F,
                          \mathcal{R}_{AB}, \mathcal{R}_{BC}) \\
    \Adonor^{(2)} &= \Phi(\mathcal{N}_F, \mathcal{N}_E, \mathcal{N}_D,
                          \mathcal{R}_{AB}, \mathcal{R}_{BC}).
\end{aligned}
\end{equation}
The names $\mathcal{N}_A, \mathcal{N}_B, \mathcal{N}_C, \mathcal{N}_D, \mathcal{N}_E, \mathcal{N}_F$ were sampled without replacement. We constructed a difference tensor by subtracting the slice corresponding to $\mathcal{N}_D$ in the first position from the slice corresponding to the same name in the final position:
\begin{equation}
    \boldsymbol{\delta}
    = (\Adonor^{(2)})_{t_\text{‹C1›}}
    - (\Adonor^{(1)})_{t_\text{‹A1›}}.
\end{equation}
We then added and subtracted $\boldsymbol{\delta}$ to and from different slices of the control tensor to generate the mosaic:
\begin{equation}
    (\Amosaic)_t =
    \begin{cases}
        (\Actrl)_t + \boldsymbol{\delta}, & t = t_\text{‹A1›} \\
        (\Actrl)_t - \boldsymbol{\delta}, & t = t_\text{‹C1›} \\
        (\Actrl)_t, & \text{otherwise}
    \end{cases}.
\label{SI-eq:additivity_mosaic}
\end{equation}


\subsubsection{Figure \figref{fig:composition}.}

We recorded activation tensors from two source contexts that differed in the first relationship:
\begin{equation}
\begin{aligned}
    \Actrl &= \Phi(\mathcal{N}_A, \mathcal{N}_B, \mathcal{N}_C,
                   \mathcal{R}_{AB}, \mathcal{R}_{BC}) \\
    \Adonor &= \Phi(\mathcal{N}_A, \mathcal{N}_B, \mathcal{N}_C,
                    \mathcal{R}_{AB}^{-1}, \mathcal{R}_{BC}),
\end{aligned}
\label{SI-eq:prospective_retrospective_1}
\end{equation}
where $\mathcal{R}_{AB}^{-1}$ denotes the inverse relationship of $\mathcal{R}_{AB}$. To generate the mosaic, we replaced control slices corresponding to the second relationship phrase and the final entity with the corresponding donor slices:\footnote{Here and elsewhere, the causal structure of the activation tensor determines what should be replaced to build $\mathbf{A}_{\mathrm{mosaic}}$. In this case, because we are asking about the structure of the name-independent component of $\mathbf{A}$, the ``edge'' or ``location'' corresponding to the last entity could appear as soon as the relation token preceding that entity.}
\begin{equation}
    (\Amosaic)_t =
    \begin{cases}
        (\Adonor)_t, & t = t_\text{‹R-BC›}, \ldots, t_\text{‹C1›} \\
        (\Actrl)_t, & \text{otherwise}
    \end{cases}.
\label{SI-eq:prospective_retrospective_2}
\end{equation}
Here, $t_\text{‹R-BC›}$ denotes the first token of the second relationship phrase.


\subsubsection{Figure \figref{fig:binding}.}

We constructed key--value mosaics by replacing vectors in a control memory with corresponding vectors from an ``average memory''. The average memory was computed over $N_{\mathrm{trials}} = 100$ separately sampled entity assignments, with the relationships held fixed. Formally, we evaluated:
\begin{equation}
    \bigl(
        \mathbf K_{\mathrm{average}},
        \mathbf V_{\mathrm{average}}
    \bigr)
    =
    \frac{1}{N_{\mathrm{trials}}}
    \sum_{n=1}^{N_{\mathrm{trials}}}
    \Pi\left(
        \Phi\left(
            \mathcal{N}_A^{(n)},
            \mathcal{N}_B^{(n)},
            \mathcal{N}_C^{(n)},
            \mathcal{R}_{AB},
            \mathcal{R}_{BC}
        \right)
    \right).
\end{equation}

\medskip
\noindent\textit{Keys-first and values-first mosaics.} This experiment was partially inspired by \cite{SI-jarvik1973genetic}. We recorded key-value memories from one source context:
\begin{equation}
    (\mathbf K_\mathrm{control}, \mathbf V_\mathrm{control})
    = \Pi\bigl(\Phi(\mathcal{N}_A, \mathcal{N}_B, \mathcal{N}_C,
                     \mathcal{R}_{AB}, \mathcal{R}_{BC})\bigr).
\end{equation}
We generated the mosaic by replacing selected key and value vectors in the control memory with the corresponding vectors from the average memory. We took $L_{\mathrm{split}} =
\lfloor N_{\mathrm{layers}}/2 \rfloor$ for all models except Qwen,
for which we used $L_{\mathrm{split}} =
\lfloor 2N_{\mathrm{layers}}/3 \rfloor$.\footnote{For Qwen models, placing the split halfway through the model did not preserve performance; we instead placed the split two-thirds of the way through the model. Retrieval in Qwen models may therefore require certain name-to-symbol pairs beyond the model's midpoint.}
For the keys-first mosaic, we replaced values at layers
$l \leq L_{\mathrm{split}}$ and keys at layers
$l > L_{\mathrm{split}}$:
\begin{equation}
\begin{aligned}
    (\mathbf K_{\text{keys-first}})_{tli}
    &=
    \begin{cases}
        (\mathbf K_{\text{control}})_{tli},
            & l \leq L_{\mathrm{split}} \\
        (\mathbf K_{\text{average}})_{tli},
            & l > L_{\mathrm{split}}
    \end{cases},
    &
    (\mathbf V_{\text{keys-first}})_{tli}
    &=
    \begin{cases}
        (\mathbf V_{\text{average}})_{tli},
            & l \leq L_{\mathrm{split}} \\
        (\mathbf V_{\text{control}})_{tli},
            & l > L_{\mathrm{split}}
    \end{cases}.
\end{aligned}
\end{equation}
For the values-first mosaic, we reversed this assignment:
\begin{equation}
\begin{aligned}
    (\mathbf K_{\text{values-first}})_{tli}
    &=
    \begin{cases}
        (\mathbf K_{\text{average}})_{tli},
            & l \leq L_{\mathrm{split}} \\
        (\mathbf K_{\text{control}})_{tli},
            & l > L_{\mathrm{split}}
    \end{cases},
    &
    (\mathbf V_{\text{values-first}})_{tli}
    &=
    \begin{cases}
        (\mathbf V_{\text{control}})_{tli},
            & l \leq L_{\mathrm{split}} \\
        (\mathbf V_{\text{average}})_{tli},
            & l > L_{\mathrm{split}}
    \end{cases}.
\end{aligned}
\end{equation}

\medskip
\noindent\textit{Sparse mosaics.}
We retained control keys and values at selected sites and replaced all other vectors with their averages. The pruning procedure used to isolate these sites is described in Section~\ref{SI-sec:pruning_trajectories}. We denote the sets of sites at which keys and values were retained by the iterative pruning procedure by $K_{\mathrm{rem}}$ and $V_{\mathrm{rem}}$, respectively.
\begin{equation}
\begin{aligned}
    (\mathbf K_{\text{sparse}})_{tli}
    &=
    \begin{cases}
        (\mathbf K_{\text{control}})_{tli},
            & (t,l,i) \in K_{\mathrm{rem}} \\
        (\mathbf K_{\text{average}})_{tli},
            & \text{otherwise}
    \end{cases},
    &
    (\mathbf V_{\text{sparse}})_{tli}
    &=
    \begin{cases}
        (\mathbf V_{\text{control}})_{tli},
            & (t,l,i) \in V_{\mathrm{rem}} \\
        (\mathbf V_{\text{average}})_{tli},
            & \text{otherwise}
    \end{cases}.
\end{aligned}
\end{equation}

\medskip
\noindent\textit{Edited mosaics.}
We recorded control and donor memories from two source contexts:
\begin{equation}
\begin{aligned}
    (\mathbf K_\mathrm{control}, \mathbf V_\mathrm{control})
    &= \Pi\bigl(\Phi(\mathcal{N}_A, \mathcal{N}_B, \mathcal{N}_C,
                     \mathcal{R}_{AB}, \mathcal{R}_{BC})\bigr) \\
    (\mathbf K_\mathrm{donor}, \mathbf V_\mathrm{donor})
    &= \Pi\bigl(\Phi(\mathcal{N}_D, \mathcal{N}_E, \mathcal{N}_F,
                     \mathcal{R}_{AB}, \mathcal{R}_{BC})\bigr).
\end{aligned}
\end{equation}
The names $\mathcal{N}_A, \mathcal{N}_B, \mathcal{N}_C ,\mathcal{N}_D, \mathcal{N}_E, \mathcal{N}_F$ were sampled without replacement. To edit the values
associated with the first entity, we replaced control values at sites in $V_{\mathrm{rem}}$ at position $t_{\text{‹A1›}}$ with the corresponding donor values. All keys and all other values were retained from the control memory:
\begin{equation}
\begin{aligned}
    (\mathbf K_{\text{edited}})_{tli}
    &= (\mathbf K_{\text{control}})_{tli}, \\
    (\mathbf V_{\text{edited}})_{tli}
    &=
    \begin{cases}
        (\mathbf V_{\text{donor}})_{tli},
            & (t,l,i) \in V_{\mathrm{rem}}
              \text{ and } t = t_{\text{‹A1›}} \\
        (\mathbf V_{\text{control}})_{tli},
            & \text{otherwise}
    \end{cases}.
\end{aligned}
\end{equation}
Other edits were defined similarly.


\subsubsection{Figure \ref{SI-fig:S1_rope_swap}.}

We recorded an activation tensor from a single source context:
\begin{equation}
    \Actrl = \Phi(\mathcal{N}_A, \mathcal{N}_B, \mathcal{N}_C,
                  \mathcal{R}_{AB}, \mathcal{R}_{BC}).
\end{equation}
We constructed the mosaic by exchanging the slices at the first occurrences of the first and second entities, leaving all other slices unchanged:
\begin{equation}
    (\Amosaic)_t =
    \begin{cases}
        (\Actrl)_{t_\text{‹B1›}}, & t = t_\text{‹A1›} \\
        (\Actrl)_{t_\text{‹A1›}}, & t = t_\text{‹B1›} \\
        (\Actrl)_t, & \text{otherwise}
    \end{cases}.
\label{SI-eq:position_swap_mosaic}
\end{equation}
During readout, $\Pi$ applies the rotation matrices associated with the destination positions, so each exchanged slice receives the positional information associated with the other's original position.


\subsubsection{Figure \ref{SI-fig:S2_indirect_swap}.}

We recorded activation tensors from three prompts containing the same entity names and relationships but differing in the number of space tokens inserted immediately before the relationship statements. We defined $\Delta = t_\text{‹B1›} - t_\text{‹A1›}$ and inserted $0$, $\Delta$, or $2\Delta$ space tokens. Writing $\Phi_{+s}$ for recording with $s$ inserted tokens, we obtained:
\begin{equation}
\begin{aligned}
    \A_{-\Delta}
    &= \Phi(\mathcal{N}_A, \mathcal{N}_B, \mathcal{N}_C,
             \mathcal{R}_{AB}, \mathcal{R}_{BC}) \\
    \Actrl
    &= \Phi_{+\Delta}(\mathcal{N}_A, \mathcal{N}_B, \mathcal{N}_C,
                      \mathcal{R}_{AB}, \mathcal{R}_{BC}) \\
    \A_{+\Delta}
    &= \Phi_{+2\Delta}(\mathcal{N}_A, \mathcal{N}_B, \mathcal{N}_C,
                       \mathcal{R}_{AB}, \mathcal{R}_{BC}).
\end{aligned}
\end{equation}
The subscripts $-\Delta$ and $+\Delta$ denote shifts relative to the control prompt. In the equations below, token indices identify positions within the relationship span, so a given index refers to the same template slot across the three tensors.

We replaced the control slice at ‹A1› with the corresponding slice from $\A_{+\Delta}$, and the control slice at ‹B1› with the corresponding slice from $\A_{-\Delta}$:
\begin{equation}
    (\Amosaic)_t =
    \begin{cases}
        (\A_{+\Delta})_{t_\text{‹A1›}}, & t = t_\text{‹A1›} \\
        (\A_{-\Delta})_{t_\text{‹B1›}}, & t = t_\text{‹B1›} \\
        (\Actrl)_t, & \text{otherwise}
    \end{cases}.
\label{SI-eq:global_position_swap_mosaic}
\end{equation}
With this choice of $\Delta$, the donor slice inserted at ‹A1› was recorded at the absolute token position occupied by ‹B1› in the control prompt, and vice versa. We read out from the mosaic using the control prompt's padding:
\begin{equation}
    \boldsymbol{\ell}_{\mathrm{ans}}'
    = \Psi_{+\Delta}(\mathcal{Q}, \Pi_{+\Delta}(\Amosaic)).
\end{equation}
