# Supplementary material for: Cognitive Maps in Large Language Models
Source: arXiv:2610.25596 source file (2026-11-06)
Supplement: Supplementary file 6 [file 04_positional_controls.tex]

\section{Tests of Position-Code Hypotheses}

In this section, we present the results of two mosaic experiments designed to test whether the putative representation of abstract relational structure in the activation tensor instead corresponds to a sequence of positional codes. Specifically, we considered the hypothesis that the activation tensor associates information about token identity with positional codes,
\begin{equation}
\begin{aligned}
\ldots,\ \mathcal{P}_{128},\ \mathcal{P}_{129} &,
\mathcal{P}_{130},\ \mathcal{P}_{131},\ \ldots
\\
\ldots,
(\mathcal{P}_{128} \leftrightarrow \text{Alice}),
(\mathcal{P}_{129} \leftrightarrow \text{has}) &,
(\mathcal{P}_{130} \leftrightarrow \text{daughter}),
(\mathcal{P}_{131} \leftrightarrow \text{Beth}),\ \ldots,
\end{aligned}
\end{equation}
and that the model uses these associations to answer queries. Note that under this account, the task-relevant information retained after context presentation is nothing more than the ordered sequence of tokens in the prompt; the interpretation of that sequence as a set of relationships is deferred until a query is presented.

In principle, positional information could either be supplied by the rotary positional embeddings applied when constructing $\M$ from $\A$ or could already be present in $\A$ as learned codes for global token position. We designed one mosaic experiment to test each possibility.

In the first experiment, we exchanged the slices of the activation tensor corresponding to the first occurrences of the first and second entities (Eq.~\ref{SI-eq:position_swap_mosaic}). Recall that when constructing the key--value memory, $\Pi$ applies position-dependent rotations determined by each slice's position (Eq.~\ref{SI-eq:kv_projection}). Therefore, this manipulation exchanges the externally supplied positional information associated with the two entity representations. If the model reconstructs relationships at query time using this positional information, this manipulation should cause it to behave as if the relationship between the first two entities had been reversed. Instead, the models' responses were largely unchanged (Fig.~\ref{SI-fig:S1_rope_swap}).

\begin{figure*}[h]
    \centering
    \fourpaneltable
        {\includegraphics[width=0.24\textwidth]{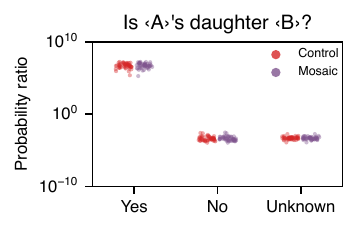}}
        {\includegraphics[width=0.24\textwidth]{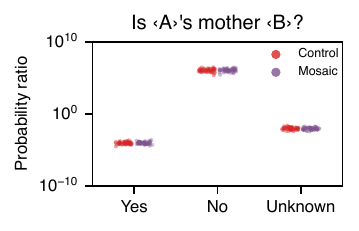}}
        {\includegraphics[width=0.24\textwidth]{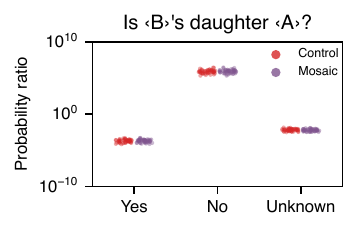}}
        {\includegraphics[width=0.24\textwidth]{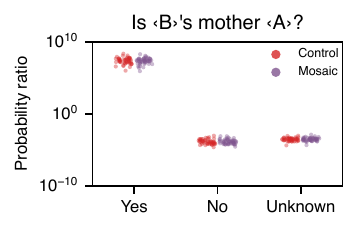}}
    \caption{Exchanging externally supplied positional information does not appreciably change model responses. Results are shown for Gemma-3-27B. 
    \textbf{A--D}, Responses to the queries indicated above each plot
    for control (red) and mosaic (purple) activation tensors.
    Probability ratios are defined as in the main text.
    Fifty trials are shown per condition.}
    \label{SI-fig:S1_rope_swap}
\end{figure*}

This result may initially seem surprising: the manipulation appears to exchange the order of two tokens without appreciably changing the model’s responses. However, note that we exchange rows of $\A$ \textit{after} the model has processed the context. Therefore, if during context processing the model assigns patterns of activity to the relevant entity tokens that track either their role or their original token position, those patterns of activity would travel with the corresponding rows and remain associated with the same entity names.

Those activity patterns could still reflect learned codes for global token positions. We therefore designed a second experiment to exchange these codes, if present, between the two entity representations by changing the token positions at which entity representations were computed. Specifically, we inserted space tokens before the relationship statements to record representations of entities at different absolute token positions. Table~\ref{SI-tab:prompt_offsets} gives an example of three prompts used to record source activation tensors on a particular trial. The middle ($+\Delta$) prompt was used to record $\Actrl$; this allowed us to obtain ``Alice'' and ``Beth'' representations from prompts where the names occurred \textit{later} and \textit{earlier}, respectively, than in the control prompt.

The offsets were chosen so that ``Alice'' in the $+2\Delta$ prompt occurs at ``Beth'''s position in the control prompt, and ``Beth'' in the $+0$ prompt occurs at ``Alice'''s position in the control prompt. We constructed $\Amosaic$ by replacing the row corresponding to ``Alice'' in $\Actrl$ with the corresponding row from the $+2\Delta$ prompt, and the row corresponding to ``Beth'' with the corresponding row from the $+0$ prompt (Eq.~\eqref{SI-eq:global_position_swap_mosaic}). In the example shown in Table~\ref{SI-tab:prompt_offsets}, the ``Alice'' representation in $\Amosaic$ should carry the 134th positional embedding, and the ``Beth'' representation should carry the 131st positional embedding. In general, this manipulation should exchange any learned positional codes associated with the two entities while preserving information about their identities and roles. Under the hypothesis that the model reconstructs relationships from the token–position associations at query time, it should recover the reversed first relationship, ``Beth has daughter Alice''. Instead, the model’s responses were largely unchanged (Fig.~\ref{SI-fig:S2_indirect_swap}).

\begin{table}[ht]
\centering
\scriptsize
\begin{tabular}{@{}r@{\hspace{1.5em}}l@{\hspace{2.5em}}l@{\hspace{2.5em}}l@{}}
\hline
Token index & $+0$ prompt & $+\Delta$ prompt & $+2\Delta$ prompt \\
\hline
$\vdots$ & $\vdots$ & $\vdots$ & $\vdots$ \\
126 & \texttt{Context} & \texttt{Context} & \texttt{Context} \\
127 & \texttt{:} & \texttt{:} & \texttt{:} \\
128 & \texttt{\textvisiblespace Alice} & \texttt{\textvisiblespace} & \texttt{\textvisiblespace} \\
129 & \texttt{\textvisiblespace has} & \texttt{\textvisiblespace} & \texttt{\textvisiblespace} \\
130 & \texttt{\textvisiblespace daughter} & \texttt{\textvisiblespace} & \texttt{\textvisiblespace} \\
131 & \texttt{\textvisiblespace Beth} & \texttt{\textvisiblespace Alice} & \texttt{\textvisiblespace} \\
132 & \texttt{.} & \texttt{\textvisiblespace has} & \texttt{\textvisiblespace} \\
133 & \texttt{\textvisiblespace Beth} & \texttt{\textvisiblespace daughter} & \texttt{\textvisiblespace} \\
134 & \texttt{\textvisiblespace has} & \texttt{\textvisiblespace Beth} & \texttt{\textvisiblespace Alice} \\
135 & \texttt{\textvisiblespace daughter} & \texttt{.} & \texttt{\textvisiblespace has} \\
136 & \texttt{\textvisiblespace Carol} & \texttt{\textvisiblespace Beth} & \texttt{\textvisiblespace daughter} \\
137 & \texttt{.} & \texttt{\textvisiblespace has} & \texttt{\textvisiblespace Beth} \\
138 & \texttt{\textbackslash n\textbackslash n} & \texttt{\textvisiblespace daughter} & \texttt{.} \\
$\vdots$ & $\vdots$ & $\vdots$ & $\vdots$ \\
\hline
\end{tabular}
\caption{Example of prompts used to construct the global-position control. The three prompts contain identical relationship statements, preceded by $0$, $\Delta$, or $2\Delta$ inserted space tokens, where $\Delta$ is the token distance between the first and second entities. The $+\Delta$ prompt serves as the control; the other two supply representations of ``Alice'' and ``Beth'' recorded at the other's absolute positions in the control prompt. The symbol \texttt{\textvisiblespace} denotes a space.}
\label{SI-tab:prompt_offsets}
\end{table}

\begin{figure*}[h]
    \centering
    \fourpaneltable
        {\includegraphics[width=0.24\textwidth]{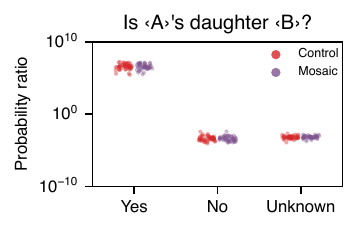}}
        {\includegraphics[width=0.24\textwidth]{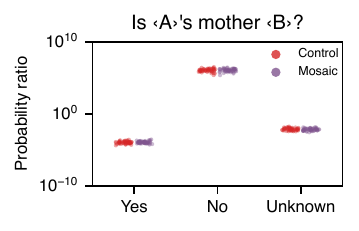}}
        {\includegraphics[width=0.24\textwidth]{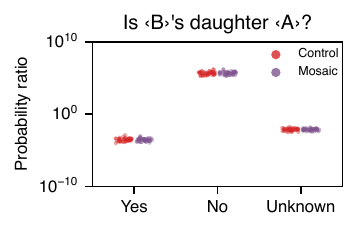}}
        {\includegraphics[width=0.24\textwidth]{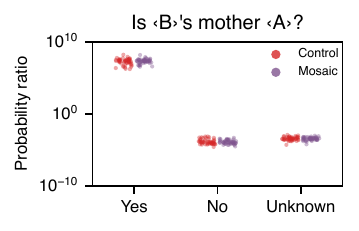}}
    \caption{Exchanging any global positional codes carried by the activation tensor does not appreciably change model responses.
    Results are shown for Gemma-3-27B. 
    \textbf{A--D}, Responses to the queries indicated above each plot
    for control (red) and mosaic (purple) activation tensors.
    Probability ratios are defined as in the main text.
    Fifty trials are shown per condition.}
    \label{SI-fig:S2_indirect_swap}
\end{figure*}
