# Supplementary material for: Cognitive Maps in Large Language Models
Source: arXiv:2610.25596 source file (2026-11-06)
Supplement: Supplementary file 7 [file 05_prospective_retrospective_more.tex]

\section{Evidence for Prospective Composition of Relationships}
\label{SI-sec:prospective_composition}

Recall that in the main text, we presented two hypotheses for the form of the representation of abstract relational structure in the activation tensor:
\begin{enumerate}
    \item \textit{Graph-based representation.} Observed relationships are represented as ``edges'' in $\A$, then composed retrospectively when a query is asked.
    \item \textit{Location-based representation.} As relationships are encountered, models compose them prospectively to assign each entity a ``location'' in a shared coordinate system.
\end{enumerate}
Recall further that the mosaic experiment presented in Fig.~\figref{fig:composition} and eqs. (\ref{SI-eq:prospective_retrospective_1}), (\ref{SI-eq:prospective_retrospective_2}) was designed to distinguish between these two hypotheses. As we argued in the main text, the former hypothesis predicts that $\Amosaic$ supports the same responses to two-step queries as $\Actrl$; the latter predicts that it supports the same responses as $\Adonor$. We found that responses typically matched those obtained from the control tensor (Fig.~\figref{fig:composition}).

Here, we present an exception to this tendency. Figure~\ref{SI-fig:S3_prospective_retrospective_exceptions} shows the models’ responses to four queries given a mosaic activation tensor constructed using the same procedure as in Fig.~\figref{fig:composition}B, but with the donor and control contexts exchanged. An additional exception, obtained with Llama-3.1-70B using the original donor and control assignment, is shown in Fig.~\figref{SI-fig:model-generalization-retrospective-prospective-llama-70b}D.

\begin{figure*}[h]
    \centering
    \fourpaneltable
        {\includegraphics[width=0.24\textwidth]{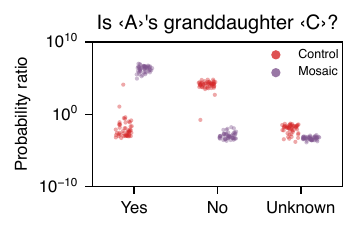}}
        {\includegraphics[width=0.24\textwidth]{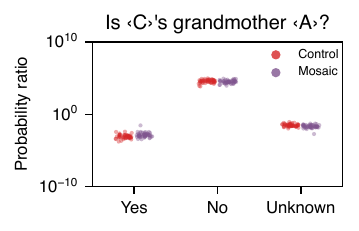}}
        {\includegraphics[width=0.24\textwidth]{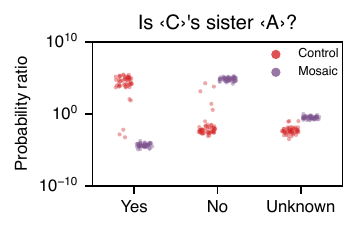}}
        {\includegraphics[width=0.24\textwidth]{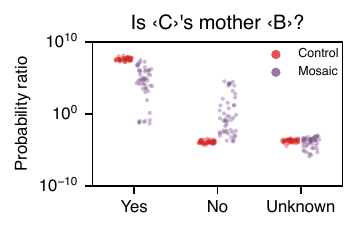}}
    \caption{Evidence for a location-based representation in the family-tree setting.
    In all four panels, the donor context was
    ``$\langle$A$\rangle$ has daughter $\langle$B$\rangle$.
    $\langle$B$\rangle$ has daughter $\langle$C$\rangle$'',
    the control context was
    ``$\langle$A$\rangle$ has mother $\langle$B$\rangle$.
    $\langle$B$\rangle$ has daughter $\langle$C$\rangle$'', and 
    the mosaic was constructed as in main-text Fig.~\figref{fig:composition}. Results are shown for Gemma-3-27B.
    \textbf{A--D}, Responses to the queries indicated above each plot
    for control (red) and mosaic (purple) activation tensors.
    Probability ratios are defined as in the main text.
    Fifty trials are shown per condition.}
    \label{SI-fig:S3_prospective_retrospective_exceptions}
\end{figure*}

In panels S3A and S3C above, the model's responses follow the two-hop relationship implied by the \textit{donor}, rather than the \textit{control} context. The entries of $\Adonor$ that were transferred into $\Actrl$ to construct $\Amosaic$ (i.e., the rows of $\Adonor$ corresponding to the ``has daughter'' and ``Carol'' tokens) must therefore supply some information beyond the relationship between Beth and Carol that is responsible for this change in behavior.

One possibility is that the transferred entries carry a copy
of the ``edge'' between Alice and Beth. The results in panels S3A and S3C could then be explained if the model sometimes uses this copy---which in $\Amosaic$ encodes the relationship between Alice and Beth in the \textit{donor} context---when retrospectively composing relationships. However, this account does not readily explain the disrupted response to the one-hop relationship shared by the control and donor contexts (Fig.~S3D).

A second possibility is that the transferred entries carry information reflecting the prospective composition of the two relationships in the donor context (i.e., the transferred entries carry the information ``Carol is Alice's granddaughter''). Such a ``location-based'' account naturally explains the observation in Fig.~S3D: the location assigned to Carol in the donor context, combined with the location assigned to Beth in the control context, would no longer encode the relationship ``Beth is Carol's mother''.

Notably, when provided with the \textit{same mosaic tensor}, the model's responses to other queries follow the two-hop relationship implied by the \textit{control} context (Fig.~S3B), as predicted by the graph-based hypothesis. Therefore, both location-based information (reflecting prospective composition of relationships) and graph-based information (requiring retrospective composition of relationships) may be available in the activation tensor. We do not yet understand what factors cause the model to rely on one type of information or the other at query time. 

Consistent with this possibility, direct visualizations of $\A$ suggest that activity within some entries of $\A$ depends primarily on the most recent relationship, whereas activity at others depends on the full history of relationships. At each token position, the sequence of hidden vectors in $\A$ across successive layers traces a trajectory through activity space $\mathbb{R}^{D_\mathrm{model}}$. We visualized these trajectories by projecting them onto the first two principal components computed from hidden vectors collected across prompts at the model’s midpoint. We found that at the second relationship token (e.g., ``daughter''), the trajectories depend on both relationships in the context (Fig. S4A). In contrast, at the final entity token (e.g., ``Carol''), they appear to depend primarily on the most recently encountered relationship (Fig. S4B). This contrast is suggestive of the coexistence of graph-based and location-based information in the activation tensor.

\begin{figure*}[h]
    \centering
    \begin{minipage}[c]{0.28\textwidth}
        \centering
        \makebox[\linewidth][l]{\textbf{A}}\par\vspace{3pt}
        \includegraphics[width=\linewidth]{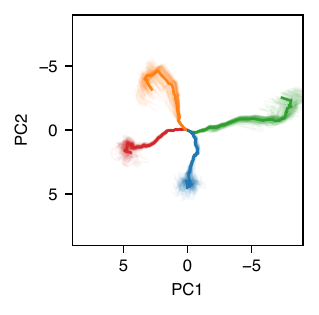}
    \end{minipage}\hspace{25pt}
    \begin{minipage}[c]{0.28\textwidth}
        \centering
        \makebox[\linewidth][l]{\textbf{B}}\par\vspace{3pt}
        \includegraphics[width=\linewidth]{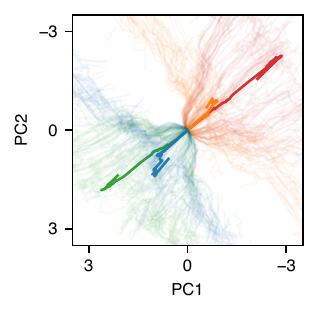}
    \end{minipage}\hfill
    \begin{minipage}[c]{0.38\textwidth}
        \centering
        \includegraphics[width=\linewidth]{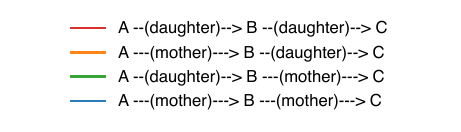}
    \end{minipage}
    \caption{PCA visualizations of activation trajectories in the family-tree setting.
    Each trajectory follows the hidden vector at a fixed token position across successive layers.
    Trajectories were centered by subtracting the layer-wise mean across
    relational structures and name resamplings, then projected
    onto the first two principal components computed from population
    activity halfway through the model.
    Faint lines show individual trajectories; solid lines
    show averages over prompts with the same relational structure but
    different entity names.
    Visualizations are shown for Llama-3.1-70B; the corresponding Gemma-3-27B
    projections were harder to interpret, possibly because the activation
    norm grew more rapidly across layers.
    \textbf{A}, Activations at the second relationship token.
    \textbf{B}, Activations at the final entity token.
}
    \label{SI-fig:family_tree_pca}
\end{figure*}

The exceptions that we describe here are easiest to find in the family-tree setting. We also observed occasional shifts from control-like toward donor-like responses in some transitive inference settings (not shown). However, these cases are harder to interpret because the models do not reliably answer ``Unknown'' when asked about a relationship that the control context leaves undetermined---for example, whether Alice is taller than Carol given ``Alice is taller than Beth; Beth is shorter than Carol''.
