# Supplementary material for: Cognitive Maps in Large Language Models
Source: arXiv:2610.25596 source file (2026-11-06)
Supplement: Supplementary file 8 [file 06_pruning_trajectories.tex]

\section{Identifying Name-to-Symbol and Symbol-to-Name Pairs}
\label{SI-sec:pruning_trajectories}

In this section, we describe the iterative pruning procedure used to find candidate name-to-symbol and symbol-to-name key--value pairs. Briefly, we iteratively ``erased'' name-dependent information from keys and values by replacing them with their averages across prompts with resampled names. At each iteration, we used the gradient of a scalar measure of task performance to estimate the keys or values whose erasure would least affect the models' behavior.

We represented the retained vectors using two binary masks, $m^{(K)}, m^{(V)} \in \{0, 1\}^{T_\mathrm{rel} \times N_\mathrm{layers} \times N_\mathrm{KV}}$. To facilitate differentiation with respect to the mask entries, we expressed the replacement rule as a linear interpolation between control and average key--value memories, treating the mask entries as continuous variables:

\begin{equation}
\begin{aligned}
    (\mathbf K_{\mathrm{interp}})_{tli}
    &=
    (\mathbf K_{\mathrm{average}})_{tli}
    + m^{(K)}_{tli}
    \bigl(
        (\mathbf K_{\mathrm{control}})_{tli}
        - (\mathbf K_{\mathrm{average}})_{tli}
    \bigr),
    \\
    (\mathbf V_{\mathrm{interp}})_{tli}
    &=
    (\mathbf V_{\mathrm{average}})_{tli}
    + m^{(V)}_{tli}
    \bigl(
        (\mathbf V_{\mathrm{control}})_{tli}
        - (\mathbf V_{\mathrm{average}})_{tli}
    \bigr),
    \\
    \M_{\mathrm{interp}}(m^{(K)},m^{(V)})
    &=
    (\mathbf K_{\mathrm{interp}},\mathbf V_{\mathrm{interp}}).
\end{aligned}
\end{equation}

We measured task performance by computing the average difference between the correct answer logit and the mean logit of the other candidate answers over a predefined collection of queries:
\begin{equation}
    \operatorname{Score}(f(\cdot))
    =
    \frac{1}{N_{\mathrm{queries}}}
    \sum_{\mathcal Q \in \text{Queries}}
    \left(
    f_{a^*(\mathcal Q)}(\mathcal Q)
    -
    \underset{a \neq a^*(\mathcal Q)}{\mathrm{mean}}
    f_a(\mathcal Q)
    \right).
\end{equation}
Here, $f_a(\mathcal Q)$ denotes the logit for answer $a$, and $a^*(\mathcal Q)$ is the correct answer.

On each iteration, the marginal effect of pruning each remaining key or value was estimated by evaluating the derivative of the scalar score with respect to each entry of either mask:
\begin{equation}
\begin{aligned}
    \frac{\partial}{\partial m^{(K)}_{tli}}
    &\operatorname{Score}\!\left(
        \Psi\!\left(
            \cdot,\M_{\mathrm{interp}}(m^{(K)}, m^{(V)}_{})
        \right)
    \right), \\
    \frac{\partial}{\partial m^{(V)}_{tli}}
    &\operatorname{Score}\!\left(
        \Psi\!\left(
            \cdot,\M_{\mathrm{interp}}(m^{(K)}, m^{(V)})
        \right)
    \right).
\end{aligned}
\end{equation}
Note that derivatives with respect to each entry of $m^{(K)}$ and $m^{(V)}$ can be evaluated simultaneously in a single backward pass. 

In practice, most key and value vectors could be erased with little effect on the score. We therefore began with a coarse schedule that erased a fixed fraction of the remaining vectors at each iteration. Once the score fell below a threshold, we rewound to an earlier point in the trajectory and continued erasing vectors one at a time, providing finer resolution around the decline in performance (Algorithm~\ref{SI-alg:iterative_erasure}). Finally, in practice, we averaged the score over queries from several prompts with independently sampled entity names and used the gradient of this mean score to guide pruning.

\begin{algorithm}[H]
\caption{Iterative erasure of key--value vectors}
\label{SI-alg:iterative_erasure}
\small
\begin{algorithmic}[1]
\Require Initial keys-first mask $m_0$; score $S(m)$;
         coarse fraction $\eta$; threshold $\tau$;
         rewind factor $\rho$
\Statex $m$: combined key and value masks;
        $N(m)$: total number of retained entries across both masks.

\State $m \gets m_0$
\State $S_{\mathrm{initial}} \gets S(m_0)$;
       $S_{\mathrm{erased}} \gets S(0)$

\While{$N(m) > 0$} \Comment{Coarse erasure}
    \State $s \gets S(m)$; $g \gets \nabla_m S(m)$
    \State Set to zero the $\lceil \eta N(m) \rceil$ retained
           mask entries with the smallest $|g|$
    \If{$\dfrac{s-S_{\mathrm{erased}}}
               {S_{\mathrm{initial}}-S_{\mathrm{erased}}}
          < \tau$}
        \State $N_{\mathrm{target}} \gets
            \min\!\left(N(m_0),\lceil \rho N(m) \rceil\right)$
        \State Rewind to the most recent mask with
               at least $N_{\mathrm{target}}$ retained entries
        \State \textbf{break}
    \EndIf
\EndWhile

\While{$N(m) > 0$} \Comment{Fine erasure}
    \State $g \gets \nabla_m S(m)$
    \State Set to zero the retained mask entry with the smallest $|g|$
\EndWhile

\State \Return the pruning trajectory, excluding steps undone by rewinding
\end{algorithmic}
\end{algorithm}

Figure~\ref{SI-fig:pruning_trajectories} shows the pruning trajectory and the distribution of retained keys and values for the sparse mask used in Fig.~\figref{fig:binding} of the main text. Several features of these results are of note:
\begin{enumerate}
    \item Name-dependent information could be ``erased'' from the vast majority of key and value vectors with little effect on the score.
    \item The score began to decline significantly when name information in roughly 200 keys or values remained, corresponding to approximately 1\% of the total number of keys and values. Therefore, a small subset of sites was sufficient to support retrieval. The subsequent decline in score was gradual, consistent with the relevant information being distributed across the retained sites.
    \item The candidate name-to-symbol and symbol-to-name pairs were distributed across depth.\footnote{Their restriction to the first and second halves of the model, respectively, follows by construction from the initial ``keys-first'' mask.}
    \item Candidate name-to-symbol pairs were concentrated at entity-name tokens and the tokens immediately following them. This may reflect the copying of information from entity-token positions to subsequent positions by previous-token heads \cite{SI-olsson2022induction}.
    \item At some points along the pruning trajectory, both the retained set of keys and values and its complement could support retrieval when tested separately (data not shown). This suggests that the candidate key--value pairs we identified are sufficient, but not necessary, for retrieval.
\end{enumerate}

\begin{figure*}[h]
    \centering
    \begin{tabular}{
        @{}c@{\hspace{0.02\textwidth}}
        c@{\hspace{0.02\textwidth}}c@{}
    }
        \makebox[0.24\textwidth][l]{\textbf{A}} &
        \makebox[0.24\textwidth][l]{\textbf{B}} &
        \makebox[0.48\textwidth][l]{\textbf{C}} \\[3pt]

        \includegraphics[
            width=0.24\textwidth
        ]{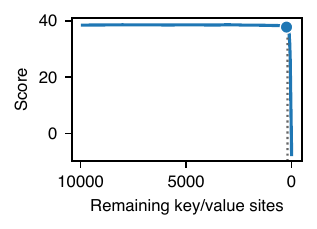}
        &
        \includegraphics[
            width=0.24\textwidth
        ]{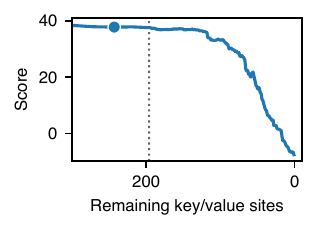}
        &
        \includegraphics[
            width=0.48\textwidth
        ]{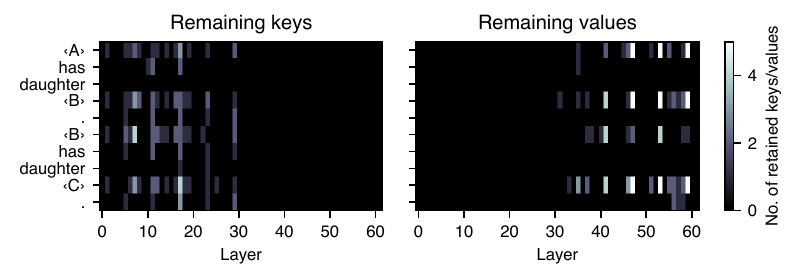}
    \end{tabular}
    \caption{
        Iterative erasure of key and value vectors. Results are shown 
        for Gemma-3-27B in the family-tree setting
        with ``who is'' queries. 
        \textbf{A}, Full erasure trajectory. Scores were 
        evaluated on the same prompts used to guide pruning.
        \textbf{B}, Expanded view of the trajectory.
        The vertical dashed line marks the transition to single-site
        erasure; the marker identifies the mask used for the main-text
        figure.
        \textbf{C}, Distribution of keys and values retained by the mask
        used for the main-text figure. 
    }
    \label{SI-fig:pruning_trajectories}
\end{figure*}
