# Supplementary material for: Cognitive Maps in Large Language Models
Source: arXiv:2610.25596 source file (2026-11-06)
Supplement: Supplementary file 9 [file 07_who_is_vs_yes_no.tex]

\section{Effects of Query Format}\label{SI-sec:query_format}

In the main text, we presented results using both yes-or-no queries (e.g., ``Is Carol's grandmother Alice?'') and queries requiring retrieval of a name (e.g., ``Who is Carol's grandmother?'').\footnote{One way to think about the difference between the two query formats is in terms of symmetries: In the first format, the answer to the query is \textit{invariant} under entity-replacement, whereas in the second setting, the answer is \textit{equivariant} under entity-replacement.}\textsuperscript{,}\footnote{In most other relational reasoning settings we studied, queries were more naturally phrased as yes-or-no questions.} We later tested both query formats for each experiment and found that, in all cases, the results were consistent with the account developed in the main text. Here, we present selected experiments using the alternative query format, and describe how the results of these experiments change with the alternative format.

Figure~\ref{SI-fig:query_format_who_is} shows the results of the mosaic experiment in main-text Fig.~\figref{fig:separability} using queries that require the model to retrieve a name. Three aspects of these data deserve comment:

\begin{enumerate}
    \item The query ``Who is Eve's mother?'' cleanly differentiates between the two hypotheses illustrated in the main text---under the attribute-tagging hypothesis, the model should respond ``Daisy''; under the identity--structure binding hypothesis, it should respond ``Alice''. The model responds ``Alice'' and assigns almost no additional probability to ``Daisy'' under the mosaic compared with the control (Fig.~\ref{SI-fig:query_format_who_is}A).\footnote{Here and throughout the SI, names are illustrative; entity names were independently resampled on each trial.}
    \item The model responds ``Carol'' to the question ``Who is Eve's daughter?'' and remains capable of answering the two-hop questions ``Who is Carol's grandmother?'' and ``Who is Alice's granddaughter?'' (Fig.~\ref{SI-fig:query_format_who_is}B, E, F). These observations parallel those in the main text that support the conclusion that the name-independent component of the activation tensor represents the complete relational structure instantiated by the prompt.
    \item When asked about Alice's daughter or Carol's mother, the model splits probability mass between ``Beth'' and ``Eve''. This is consistent with the schematic presented in the main text, where both ``Beth'' and ``Eve'' are bound to the same structural symbol.
\end{enumerate}

\begin{figure*}[h]
    \centering
    \begingroup


    \begin{figurepanel}{A}{0.28\textwidth}
        \includegraphics[width=\linewidth]{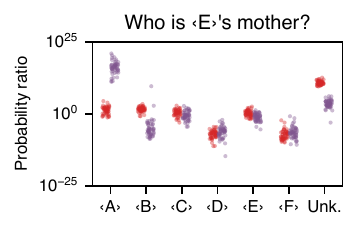}%
    \end{figurepanel}
    \hfill
    \begin{figurepanel}{C}{0.28\textwidth}
        \includegraphics[width=\linewidth]{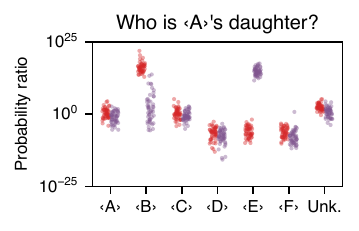}%
    \end{figurepanel}
    \hfill
    \begin{figurepanel}{E}{0.28\textwidth}
        \includegraphics[width=\linewidth]{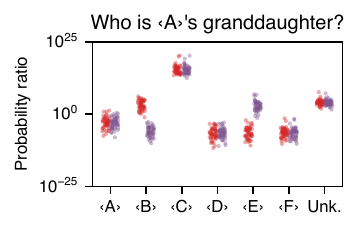}%
    \end{figurepanel}

    \par\medskip

    \begin{figurepanel}{B}{0.28\textwidth}
        \includegraphics[width=\linewidth]{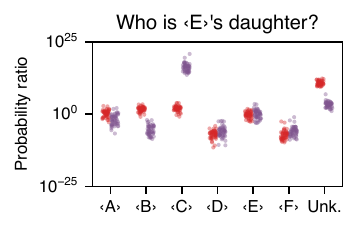}%
    \end{figurepanel}
    \hfill
    \begin{figurepanel}{D}{0.28\textwidth}
        \includegraphics[width=\linewidth]{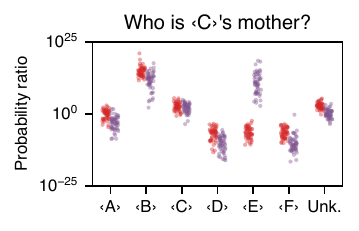}%
    \end{figurepanel}
    \hfill
    \begin{figurepanel}{F}{0.28\textwidth}
        \includegraphics[width=\linewidth]{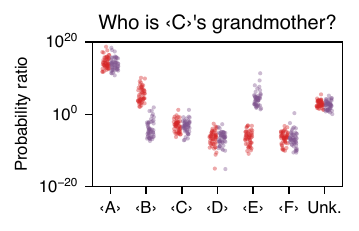}%
    \end{figurepanel}
    \par\smallskip
    \includegraphics[width=0.28\textwidth]{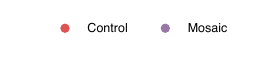}
    \endgroup

    \caption{
        Results under the \texttt{who-is} query format are consistent
        with identity-structure separation. 
        Responses are plotted
        for control (red) and mosaic (purple) activation tensors.
        The mosaic was constructed as in main-text Fig.~\figref{fig:separability}.
        Results are shown for Gemma-3-27B in the family-tree
        setting. Probability ratios are defined as in the
        main text. Fifty trials are shown per condition,
        with entity names independently resampled on each trial.
        The labels ‹A›, ‹B›, and ‹C› denote the control names
        in order of first appearance; ‹D›, ‹E›, and ‹F› denote
        the corresponding donor names.
    }
    \label{SI-fig:query_format_who_is}
\end{figure*}

Figure~\ref{SI-fig:query_format_yes_no} shows the results of experiments analogous to those presented in Fig.~\figref{fig:binding} using yes-or-no queries. We note that to answer a yes-or-no question (e.g., ``Is Beth's mother Alice?''), models can use at least two strategies. First, they can retrieve the information ``Beth's mother is Alice'' using the mechanism we described in the main text, compare the retrieved name with the ``Alice'' in the query, then respond ``yes''. Alternatively, they can retrieve the symbols corresponding to ``Alice'' and ``Beth'', compare them, and respond ``yes''. Note that the second strategy does not require symbol-to-name pairs.

The following observations support the sufficiency of the second strategy for answering yes-or-no questions:

\begin{enumerate}
    \item We constructed an additional \textit{keys-only} mosaic, which is similar to the \textit{keys-first} mosaic, except that values after the layer split are also replaced with their averages across prompts with resampled names:
    \begin{equation}
    \begin{aligned}
        (\mathbf K_{\text{keys-only}})_{tli}
        &=
        \begin{cases}
            (\mathbf K_{\text{control}})_{tli},
                & l \leq L_{\mathrm{split}}, \\
            (\mathbf K_{\text{average}})_{tli},
                & l > L_{\mathrm{split}},
        \end{cases}
        \\
        (\mathbf V_{\text{keys-only}})_{tli}
        &= (\mathbf V_{\text{average}})_{tli}.
    \end{aligned}
    \label{SI-eq:keys_only_mosaic}
    \end{equation}
    This mosaic removes name-dependent information from all values, including those of candidate symbol-to-name pairs.\footnote{This manipulation can be viewed as imposing an explicit relational bottleneck (see \cite{SI-webb2021emergent}) on the model.} We found that the model tolerated this manipulation with no major drop in performance (Fig.~\ref{SI-fig:query_format_yes_no}A).
    \item When we applied the iterative pruning procedure starting from the keys-first mosaic, the resulting sparse mosaic retained name-dependent information in 143 keys and 16 values while largely preserving performance (Fig.~\ref{SI-fig:query_format_yes_no}B--E). The much smaller number of retained values is consistent with a greater reliance on name-to-symbol pairs for these queries.
    \item We edited the key--value memory using a procedure analogous to that described in the main text. In Fig.~\ref{SI-fig:query_format_yes_no}F and G, we replaced the keys of candidate name-to-symbol pairs associated with the first entity with the corresponding donor keys. This intervention caused the model to answer yes to both ``Is Beth's mother Daisy?'' and ``Is Daisy's daughter Beth?''. Thus, editing keys associated with an entity altered responses to yes-or-no queries in both directions.
\end{enumerate}

\begin{figure*}[h]
    \centering
    \begingroup


    \begin{figurepanel}{A}{0.35\textwidth}
        \includegraphics[width=\linewidth]{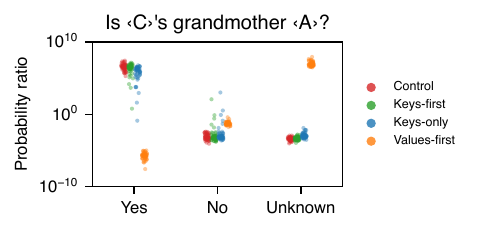}%
    \end{figurepanel}

    \par\medskip

    \begin{figurepanel}{B}{0.24\textwidth}
        \includegraphics[width=\linewidth]{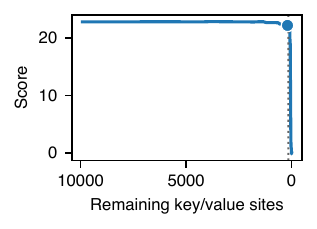}%
    \end{figurepanel}
    \hfill
    \begin{figurepanel}{C}{0.24\textwidth}
        \includegraphics[width=\linewidth]{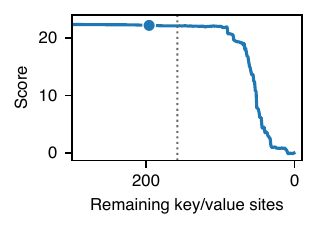}%
    \end{figurepanel}
    \hfill
    \begin{figurepanel}{D}{0.48\textwidth}
        \includegraphics[width=\linewidth]{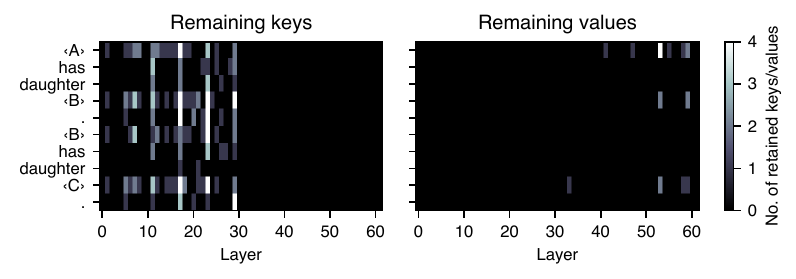}%
    \end{figurepanel}

    \par\medskip

    \begin{figurepanel}{E}{0.33\textwidth}
        \includegraphics[width=\linewidth]{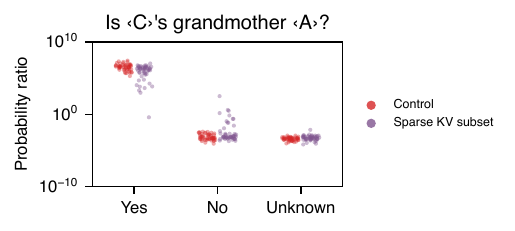}%
    \end{figurepanel}
    \hfill
    \begin{figurepanel}{F}{0.3\textwidth}
        \includegraphics[width=\linewidth]{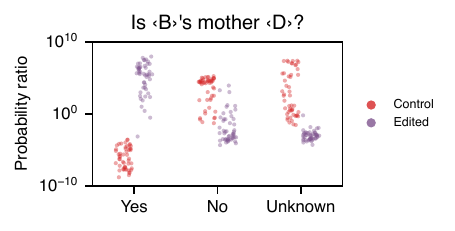}%
    \end{figurepanel}
    \hfill
    \begin{figurepanel}{G}{0.3\textwidth}
        \includegraphics[width=\linewidth]{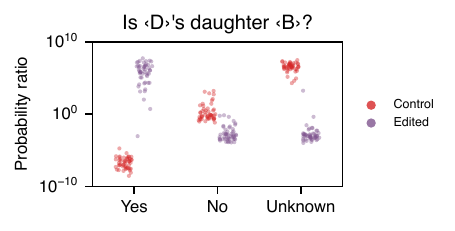}%
    \end{figurepanel}
    \endgroup

    \caption{
        Retrieval under the \texttt{yes-or-no} query format involves
        a sparse set of name-to-symbol pairs. Results are shown for Gemma-3-27B in 
        the family-tree setting. In all mosaic experiments, probability ratios are 
        defined as in the main text and fifty trials are shown per condition. 
        The labels ‹A›, ‹B›, and ‹C› denote the control names
        in order of first appearance, and ‹D› denotes the first
        donor name; these names are resampled on each trial.
        \textbf{A}, Restricting name-dependent information to keys
        before the layer split preserves performance.
        \textbf{B}, Full pruning trajectory starting from the
        keys-first mosaic. Scores were evaluated on the same
        prompts used to guide pruning.
        \textbf{C}, Expanded view of the trajectory.
        The vertical dashed line marks the transition to
        single-site pruning; the marker identifies the mask
        used in the subsequent panels.
        \textbf{D}, Distribution of the 143 keys and 16 values
        retained by this mask across token positions and layers.
        \textbf{E}, Performance is largely preserved when
        name-dependent information is restricted to the 143 keys
        and 16 values identified by iterative pruning.
        \textbf{F,G}, Editing candidate name-to-symbol pairs changes 
        the model's responses in both query directions.
    }
    \label{SI-fig:query_format_yes_no}
\end{figure*}
