# Supplementary material for: Cognitive Maps in Large Language Models
Source: arXiv:2610.25596 source file (2026-11-06)
Supplement: Supplementary file 10 [file 08_prompt_templates.tex]

\clearpage
\section{Prompt Templates}
\label{SI-sec:prompt_templates}

Here, we provide prompt templates for the fourteen relational reasoning tasks used in this study. These tasks span four task families\footnote{Formally, two tasks belong to the same task family if there is a one-to-one correspondence between the sets of relationships that preserves relationship composition.}: family trees (``family trees'', ``family trees (name-retrieval queries)'', ``ancestor--descendant relationships''); ordinal relationships (``company hierarchies'', ``age comparisons'', ``height comparisons'', ``speed comparisons'', ``east--west relationships'', ``north--south relationships'', ``ahead--behind relationships'', ``exact age differences''); signed interactions (``gene regulatory networks'', ``neural circuits''); and equivalence (``propositional equivalence'', ``variable equality'').

Entity names were sampled from fixed pools specific to each tokenizer family and prompt template. The complete pools are included in the accompanying code. Each template used one of five name pools:

\begin{itemize}
    \item \textit{Female given names} (\texttt{human\_names.txt}):
    ``family trees'', ``family trees (name-retrieval queries)'',
    ``ancestor--descendant relationships'', ``company hierarchies'',
    ``age comparisons'', ``height comparisons'', ``speed comparisons'',
    and ``exact age differences''.

    \item \textit{Place names} (\texttt{places.txt}):
    ``east--west relationships'', ``north--south relationships'',
    and ``ahead--behind relationships''.

    \item \textit{Roman numerals I--X} (\texttt{numbers.txt}):
    ``propositional equivalence''.

    \item \textit{Lowercase letters a--z} (\texttt{letters.txt}):
    ``variable equality''.

    \item \textit{Synthetic names} (\texttt{alien\_names.txt}):
    ``gene regulatory networks'' and ``neural circuits''.
\end{itemize}

All entity names were selected to tokenize as a single token both with and without a preceding space. For templates whose domain-appropriate names were not already synthetic, we additionally evaluated behavioral performance using synthetic names sampled from fixed pools of lowercase three-letter strings.

\begingroup
\raggedbottom

\subsection{Family Trees}

\noindent\begin{minipage}{\linewidth}
\begin{Verbatim}[breaklines=true, fontsize=\small]
Instructions:
1) Read the context describing a series of relationships between people in a family.
2) Keep track of who is related to whom as you read.
3) You may assume that everyone who appears in the context is female.
4) At the end, answer the question. You may use:
    (a) Information stated in the context.
    (b) Any facts that follow from the context by valid logical inference.
5) If the statement is true, output 'Yes'.
6) If the statement is false, output 'No'.
7) If the context does not uniquely determine an answer, output 'Unknown'. Do not guess.
8) Output exactly one word (no punctuation or extra text).

Context: ‹Alice› has ‹daughter/mother› ‹Beth›. ‹Beth› has ‹daughter/mother› ‹Carol›.

Question: Is ‹Carol›'s ‹grandmother› ‹Alice›?

Answer:
\end{Verbatim}
\end{minipage}

\subsection{Family Trees (Name-Retrieval Queries)}

\noindent\begin{minipage}{\linewidth}
\begin{Verbatim}[breaklines=true, fontsize=\small]
Instructions:
1) Read the context describing a series of relationships between people in a family.
2) Keep track of who is related to whom as you read.
3) You may assume that everyone who appears in the context is female.
4) At the end, answer the question. You may use:
    (a) Information stated in the context.
    (b) Any facts that follow from the context by valid logical inference.
5) If the context does not uniquely determine an answer, output 'Unknown'. Do not guess.
6) Output exactly one word (no punctuation or extra text).

Context: ‹Alice› has ‹daughter/mother› ‹Beth›. ‹Beth› has ‹daughter/mother› ‹Carol›.

Question: Who is ‹Carol›'s ‹grandmother›?

Answer:
\end{Verbatim}
\end{minipage}

\subsection{Ancestor--Descendant Relationships}

\noindent\begin{minipage}{\linewidth}
\begin{Verbatim}[breaklines=true, fontsize=\small]
Instructions:
1) Read the context describing a series of relationships between people in a family.
2) Keep track of who is related to whom as you read.
3) You may assume that everyone who appears in the context is female.
4) At the end, answer the question. You may use:
    (a) Information stated in the context.
    (b) Any facts that follow from the context by valid logical inference.
5) If the statement is true, output 'Yes'.
6) If the statement is false, output 'No'.
7) If the context does not uniquely determine an answer, output 'Unknown'. Do not guess.
8) Output exactly one word (no punctuation or extra text).

Context: ‹Alice› has ‹daughter/mother› ‹Beth›. ‹Beth› has ‹daughter/mother› ‹Carol›.

Question: Is ‹Carol› ‹a descendant› of ‹Alice›?

Answer:
\end{Verbatim}
\end{minipage}

\subsection{Company Hierarchies}

\noindent\begin{minipage}{\linewidth}
\begin{Verbatim}[breaklines=true, fontsize=\small]
Instructions:
1) Read the context describing the organizational structure in a company.
2) At the end, determine whether the statement in the question is true. You may use:
    (a) Information stated in the context.
    (b) Any facts that follow from the context by valid logical inference.
3) If the statement is true, output 'Yes'.
4) If the statement is false, output 'No'.
5) If the context does not uniquely determine an answer, output 'Unknown'. Do not guess.
6) Output exactly one word (no punctuation or extra text).

Context: ‹Alice›'s ‹boss/employee› is ‹Beth›. ‹Beth›'s ‹boss/employee› is ‹Carol›.

Question: Is ‹Carol› ‹senior› to ‹Alice›?

Answer:
\end{Verbatim}
\end{minipage}

\subsection{Age Comparisons}

\noindent\begin{minipage}{\linewidth}
\begin{Verbatim}[breaklines=true, fontsize=\small]
Instructions:
1) Read the context describing a series of comparisons between people.
2) At the end, determine whether the statement in the question is true. You may use:
    (a) Information stated in the context.
    (b) Any facts that follow from the context by valid logical inference.
3) If the statement is true, output 'Yes'.
4) If the statement is false, output 'No'.
5) If the context does not uniquely determine an answer, output 'Unknown'. Do not guess.
6) Output exactly one word (no punctuation or extra text).

Context: ‹Alice› is ‹older/younger› than ‹Beth›. ‹Beth› is ‹older/younger› than ‹Carol›.

Question: Is ‹Carol› ‹younger› than ‹Alice›?

Answer:
\end{Verbatim}
\end{minipage}

\subsection{Height Comparisons}

\noindent\begin{minipage}{\linewidth}
\begin{Verbatim}[breaklines=true, fontsize=\small]
Instructions:
1) Read the context describing a series of comparisons between people.
2) At the end, determine whether the statement in the question is true. You may use:
    (a) Information stated in the context.
    (b) Any facts that follow from the context by valid logical inference.
3) If the statement is true, output 'Yes'.
4) If the statement is false, output 'No'.
5) If the context does not uniquely determine an answer, output 'Unknown'. Do not guess.
6) Output exactly one word (no punctuation or extra text).

Context: ‹Alice› is ‹taller/shorter› than ‹Beth›. ‹Beth› is ‹taller/shorter› than ‹Carol›.

Question: Is ‹Carol› ‹shorter› than ‹Alice›?

Answer:
\end{Verbatim}
\end{minipage}

\subsection{Speed Comparisons}

\noindent\begin{minipage}{\linewidth}
\begin{Verbatim}[breaklines=true, fontsize=\small]
Instructions:
1) Read the context describing a series of comparisons between people.
2) At the end, determine whether the statement in the question is true. You may use:
    (a) Information stated in the context.
    (b) Any facts that follow from the context by valid logical inference.
3) If the statement is true, output 'Yes'.
4) If the statement is false, output 'No'.
5) If the context does not uniquely determine an answer, output 'Unknown'. Do not guess.
6) Output exactly one word (no punctuation or extra text).

Context: ‹Alice› is ‹faster/slower› than ‹Beth›. ‹Beth› is ‹faster/slower› than ‹Carol›.

Question: Is ‹Carol› ‹slower› than ‹Alice›?

Answer:
\end{Verbatim}
\end{minipage}

\subsection{East--West Relationships}

\noindent\begin{minipage}{\linewidth}
\begin{Verbatim}[breaklines=true, fontsize=\small]
Instructions:
1) Read the context describing a series of spatial relationships between locations.
2) At the end, determine whether the statement in the question is true. You may use:
    (a) Information stated in the context.
    (b) Any facts that follow from the context by valid logical inference.
3) If the statement is true, output 'Yes'.
4) If the statement is false, output 'No'.
5) If the context does not uniquely determine an answer, output 'Unknown'. Do not guess.
6) Output exactly one word (no punctuation or extra text).

Context: The ‹library› is ‹east/west› of the ‹museum›. The ‹museum› is ‹east/west› of the ‹station›.

Question: Is the ‹station› ‹west› of the ‹library›?

Answer:
\end{Verbatim}
\end{minipage}

\subsection{North--South Relationships}

\noindent\begin{minipage}{\linewidth}
\begin{Verbatim}[breaklines=true, fontsize=\small]
Instructions:
1) Read the context describing a series of spatial relationships between locations.
2) At the end, determine whether the statement in the question is true. You may use:
    (a) Information stated in the context.
    (b) Any facts that follow from the context by valid logical inference.
3) If the statement is true, output 'Yes'.
4) If the statement is false, output 'No'.
5) If the context does not uniquely determine an answer, output 'Unknown'. Do not guess.
6) Output exactly one word (no punctuation or extra text).

Context: The ‹library› is ‹north/south› of the ‹museum›. The ‹museum› is ‹north/south› of the ‹station›.

Question: Is the ‹station› ‹south› of the ‹library›?

Answer:
\end{Verbatim}
\end{minipage}

\subsection{Ahead--Behind Relationships\footnote{The wording ‘behind of’ is a grammatical error in the prompt template; the intended wording is ‘behind’. It is retained here to match the prompts presented to the model.}}

\noindent\begin{minipage}{\linewidth}
\begin{Verbatim}[breaklines=true, fontsize=\small]
Instructions:
1) Read the context describing a series of spatial relationships between locations.
2) At the end, determine whether the statement in the question is true. You may use:
    (a) Information stated in the context.
    (b) Any facts that follow from the context by valid logical inference.
3) If the statement is true, output 'Yes'.
4) If the statement is false, output 'No'.
5) If the context does not uniquely determine an answer, output 'Unknown'. Do not guess.
6) Output exactly one word (no punctuation or extra text).

Context: The ‹library› is ‹ahead/behind› of the ‹museum›. The ‹museum› is ‹ahead/behind› of the ‹station›.

Question: Is the ‹station› ‹behind› of the ‹library›?

Answer:
\end{Verbatim}
\end{minipage}

\subsection{Exact Age Differences\footnote{We grouped exact age differences with ordinal comparisons under ``ordering relationships'' for presentation, although specifying exact age differences changes the rules for composing relationships.}}

\noindent\begin{minipage}{\linewidth}
\begin{Verbatim}[breaklines=true, fontsize=\small]
Instructions:
1) Read the context describing a series of comparisons between people.
2) At the end, determine whether the statement in the question is true. You may use:
    (a) Information stated in the context.
    (b) Any facts that follow from the context by valid logical inference.
3) If the statement is true, output 'Yes'.
4) If the statement is false, output 'No'.
5) If the context does not uniquely determine an answer, output 'Unknown'. Do not guess.
6) Output exactly one word (no punctuation or extra text).

Context: ‹Alice› is ‹one year older/one year younger› than ‹Beth›. ‹Beth› is ‹one year older/one year younger› than ‹Carol›.

Question: Is ‹Carol› ‹two years younger› than ‹Alice›?

Answer:
\end{Verbatim}
\end{minipage}

\subsection{Gene Regulatory Networks}

\noindent\begin{minipage}{\linewidth}
\begin{Verbatim}[breaklines=true, fontsize=\small]
Instructions:
1) Read the context describing a simple gene regulatory network.
2) For this task, genes are identified by three-letter strings.
3) At the end, determine whether the statement in the question is true. You may use:
    (a) Information stated in the context.
    (b) Any facts that follow from the context by valid logical inference.
4) If the statement is true, output 'Yes'.
5) If the statement is false, output 'No'.
6) If the context does not uniquely determine an answer, output 'Unknown'. Do not guess.
7) Output exactly one word (no punctuation or extra text).

Context: ‹axs› ‹activates/represses› ‹bpy›. ‹bpy› ‹activates/represses› ‹chh›.

Question: Does ‹axs› ‹repress› ‹chh›?

Answer:
\end{Verbatim}
\end{minipage}

\subsection{Neural Circuits}

\noindent\begin{minipage}{\linewidth}
\begin{Verbatim}[breaklines=true, fontsize=\small]
Instructions:
1) Read the context describing a simple vertebrate neural circuit.
2) For this task, neurons are identified by three-letter strings.
3) At the end, determine whether the statement in the question is true. You may use:
    (a) Information stated in the context.
    (b) Any facts that follow from the context by valid logical inference.
4) If the statement is true, output 'Yes'.
5) If the statement is false, output 'No'.
6) If the context does not uniquely determine an answer, output 'Unknown'. Do not guess.
7) Output exactly one word (no punctuation or extra text).

Context: ‹axs› makes ‹glutamatergic/GABAergic› projections to ‹bpy›. ‹bpy› makes ‹glutamatergic/GABAergic› projections to ‹chh›.

Question: Does ‹axs› ‹inhibit› ‹chh›?

Answer:
\end{Verbatim}
\end{minipage}

\subsection{Propositional Equivalence}

\noindent\begin{minipage}{\linewidth}
\begin{Verbatim}[breaklines=true, fontsize=\small]
Instructions:
1) Read the context describing a series of relationships between propositions.
2) For this task, propositions are numbered by a roman numeral.
3) At the end, determine whether the statement in the question is true. You may use:
    (a) Information stated in the context.
    (b) Any facts that follow from the context by valid logical inference.
4) If the statement is true, output 'Yes'.
5) If the statement is false, output 'No'.
6) If the context does not uniquely determine an answer, output 'Unknown'. Do not guess.
7) Output exactly one word (no punctuation or extra text).

Context: ‹I› is ‹equivalent to/incompatible with› ‹II›. ‹II› is ‹equivalent to/incompatible with› ‹III›.

Question: Is ‹III› ‹equivalent to› ‹I›?

Answer:
\end{Verbatim}
\end{minipage}

\subsection{Variable Equality}

\noindent\begin{minipage}{\linewidth}
\begin{Verbatim}[breaklines=true, fontsize=\small]
Instructions:
1) Read the context describing a series of relationships between variables.
2) For this task, variables are identified by a single letter.
3) At the end, determine whether the statement in the question is true. You may use:
    (a) Information stated in the context.
    (b) Any facts that follow from the context by valid logical inference.
4) If the statement is true, output 'Yes'.
5) If the statement is false, output 'No'.
6) If the context does not uniquely determine an answer, output 'Unknown'. Do not guess.
7) Output exactly one word (no punctuation or extra text).

Context: ‹x› is ‹equal/not equal› to ‹y›. ‹y› is ‹equal/not equal› to ‹z›.

Question: Is ‹z› ‹equal› to ‹x›?

Answer:
\end{Verbatim}
\end{minipage}

\endgroup
