# Supplementary material for: Cognitive Maps in Large Language Models
Source: arXiv:2610.25596 source file (2026-11-06)
Supplement: Supplementary file 11 [file 09_all_tasks.tex]

\section{Analogous Experiments Across Relational Reasoning Tasks}

To assess the generality of the representational strategies we describe in the main text, we performed analogous experiments across various combinations of relational reasoning tasks (Section~\ref{SI-sec:prompt_templates}) and models (Table~\ref{SI-tab:model_revisions}). Here, we present the results of these experiments for Gemma-3-27B on all relational reasoning tasks; in the next section, we present results for all models on the ``family trees'' task. In several task families, queries are most naturally phrased as yes-or-no questions, so we use this query format throughout this and the next section. The accompanying code can be used to generate analogous plots for model–task combinations not shown here.

Across models and tasks, the qualitative results were broadly similar to those presented in the main text, with the following notable exceptions:

\begin{enumerate}
    \item \textit{Exceptions in settings with poor baseline task performance}
    (e.g., Figs.~\figref{SI-fig:separability-gemma27b-gene-regulatory-network}E, \figref{SI-fig:additivity-gemma27b-gene-regulatory-network}B,D, and \figref{SI-fig:model-generalization-separability-llama-8b}).
    When the model cannot reliably perform the underlying task, mosaic experiments may yield unexpected results. Because mosaic experiments use the models themselves to assess what information is available in the manipulated activation tensor, poor task performance makes these results difficult to interpret.
    \item \textit{Exceptions in the additivity experiments}
    (e.g., Figs.~\figref{SI-fig:additivity-gemma27b-east-west}, \figref{SI-fig:additivity-gemma27b-north-south}, and \figref{SI-fig:additivity-gemma27b-ahead-behind}).
    These exceptions were limited to the ordinal relationships task family. We speculate that they arise from redundant information in rows of $\mathbf A$ that follow entity-token rows. Such redundancy could arise if information from entity-token positions propagates to later positions (e.g., through previous-token heads \cite{SI-olsson2022induction}). Because the manipulation in Eq.~\eqref{SI-eq:additivity_mosaic} leaves these later rows unchanged, they may contain information that conflicts with the modified entity-token rows. Unexpected behavior could arise if the model retrieves information from both sets of rows at query time. Consistent with this idea, pruning experiments retain candidate name-to-symbol pairs at both entity-token positions and later positions (e.g., Fig.~\figref{SI-fig:erasure-north-south}C).
    \item \textit{Exceptions in the prospective--retrospective experiments}
    (Fig.~\figref{SI-fig:model-generalization-retrospective-prospective-llama-70b}D).
    As discussed in Section~\ref{SI-sec:prospective_composition}, such exceptions suggest that the activation tensor may contain information reflecting the prospective composition of relationships.
    \item \textit{Exceptions in the editing experiments}
    (e.g., Figs.~\figref{SI-fig:erasure-faster-slower}E, \figref{SI-fig:erasure-east-west}D, and \figref{SI-fig:erasure-north-south}D).
    We speculate that these exceptions arise from redundancy in the key--value memory. Specifically, the pruning procedure described in Section~\ref{SI-sec:pruning_trajectories} is designed to identify a set of key--value pairs for which retaining name-dependent information is \textit{sufficient} to mediate retrieval of all relationships. However, key--value pairs outside this subset may carry redundant information that influences behavior when the identified pairs are perturbed (see \cite{SI-wang2023interpretability} for evidence of redundant mechanisms in another setting). If this is the case, editing only the key--value pairs identified by the pruning procedure could leave conflicting information in unedited pairs, potentially accounting for some of the unexpected responses.
\end{enumerate}


\input{supplementary/sections/all_tasks/behavior}
\input{supplementary/sections/all_tasks/separability}
\input{supplementary/sections/all_tasks/additivity}
\input{supplementary/sections/all_tasks/retrospective_prospective}
\input{supplementary/sections/all_tasks/erasure}
