# Supplementary material for: Cognitive Maps in Large Language Models
Source: arXiv:2610.25596 source file (2026-11-06)
Supplement: Supplementary file 12 [file 10_all_models.tex]

\clearpage
\section{Analogous Experiments Across Model Families and Scales}
\input{supplementary/sections/all_models/separability}
\input{supplementary/sections/all_models/additivity}
\input{supplementary/sections/all_models/retrospective_prospective}
\input{supplementary/sections/all_models/erasure}
