# Supplementary material for: Cognitive Maps in Large Language Models
Source: arXiv:2610.25596 source file (2026-11-06)
Supplement: Supplementary file 14 [file erasure.tex]

\clearpage

\subsection{Key--value erasure and editing across models}

\begin{figure*}[!htbp]
    \centering
    \erasurepanels
        {\includegraphics[width=\linewidth]{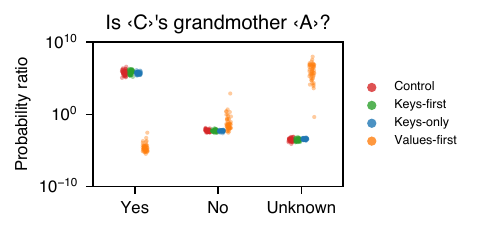}}
        {\includegraphics[width=\linewidth]{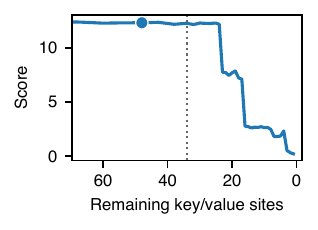}}
        {\includegraphics[width=\linewidth]{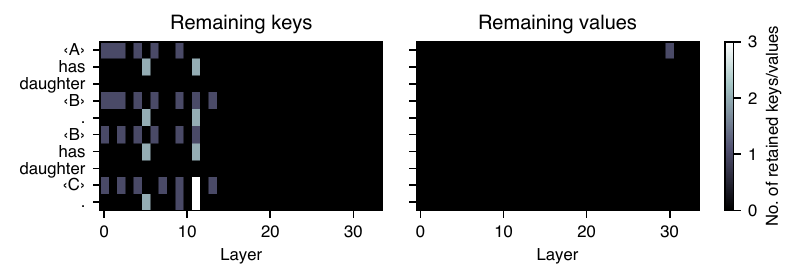}}
        {\includegraphics[width=\linewidth]{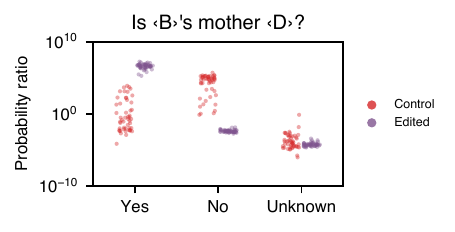}}
        {\includegraphics[width=\linewidth]{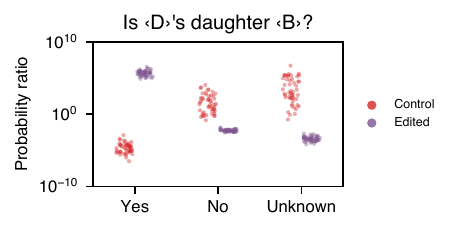}}
    \caption{\textbf{Key--value erasure and editing: Gemma-3-4B.}
        Results are shown for the ``family-trees'' setting. Procedures follow main-text Fig.~\figref{fig:binding}.
        The control context is ``‹A› has daughter ‹B›. ‹B› has daughter ‹C›'';
        the donor context is ``‹D› has daughter ‹E›. ‹E› has daughter ‹F›''.
        \textbf{A}, Responses for the keys-first, keys-only, and values-first memories.
        \textbf{B}, Final portion of the pruning trajectory.
        \textbf{C}, Distribution of the 47 keys and 1 value retained by this mask,
        together comprising 1.76\% of all key/value sites.
        \textbf{D, E}, Responses before and after replacing selected keys associated
        with the first entity in the control memory with the corresponding donor keys.
    }
    \label{SI-fig:model-generalization-erasure-gemma-4b}
\end{figure*}

\begin{figure*}[!htbp]
    \centering
    \erasurepanels
        {\includegraphics[width=\linewidth]{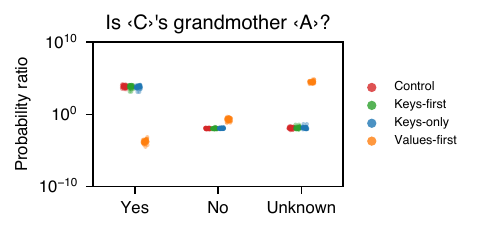}}
        {\includegraphics[width=\linewidth]{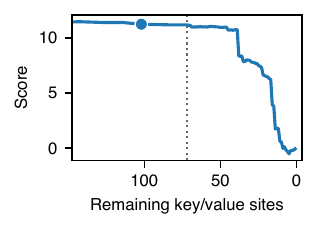}}
        {\includegraphics[width=\linewidth]{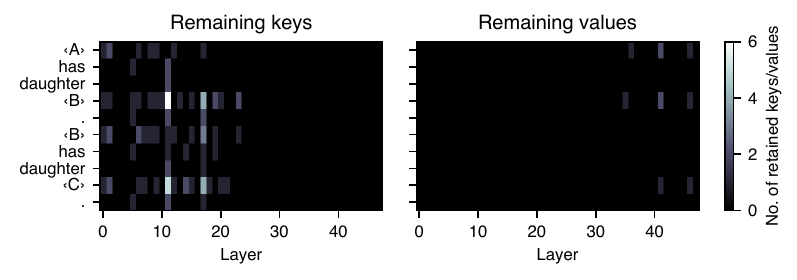}}
        {\includegraphics[width=\linewidth]{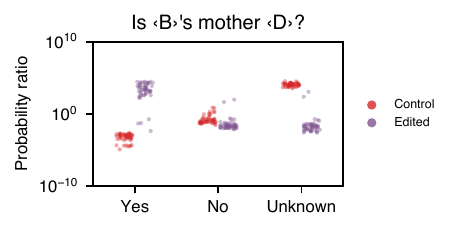}}
        {\includegraphics[width=\linewidth]{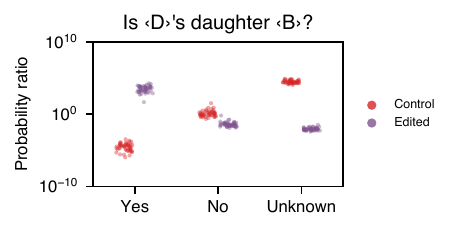}}
    \caption{\textbf{Key--value erasure and editing: Gemma-3-12B.}
        Results are shown for the ``family-trees'' setting. Procedures follow main-text Fig.~\figref{fig:binding}.
        The control context is ``‹A› has daughter ‹B›. ‹B› has daughter ‹C›'';
        the donor context is ``‹D› has daughter ‹E›. ‹E› has daughter ‹F›''.
        \textbf{A}, Responses for the keys-first, keys-only, and values-first memories.
        \textbf{B}, Final portion of the pruning trajectory.
        \textbf{C}, Distribution of the 92 keys and 10 values retained by this mask,
        together comprising 1.33\% of all key/value sites.
        \textbf{D, E}, Responses before and after replacing selected keys associated
        with the first entity in the control memory with the corresponding donor keys.
    }
    \label{SI-fig:model-generalization-erasure-gemma-12b}
\end{figure*}

\begin{figure*}[!htbp]
    \centering
    \erasurepanels
        {\includegraphics[width=\linewidth]{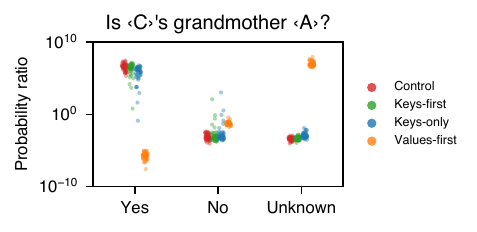}}
        {\includegraphics[width=\linewidth]{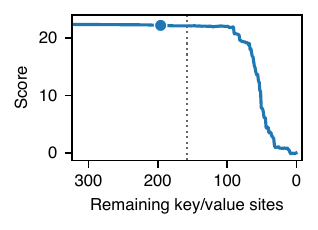}}
        {\includegraphics[width=\linewidth]{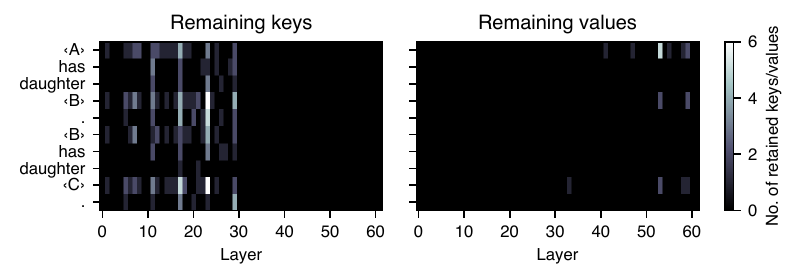}}
        {\includegraphics[width=\linewidth]{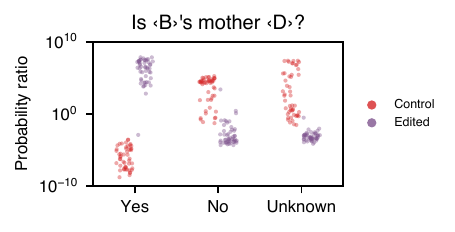}}
        {\includegraphics[width=\linewidth]{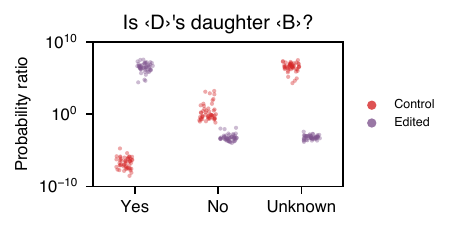}}
    \caption{\textbf{Key--value erasure and editing: Gemma-3-27B.}
        Results are shown for the ``family-trees'' setting. Procedures follow main-text Fig.~\figref{fig:binding}.
        The control context is ``‹A› has daughter ‹B›. ‹B› has daughter ‹C›'';
        the donor context is ``‹D› has daughter ‹E›. ‹E› has daughter ‹F›''.
        \textbf{A}, Responses for the keys-first, keys-only, and values-first memories.
        \textbf{B}, Final portion of the pruning trajectory.
        \textbf{C}, Distribution of the 176 keys and 20 values retained by this mask,
        together comprising 0.99\% of all key/value sites.
        \textbf{D, E}, Responses before and after replacing selected keys associated
        with the first entity in the control memory with the corresponding donor keys.
    }
    \label{SI-fig:model-generalization-erasure-gemma-27b}
\end{figure*}

\begin{figure*}[!htbp]
    \centering
    \erasurepanels
        {\includegraphics[width=\linewidth]{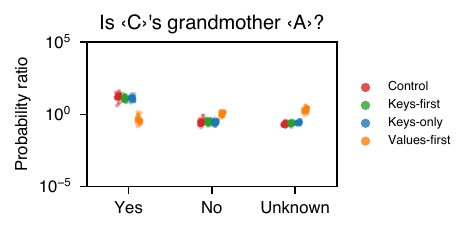}}
        {\includegraphics[width=\linewidth]{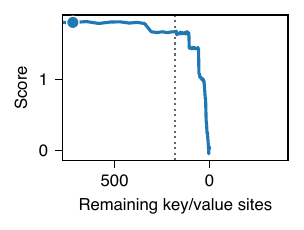}}
        {\includegraphics[width=\linewidth]{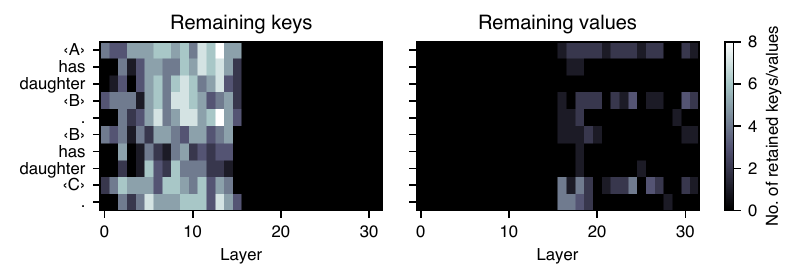}}
        {\includegraphics[width=\linewidth]{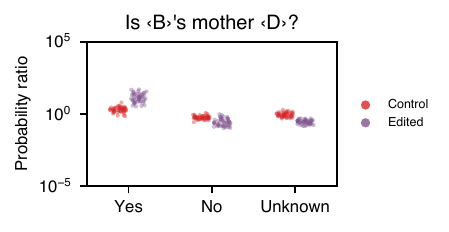}}
        {\includegraphics[width=\linewidth]{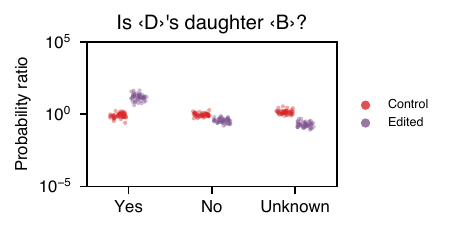}}
    \caption{\textbf{Key--value erasure and editing: Llama-3.1-8B.}
        Results are shown for the ``family-trees'' setting. Procedures follow main-text Fig.~\figref{fig:binding}.
        The control context is ``‹A› has daughter ‹B›. ‹B› has daughter ‹C›'';
        the donor context is ``‹D› has daughter ‹E›. ‹E› has daughter ‹F›''.
        \textbf{A}, Responses for the keys-first, keys-only, and values-first memories.
        \textbf{B}, Final portion of the pruning trajectory.
        \textbf{C}, Distribution of the 616 keys and 104 values retained by this mask,
        together comprising 14.06\% of all key/value sites.
        \textbf{D, E}, Responses before and after replacing selected keys associated
        with the first entity in the control memory with the corresponding donor keys.
    }
    \label{SI-fig:model-generalization-erasure-llama-8b}
\end{figure*}

\begin{figure*}[!htbp]
    \centering
    \erasurepanels
        {\includegraphics[width=\linewidth]{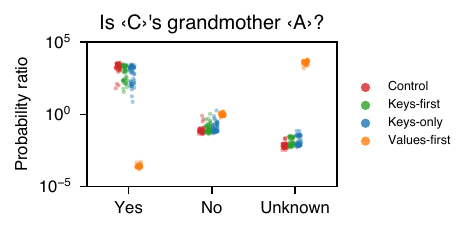}}
        {\includegraphics[width=\linewidth]{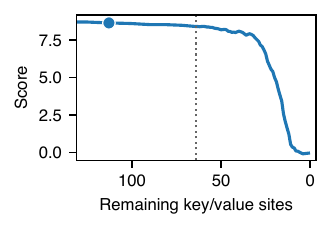}}
        {\includegraphics[width=\linewidth]{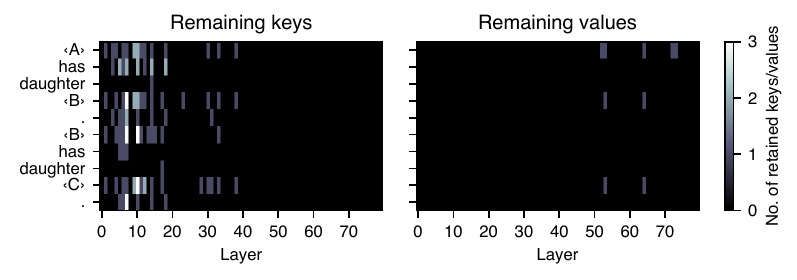}}
        {\includegraphics[width=\linewidth]{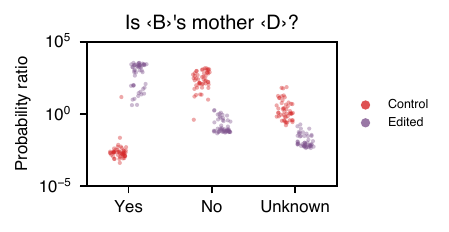}}
        {\includegraphics[width=\linewidth]{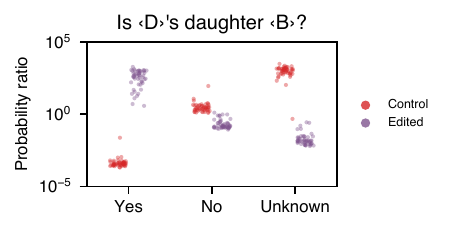}}
    \caption{\textbf{Key--value erasure and editing: Llama-3.1-70B.}
        Results are shown for the ``family-trees'' setting. Procedures follow main-text Fig.~\figref{fig:binding}.
        The control context is ``‹A› has daughter ‹B›. ‹B› has daughter ‹C›'';
        the donor context is ``‹D› has daughter ‹E›. ‹E› has daughter ‹F›''.
        \textbf{A}, Responses for the keys-first, keys-only, and values-first memories.
        \textbf{B}, Final portion of the pruning trajectory.
        \textbf{C}, Distribution of the 104 keys and 9 values retained by this mask,
        together comprising 0.88\% of all key/value sites.
        \textbf{D, E}, Responses before and after replacing selected keys associated
        with the first entity in the control memory with the corresponding donor keys.
    }
    \label{SI-fig:model-generalization-erasure-llama-70b}
\end{figure*}

\begin{figure*}[!htbp]
    \centering
    \erasurepanels
        {\includegraphics[width=\linewidth]{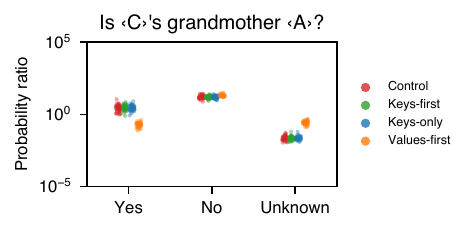}}
        {\includegraphics[width=\linewidth]{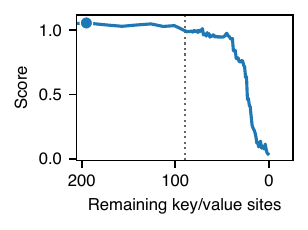}}
        {\includegraphics[width=\linewidth]{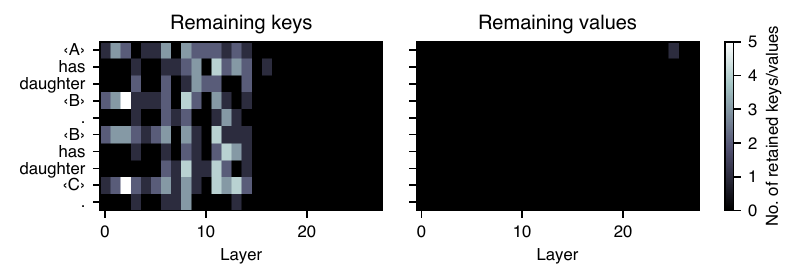}}
        {\includegraphics[width=\linewidth]{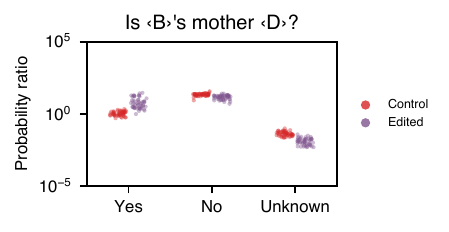}}
        {\includegraphics[width=\linewidth]{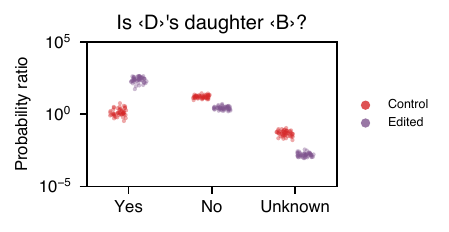}}
    \caption{\textbf{Key--value erasure and editing: Qwen-3-0.6B.}
        Results are shown for the ``family-trees'' setting. Procedures follow main-text Fig.~\figref{fig:binding}.
        The control context is ``‹A› has daughter ‹B›. ‹B› has daughter ‹C›'';
        the donor context is ``‹D› has daughter ‹E›. ‹E› has daughter ‹F›''.
        \textbf{A}, Responses for the keys-first, keys-only, and values-first memories.
        \textbf{B}, Final portion of the pruning trajectory.
        \textbf{C}, Distribution of the 194 keys and 1 value retained by this mask,
        together comprising 4.35\% of all key/value sites.
        \textbf{D, E}, Responses before and after replacing selected keys associated
        with the first entity in the control memory with the corresponding donor keys.
    }
    \label{SI-fig:model-generalization-erasure-qwen-0p6b}
\end{figure*}

\begin{figure*}[!htbp]
    \centering
    \erasurepanels
        {\includegraphics[width=\linewidth]{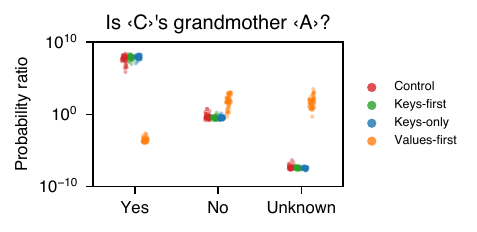}}
        {\includegraphics[width=\linewidth]{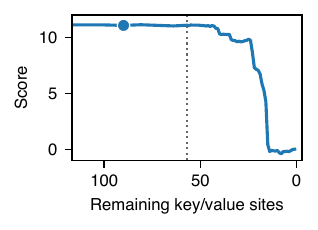}}
        {\includegraphics[width=\linewidth]{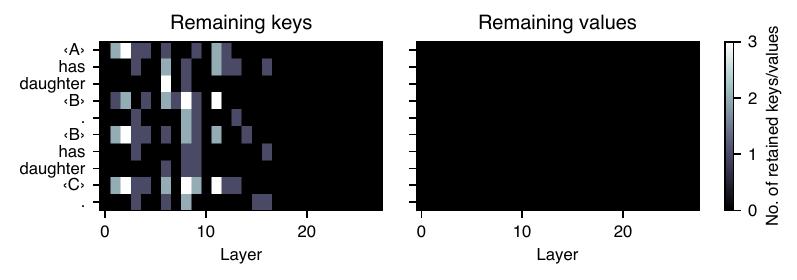}}
        {\includegraphics[width=\linewidth]{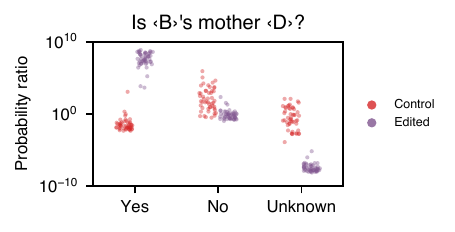}}
        {\includegraphics[width=\linewidth]{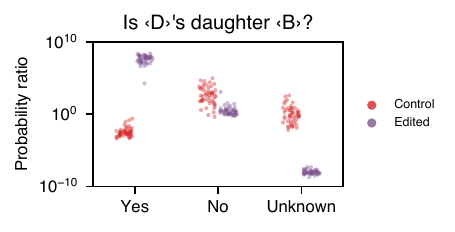}}
    \caption{\textbf{Key--value erasure and editing: Qwen-3-1.7B.}
        Results are shown for the ``family-trees'' setting. Procedures follow main-text Fig.~\figref{fig:binding}.
        The control context is ``‹A› has daughter ‹B›. ‹B› has daughter ‹C›'';
        the donor context is ``‹D› has daughter ‹E›. ‹E› has daughter ‹F›''.
        \textbf{A}, Responses for the keys-first, keys-only, and values-first memories.
        \textbf{B}, Final portion of the pruning trajectory.
        \textbf{C}, Distribution of the 90 keys and 0 values retained by this mask,
        together comprising 2.01\% of all key/value sites.
        \textbf{D, E}, Responses before and after replacing selected keys associated
        with the first entity in the control memory with the corresponding donor keys.
    }
    \label{SI-fig:model-generalization-erasure-qwen-1p7b}
\end{figure*}

\begin{figure*}[!htbp]
    \centering
    \erasurepanels
        {\includegraphics[width=\linewidth]{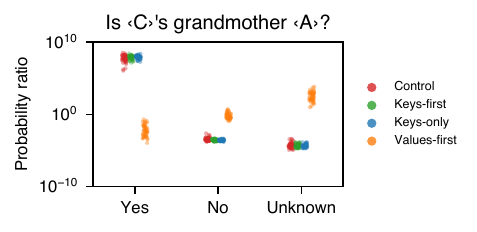}}
        {\includegraphics[width=\linewidth]{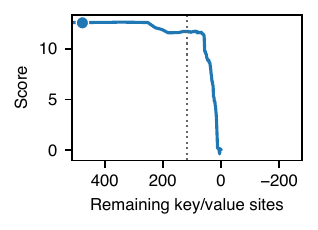}}
        {\includegraphics[width=\linewidth]{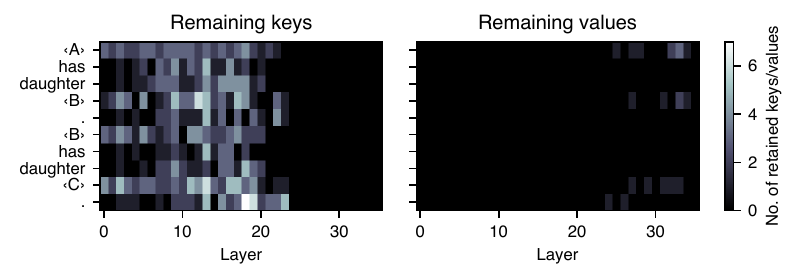}}
        {\includegraphics[width=\linewidth]{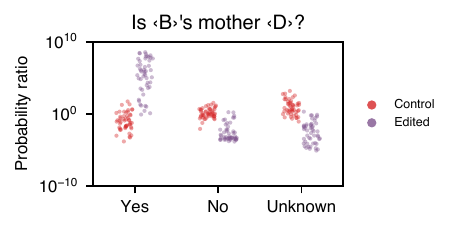}}
        {\includegraphics[width=\linewidth]{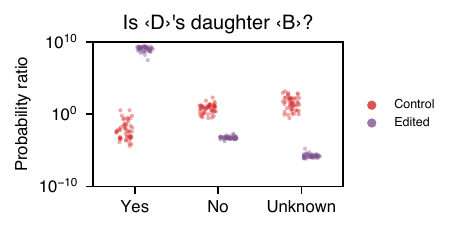}}
    \caption{\textbf{Key--value erasure and editing: Qwen-3-4B.}
        Results are shown for the ``family-trees'' setting. Procedures follow main-text Fig.~\figref{fig:binding}.
        The control context is ``‹A› has daughter ‹B›. ‹B› has daughter ‹C›'';
        the donor context is ``‹D› has daughter ‹E›. ‹E› has daughter ‹F›''.
        \textbf{A}, Responses for the keys-first, keys-only, and values-first memories.
        \textbf{B}, Final portion of the pruning trajectory.
        \textbf{C}, Distribution of the 456 keys and 21 values retained by this mask,
        together comprising 8.28\% of all key/value sites.
        \textbf{D, E}, Responses before and after replacing selected keys associated
        with the first entity in the control memory with the corresponding donor keys.
    }
    \label{SI-fig:model-generalization-erasure-qwen-4b}
\end{figure*}

\begin{figure*}[!htbp]
    \centering
    \erasurepanels
        {\includegraphics[width=\linewidth]{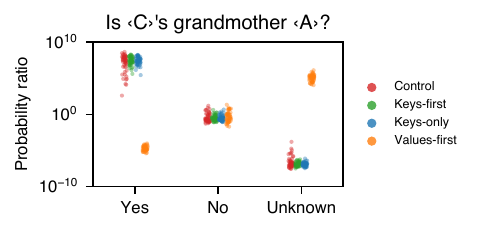}}
        {\includegraphics[width=\linewidth]{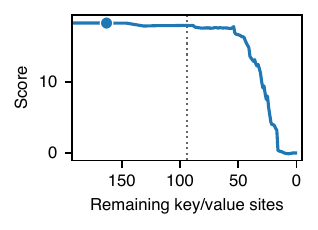}}
        {\includegraphics[width=\linewidth]{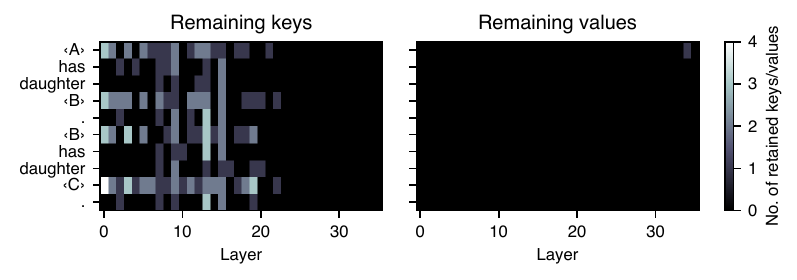}}
        {\includegraphics[width=\linewidth]{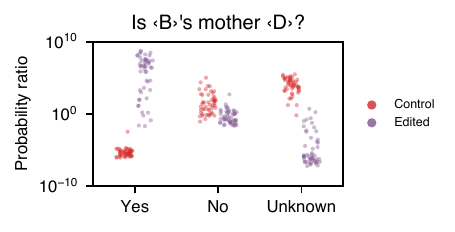}}
        {\includegraphics[width=\linewidth]{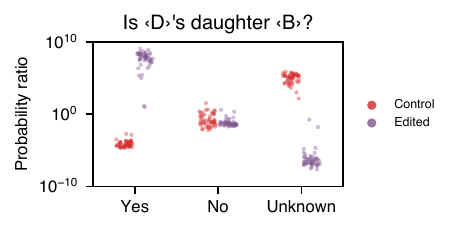}}
    \caption{\textbf{Key--value erasure and editing: Qwen-3-8B.}
        Results are shown for the ``family-trees'' setting. Procedures follow main-text Fig.~\figref{fig:binding}.
        The control context is ``‹A› has daughter ‹B›. ‹B› has daughter ‹C›'';
        the donor context is ``‹D› has daughter ‹E›. ‹E› has daughter ‹F›''.
        \textbf{A}, Responses for the keys-first, keys-only, and values-first memories.
        \textbf{B}, Final portion of the pruning trajectory.
        \textbf{C}, Distribution of the 162 keys and 1 value retained by this mask,
        together comprising 2.83\% of all key/value sites.
        \textbf{D, E}, Responses before and after replacing selected keys associated
        with the first entity in the control memory with the corresponding donor keys.
    }
    \label{SI-fig:model-generalization-erasure-qwen-8b}
\end{figure*}

\begin{figure*}[!htbp]
    \centering
    \erasurepanels
        {\includegraphics[width=\linewidth]{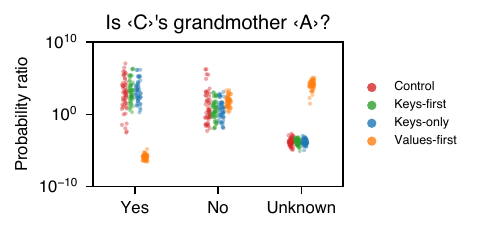}}
        {\includegraphics[width=\linewidth]{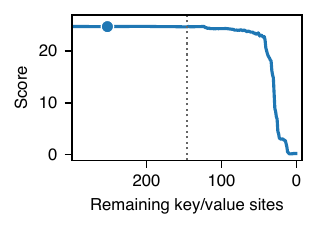}}
        {\includegraphics[width=\linewidth]{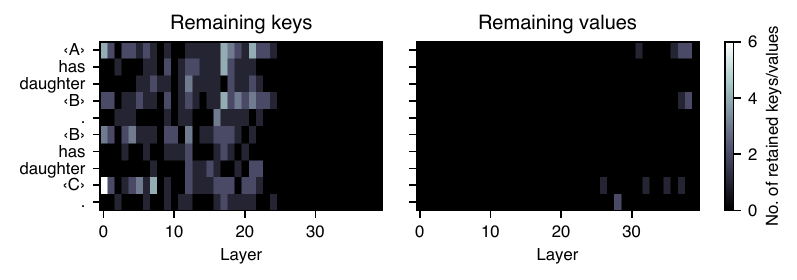}}
        {\includegraphics[width=\linewidth]{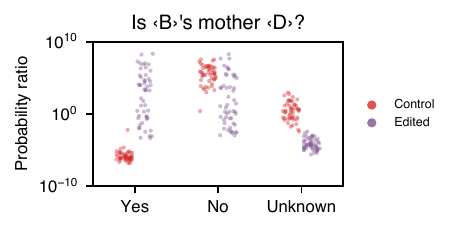}}
        {\includegraphics[width=\linewidth]{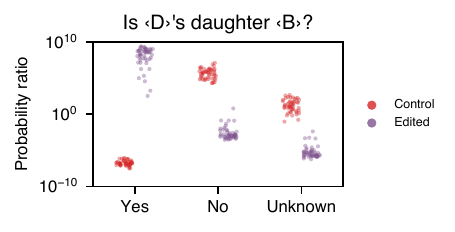}}
    \caption{\textbf{Key--value erasure and editing: Qwen-3-14B.}
        Results are shown for the ``family-trees'' setting. Procedures follow main-text Fig.~\figref{fig:binding}.
        The control context is ``‹A› has daughter ‹B›. ‹B› has daughter ‹C›'';
        the donor context is ``‹D› has daughter ‹E›. ‹E› has daughter ‹F›''.
        \textbf{A}, Responses for the keys-first, keys-only, and values-first memories.
        \textbf{B}, Final portion of the pruning trajectory.
        \textbf{C}, Distribution of the 237 keys and 15 values retained by this mask,
        together comprising 3.94\% of all key/value sites.
        \textbf{D, E}, Responses before and after replacing selected keys associated
        with the first entity in the control memory with the corresponding donor keys.
    }
    \label{SI-fig:model-generalization-erasure-qwen-14b}
\end{figure*}

\begin{figure*}[!htbp]
    \centering
    \erasurepanels
        {\includegraphics[width=\linewidth]{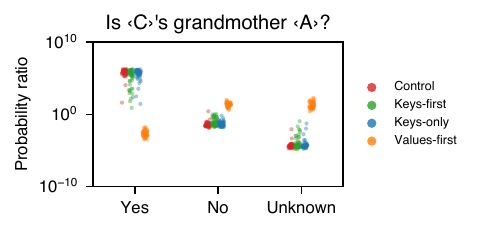}}
        {\includegraphics[width=\linewidth]{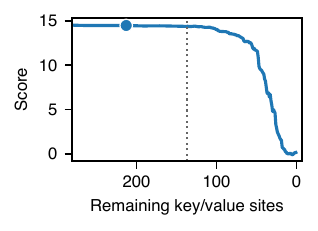}}
        {\includegraphics[width=\linewidth]{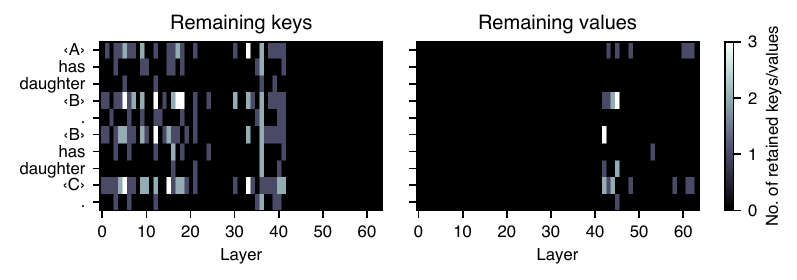}}
        {\includegraphics[width=\linewidth]{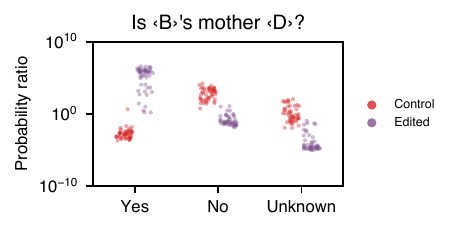}}
        {\includegraphics[width=\linewidth]{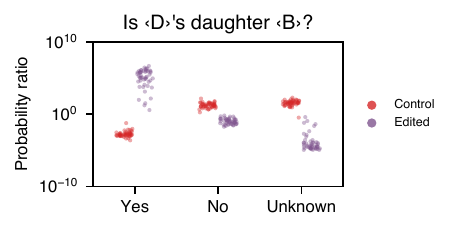}}
    \caption{\textbf{Key--value erasure and editing: Qwen-3-32B.}
        Results are shown for the ``family-trees'' setting. Procedures follow main-text Fig.~\figref{fig:binding}.
        The control context is ``‹A› has daughter ‹B›. ‹B› has daughter ‹C›'';
        the donor context is ``‹D› has daughter ‹E›. ‹E› has daughter ‹F›''.
        \textbf{A}, Responses for the keys-first, keys-only, and values-first memories.
        \textbf{B}, Final portion of the pruning trajectory.
        \textbf{C}, Distribution of the 183 keys and 30 values retained by this mask,
        together comprising 2.08\% of all key/value sites.
        \textbf{D, E}, Responses before and after replacing selected keys associated
        with the first entity in the control memory with the corresponding donor keys.
    }
    \label{SI-fig:model-generalization-erasure-qwen-32b}
\end{figure*}
