# Supplementary material for: Cognitive Maps in Large Language Models
Source: arXiv:2610.25596 source file (2026-11-06)
Supplement: Supplementary file 16 [file separability.tex]

\subsection{Identity--structure separability across models}

\begin{figure*}[!htbp]
    \centering
    \sixpanelgrid
        {\includegraphics[width=\linewidth]{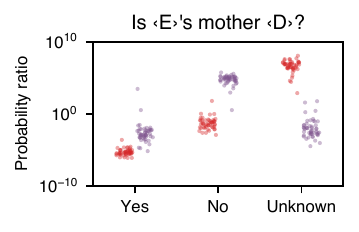}}
        {\includegraphics[width=\linewidth]{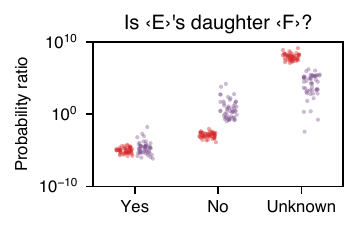}}
        {\includegraphics[width=\linewidth]{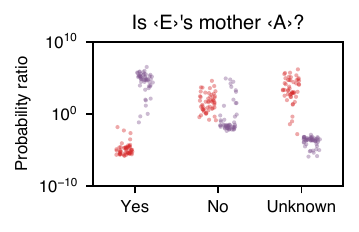}}
        {\includegraphics[width=\linewidth]{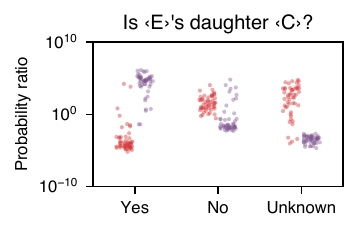}}
        {\includegraphics[width=\linewidth]{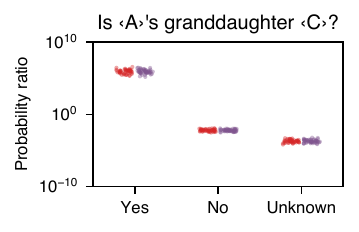}}
        {\includegraphics[width=\linewidth]{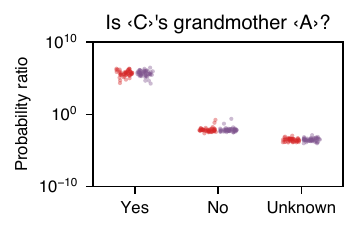}}
        {\includegraphics[width=0.28\textwidth]{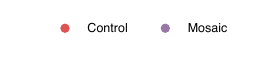}}
    \caption{
        \textbf{Identity--structure separability: Gemma-3-4B.}
        Results are shown for the ``family-trees'' setting.
        The control context is ``‹A› has daughter ‹B›. ‹B› has daughter ‹C›'';
        the donor context is ``‹D› has daughter ‹E›. ‹E› has daughter ‹F›''.
        The mosaic was constructed as in main-text Fig.~\figref{fig:separability}.
    }
    \label{SI-fig:model-generalization-separability-gemma-4b}
\end{figure*}

\begin{figure*}[!htbp]
    \centering
    \sixpanelgrid
        {\includegraphics[width=\linewidth]{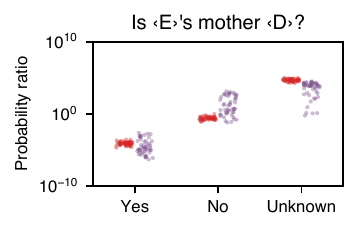}}
        {\includegraphics[width=\linewidth]{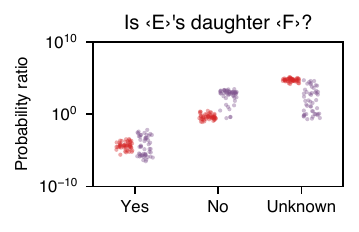}}
        {\includegraphics[width=\linewidth]{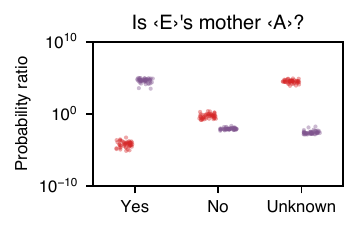}}
        {\includegraphics[width=\linewidth]{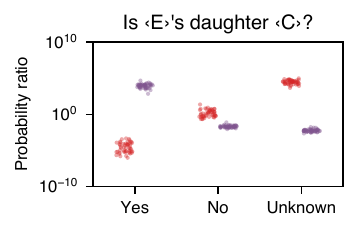}}
        {\includegraphics[width=\linewidth]{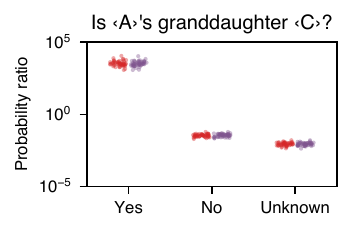}}
        {\includegraphics[width=\linewidth]{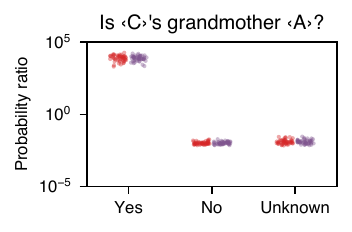}}
        {\includegraphics[width=0.28\textwidth]{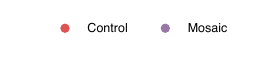}}
    \caption{
        \textbf{Identity--structure separability: Gemma-3-12B.}
        Results are shown for the ``family-trees'' setting.
        The control context is ``‹A› has daughter ‹B›. ‹B› has daughter ‹C›'';
        the donor context is ``‹D› has daughter ‹E›. ‹E› has daughter ‹F›''.
        The mosaic was constructed as in main-text Fig.~\figref{fig:separability}.
    }
    \label{SI-fig:model-generalization-separability-gemma-12b}
\end{figure*}

\begin{figure*}[!htbp]
    \centering
    \sixpanelgrid
        {\includegraphics[width=\linewidth]{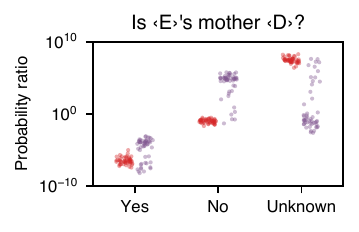}}
        {\includegraphics[width=\linewidth]{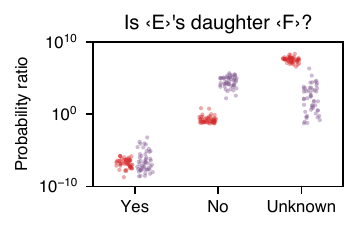}}
        {\includegraphics[width=\linewidth]{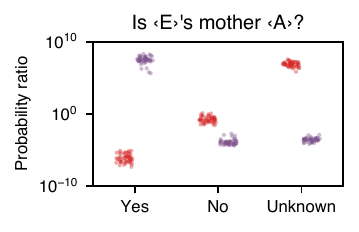}}
        {\includegraphics[width=\linewidth]{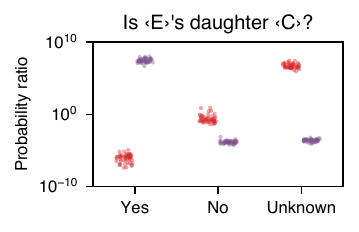}}
        {\includegraphics[width=\linewidth]{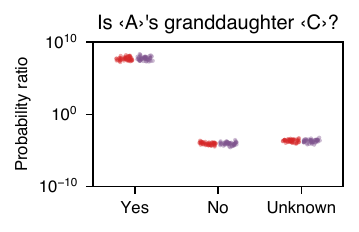}}
        {\includegraphics[width=\linewidth]{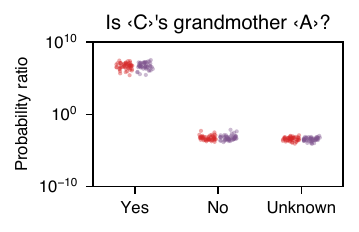}}
        {\includegraphics[width=0.28\textwidth]{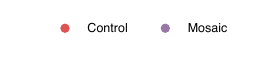}}
    \caption{
        \textbf{Identity--structure separability: Gemma-3-27B.}
        Results are shown for the ``family-trees'' setting.
        The control context is ``‹A› has daughter ‹B›. ‹B› has daughter ‹C›'';
        the donor context is ``‹D› has daughter ‹E›. ‹E› has daughter ‹F›''.
        The mosaic was constructed as in main-text Fig.~\figref{fig:separability}.
    }
    \label{SI-fig:model-generalization-separability-gemma-27b}
\end{figure*}

\begin{figure*}[!htbp]
    \centering
    \sixpanelgrid
        {\includegraphics[width=\linewidth]{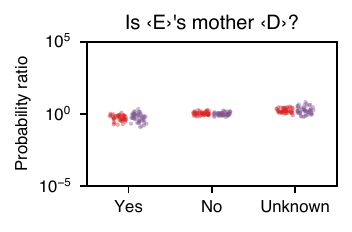}}
        {\includegraphics[width=\linewidth]{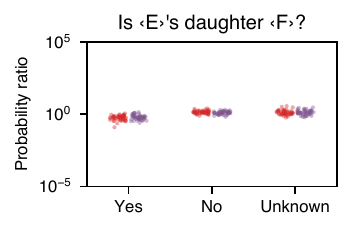}}
        {\includegraphics[width=\linewidth]{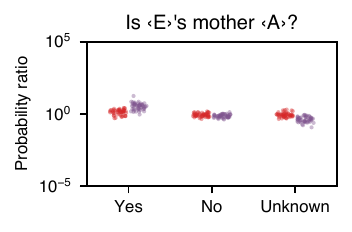}}
        {\includegraphics[width=\linewidth]{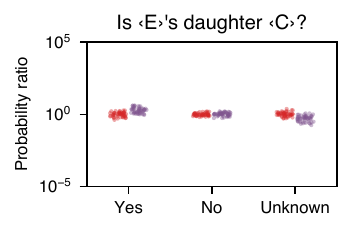}}
        {\includegraphics[width=\linewidth]{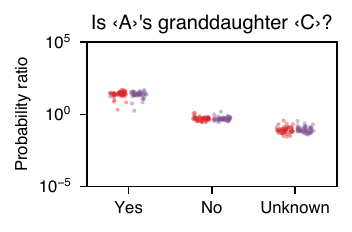}}
        {\includegraphics[width=\linewidth]{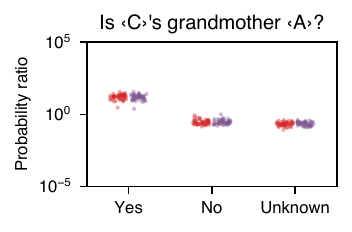}}
        {\includegraphics[width=0.28\textwidth]{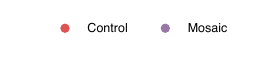}}
    \caption{
        \textbf{Identity--structure separability: Llama-3.1-8B.}
        Results are shown for the ``family-trees'' setting.
        The control context is ``‹A› has daughter ‹B›. ‹B› has daughter ‹C›'';
        the donor context is ``‹D› has daughter ‹E›. ‹E› has daughter ‹F›''.
        The mosaic was constructed as in main-text Fig.~\figref{fig:separability}.
    }
    \label{SI-fig:model-generalization-separability-llama-8b}
\end{figure*}

\begin{figure*}[!htbp]
    \centering
    \sixpanelgrid
        {\includegraphics[width=\linewidth]{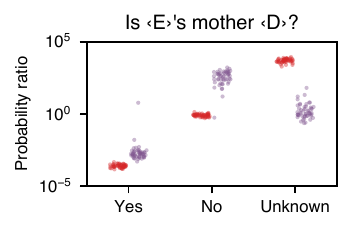}}
        {\includegraphics[width=\linewidth]{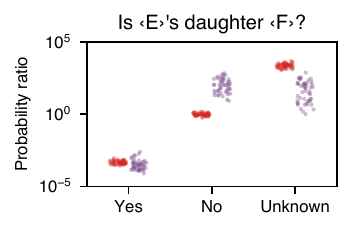}}
        {\includegraphics[width=\linewidth]{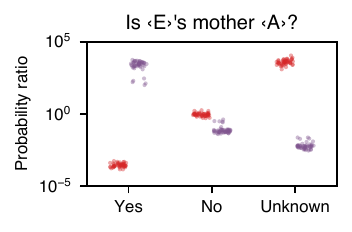}}
        {\includegraphics[width=\linewidth]{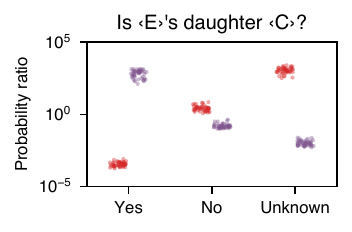}}
        {\includegraphics[width=\linewidth]{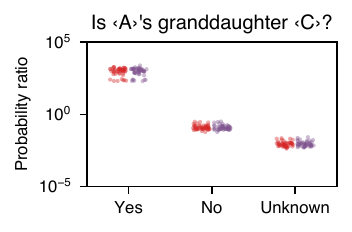}}
        {\includegraphics[width=\linewidth]{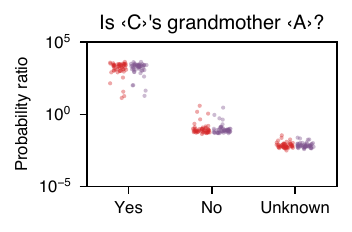}}
        {\includegraphics[width=0.28\textwidth]{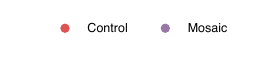}}
    \caption{
        \textbf{Identity--structure separability: Llama-3.1-70B.}
        Results are shown for the ``family-trees'' setting.
        The control context is ``‹A› has daughter ‹B›. ‹B› has daughter ‹C›'';
        the donor context is ``‹D› has daughter ‹E›. ‹E› has daughter ‹F›''.
        The mosaic was constructed as in main-text Fig.~\figref{fig:separability}.
    }
    \label{SI-fig:model-generalization-separability-llama-70b}
\end{figure*}

\begin{figure*}[!htbp]
    \centering
    \sixpanelgrid
        {\includegraphics[width=\linewidth]{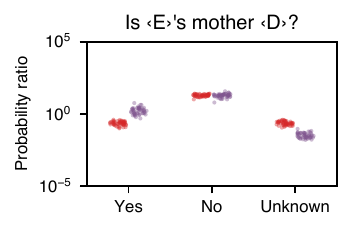}}
        {\includegraphics[width=\linewidth]{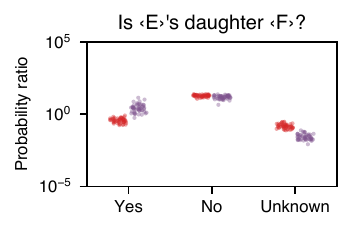}}
        {\includegraphics[width=\linewidth]{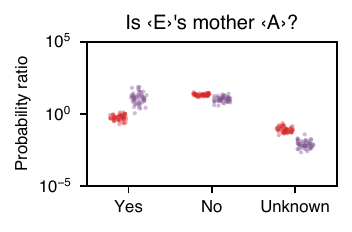}}
        {\includegraphics[width=\linewidth]{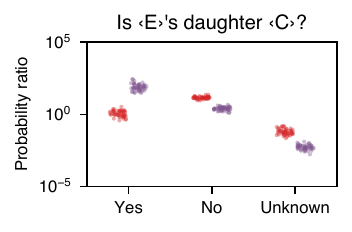}}
        {\includegraphics[width=\linewidth]{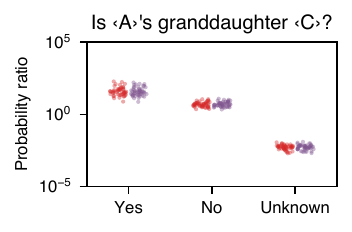}}
        {\includegraphics[width=\linewidth]{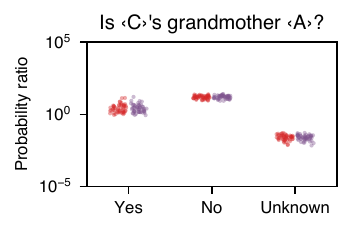}}
        {\includegraphics[width=0.28\textwidth]{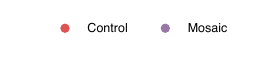}}
    \caption{
        \textbf{Identity--structure separability: Qwen-3-0.6B.}
        Results are shown for the ``family-trees'' setting.
        The control context is ``‹A› has daughter ‹B›. ‹B› has daughter ‹C›'';
        the donor context is ``‹D› has daughter ‹E›. ‹E› has daughter ‹F›''.
        The mosaic was constructed as in main-text Fig.~\figref{fig:separability}.
    }
    \label{SI-fig:model-generalization-separability-qwen-0p6b}
\end{figure*}

\begin{figure*}[!htbp]
    \centering
    \sixpanelgrid
        {\includegraphics[width=\linewidth]{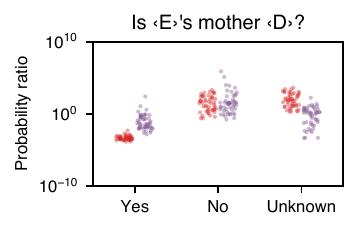}}
        {\includegraphics[width=\linewidth]{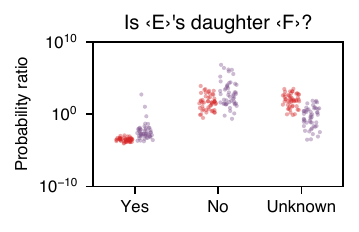}}
        {\includegraphics[width=\linewidth]{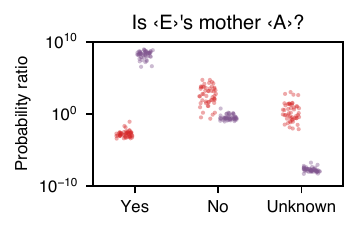}}
        {\includegraphics[width=\linewidth]{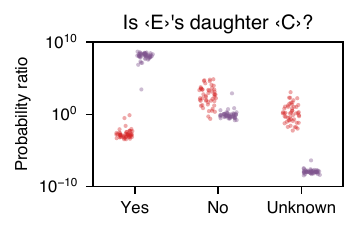}}
        {\includegraphics[width=\linewidth]{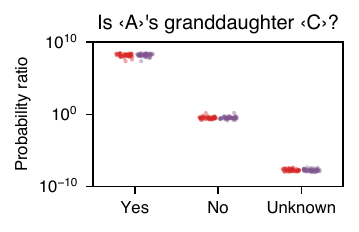}}
        {\includegraphics[width=\linewidth]{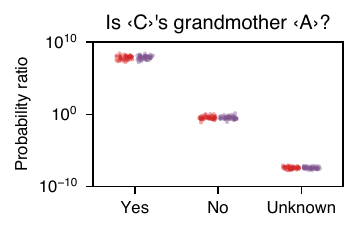}}
        {\includegraphics[width=0.28\textwidth]{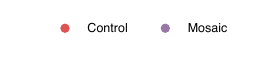}}
    \caption{
        \textbf{Identity--structure separability: Qwen-3-1.7B.}
        Results are shown for the ``family-trees'' setting.
        The control context is ``‹A› has daughter ‹B›. ‹B› has daughter ‹C›'';
        the donor context is ``‹D› has daughter ‹E›. ‹E› has daughter ‹F›''.
        The mosaic was constructed as in main-text Fig.~\figref{fig:separability}.
    }
    \label{SI-fig:model-generalization-separability-qwen-1p7b}
\end{figure*}

\begin{figure*}[!htbp]
    \centering
    \sixpanelgrid
        {\includegraphics[width=\linewidth]{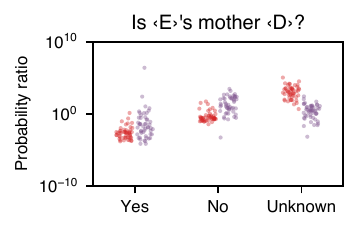}}
        {\includegraphics[width=\linewidth]{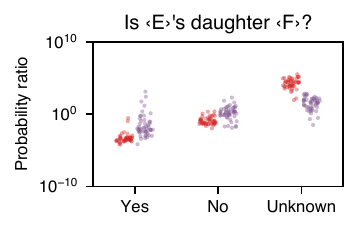}}
        {\includegraphics[width=\linewidth]{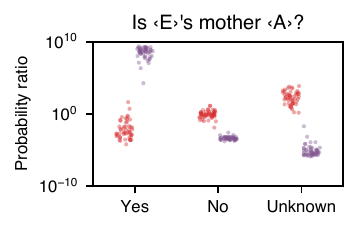}}
        {\includegraphics[width=\linewidth]{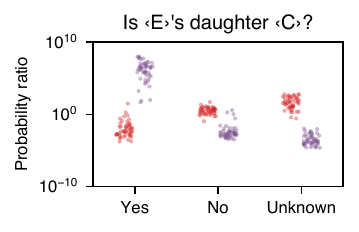}}
        {\includegraphics[width=\linewidth]{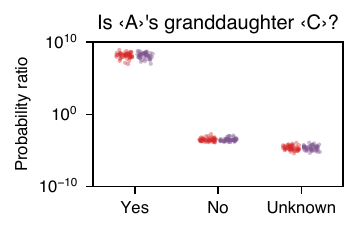}}
        {\includegraphics[width=\linewidth]{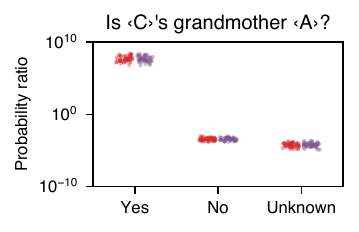}}
        {\includegraphics[width=0.28\textwidth]{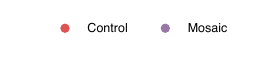}}
    \caption{
        \textbf{Identity--structure separability: Qwen-3-4B.}
        Results are shown for the ``family-trees'' setting.
        The control context is ``‹A› has daughter ‹B›. ‹B› has daughter ‹C›'';
        the donor context is ``‹D› has daughter ‹E›. ‹E› has daughter ‹F›''.
        The mosaic was constructed as in main-text Fig.~\figref{fig:separability}.
    }
    \label{SI-fig:model-generalization-separability-qwen-4b}
\end{figure*}

\begin{figure*}[!htbp]
    \centering
    \sixpanelgrid
        {\includegraphics[width=\linewidth]{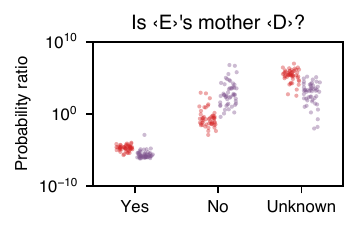}}
        {\includegraphics[width=\linewidth]{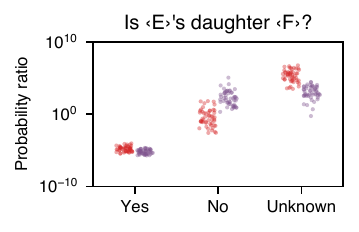}}
        {\includegraphics[width=\linewidth]{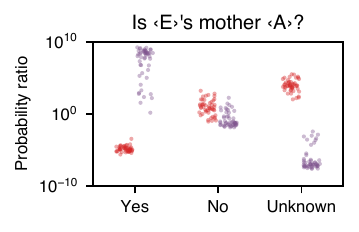}}
        {\includegraphics[width=\linewidth]{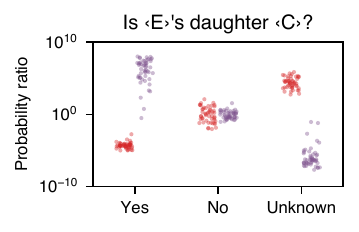}}
        {\includegraphics[width=\linewidth]{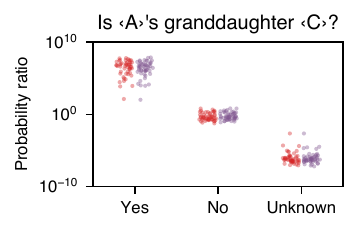}}
        {\includegraphics[width=\linewidth]{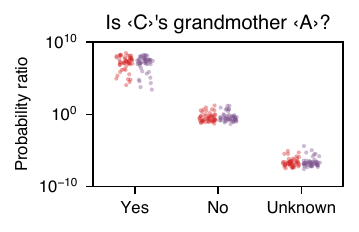}}
        {\includegraphics[width=0.28\textwidth]{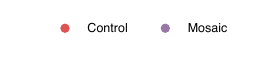}}
    \caption{
        \textbf{Identity--structure separability: Qwen-3-8B.}
        Results are shown for the ``family-trees'' setting.
        The control context is ``‹A› has daughter ‹B›. ‹B› has daughter ‹C›'';
        the donor context is ``‹D› has daughter ‹E›. ‹E› has daughter ‹F›''.
        The mosaic was constructed as in main-text Fig.~\figref{fig:separability}.
    }
    \label{SI-fig:model-generalization-separability-qwen-8b}
\end{figure*}

\begin{figure*}[!htbp]
    \centering
    \sixpanelgrid
        {\includegraphics[width=\linewidth]{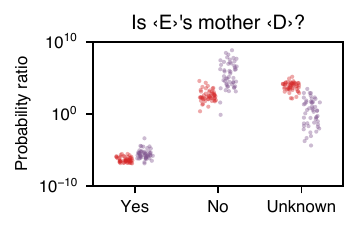}}
        {\includegraphics[width=\linewidth]{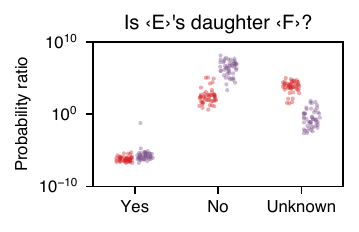}}
        {\includegraphics[width=\linewidth]{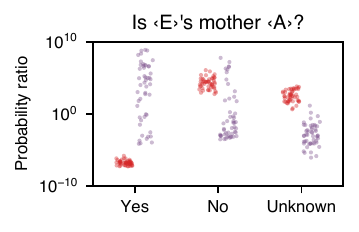}}
        {\includegraphics[width=\linewidth]{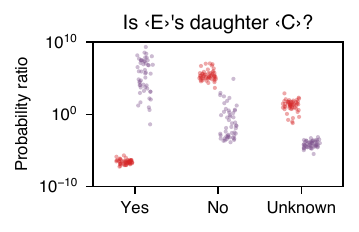}}
        {\includegraphics[width=\linewidth]{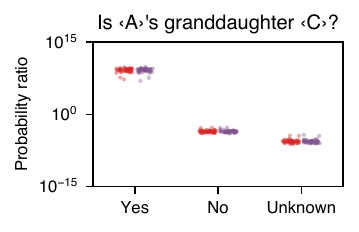}}
        {\includegraphics[width=\linewidth]{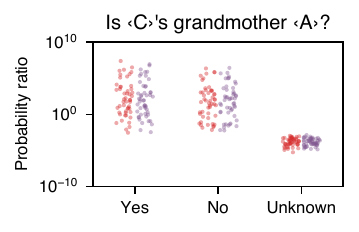}}
        {\includegraphics[width=0.28\textwidth]{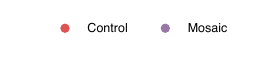}}
    \caption{
        \textbf{Identity--structure separability: Qwen-3-14B.}
        Results are shown for the ``family-trees'' setting.
        The control context is ``‹A› has daughter ‹B›. ‹B› has daughter ‹C›'';
        the donor context is ``‹D› has daughter ‹E›. ‹E› has daughter ‹F›''.
        The mosaic was constructed as in main-text Fig.~\figref{fig:separability}.
    }
    \label{SI-fig:model-generalization-separability-qwen-14b}
\end{figure*}

\begin{figure*}[!htbp]
    \centering
    \sixpanelgrid
        {\includegraphics[width=\linewidth]{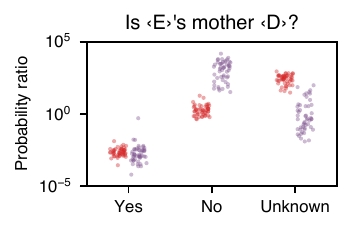}}
        {\includegraphics[width=\linewidth]{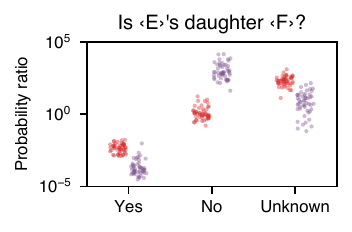}}
        {\includegraphics[width=\linewidth]{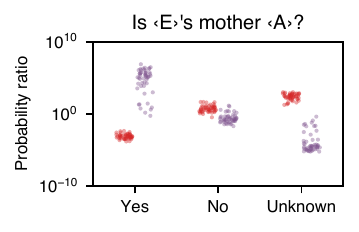}}
        {\includegraphics[width=\linewidth]{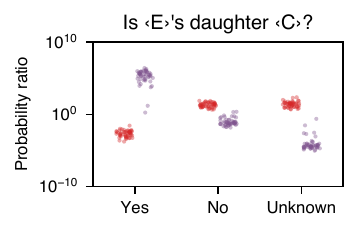}}
        {\includegraphics[width=\linewidth]{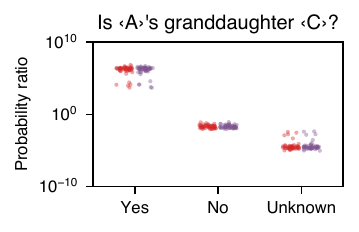}}
        {\includegraphics[width=\linewidth]{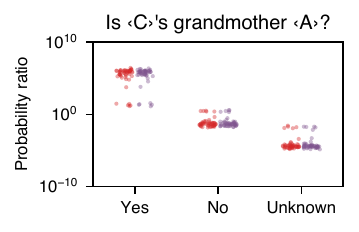}}
        {\includegraphics[width=0.28\textwidth]{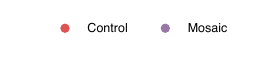}}
    \caption{
        \textbf{Identity--structure separability: Qwen-3-32B.}
        Results are shown for the ``family-trees'' setting.
        The control context is ``‹A› has daughter ‹B›. ‹B› has daughter ‹C›'';
        the donor context is ``‹D› has daughter ‹E›. ‹E› has daughter ‹F›''.
        The mosaic was constructed as in main-text Fig.~\figref{fig:separability}.
    }
    \label{SI-fig:model-generalization-separability-qwen-32b}
\end{figure*}
