# Supplementary material for: Cognitive Maps in Large Language Models
Source: arXiv:2610.25596 source file (2026-11-06)
Supplement: Supplementary file 17 [file additivity.tex]

\clearpage

\subsection{Additivity of representations of identity and structure across tasks}

\begin{figure*}[!htbp]
    \centering
    \fourpanelrowwithlegend
        {\includegraphics[width=\linewidth]{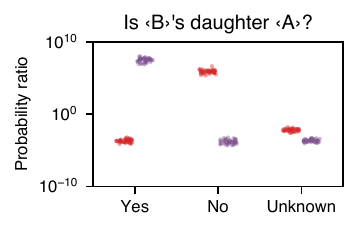}}
        {\includegraphics[width=\linewidth]{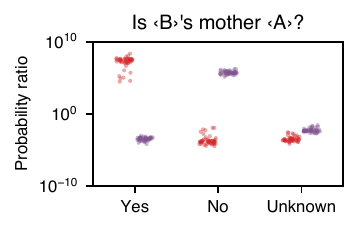}}
        {\includegraphics[width=\linewidth]{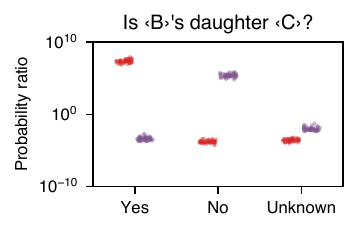}}
        {\includegraphics[width=\linewidth]{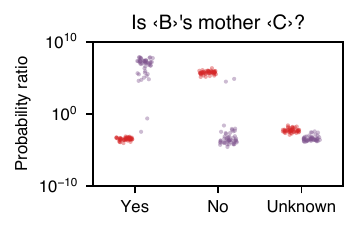}}
        {\includegraphics[width=0.28\textwidth]{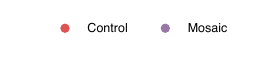}}
    \caption{
        \textbf{Additivity: family trees.}
        Results are shown for Gemma-3-27B.
        The control context is ``‹A› has daughter ‹B›. ‹B› has daughter ‹C›'';
        the donor contexts are ``‹D› has daughter ‹E›. ‹E› has daughter ‹F›''
        and ``‹F› has daughter ‹E›. ‹E› has daughter ‹D›''.
        The mosaic was constructed as in main-text Fig.~\figref{fig:additivity}.
    }
    \label{SI-fig:additivity-gemma27b-family-tree-yes-no}
\end{figure*}

\begin{figure*}[!htbp]
    \centering
    \fourpanelrowwithlegend
        {\includegraphics[width=\linewidth]{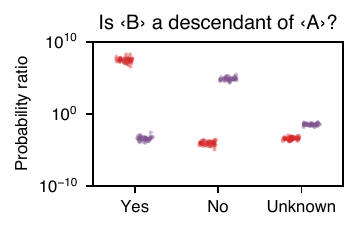}}
        {\includegraphics[width=\linewidth]{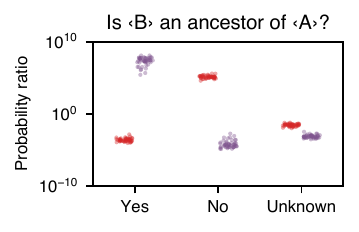}}
        {\includegraphics[width=\linewidth]{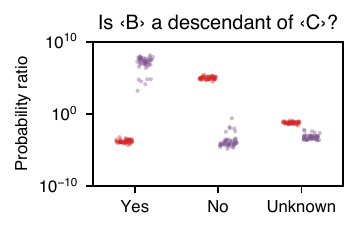}}
        {\includegraphics[width=\linewidth]{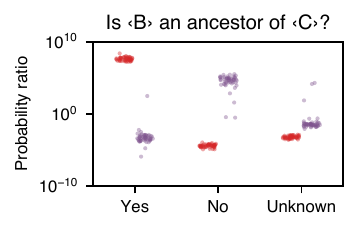}}
        {\includegraphics[width=0.28\textwidth]{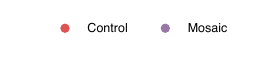}}
    \caption{
        \textbf{Additivity: ancestor--descendant relationships.}
        Results are shown for Gemma-3-27B.
        The control context is ``‹A› has daughter ‹B›. ‹B› has daughter ‹C›'';
        the donor contexts are ``‹D› has daughter ‹E›. ‹E› has daughter ‹F›''
        and ``‹F› has daughter ‹E›. ‹E› has daughter ‹D›''.
        The mosaic was constructed as in main-text Fig.~\figref{fig:additivity}.
    }
    \label{SI-fig:additivity-gemma27b-family-trees-descendant-ancestor}
\end{figure*}

\begin{figure*}[!htbp]
    \centering
    \fourpanelrowwithlegend
        {\includegraphics[width=\linewidth]{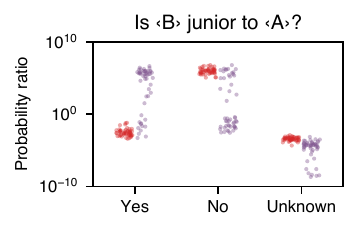}}
        {\includegraphics[width=\linewidth]{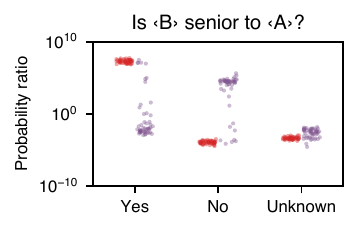}}
        {\includegraphics[width=\linewidth]{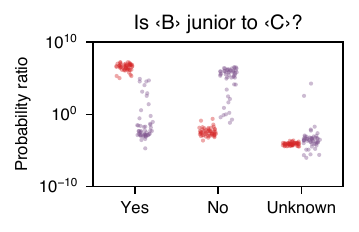}}
        {\includegraphics[width=\linewidth]{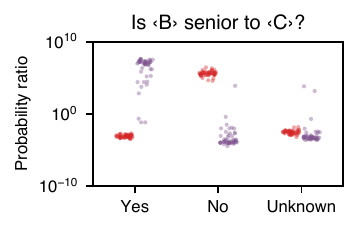}}
        {\includegraphics[width=0.28\textwidth]{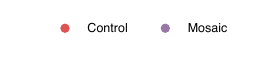}}
    \caption{
        \textbf{Additivity: company hierarchies.}
        Results are shown for Gemma-3-27B.
        The control context is ``‹A›'s boss is ‹B›. ‹B›'s boss is ‹C›'';
        the donor contexts are ``‹D›'s boss is ‹E›. ‹E›'s boss is ‹F›''
        and ``‹F›'s boss is ‹E›. ‹E›'s boss is ‹D›''.
        The mosaic was constructed as in main-text Fig.~\figref{fig:additivity}.
    }
    \label{SI-fig:additivity-gemma27b-company-structure}
\end{figure*}

\begin{figure*}[!htbp]
    \centering
    \fourpanelrowwithlegend
        {\includegraphics[width=\linewidth]{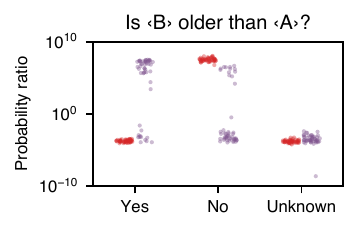}}
        {\includegraphics[width=\linewidth]{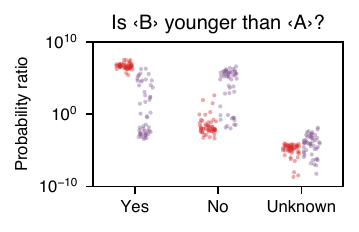}}
        {\includegraphics[width=\linewidth]{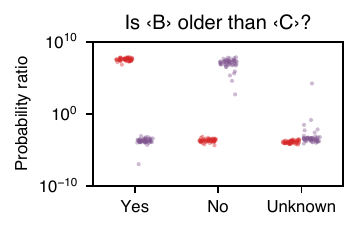}}
        {\includegraphics[width=\linewidth]{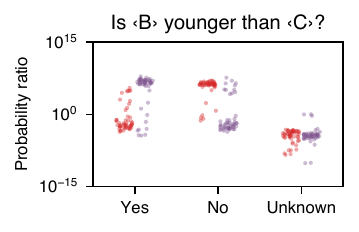}}
        {\includegraphics[width=0.28\textwidth]{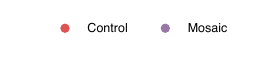}}
    \caption{
        \textbf{Additivity: age comparisons.}
        Results are shown for Gemma-3-27B.
        The control context is ``‹A› is older than ‹B›. ‹B› is older than ‹C›'';
        the donor contexts are ``‹D› is older than ‹E›. ‹E› is older than ‹F›''
        and ``‹F› is older than ‹E›. ‹E› is older than ‹D›''.
        The mosaic was constructed as in main-text Fig.~\figref{fig:additivity}.
    }
    \label{SI-fig:additivity-gemma27b-older-younger}
\end{figure*}

\begin{figure*}[!htbp]
    \centering
    \fourpanelrowwithlegend
        {\includegraphics[width=\linewidth]{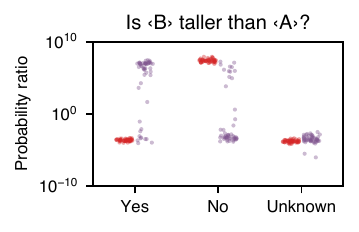}}
        {\includegraphics[width=\linewidth]{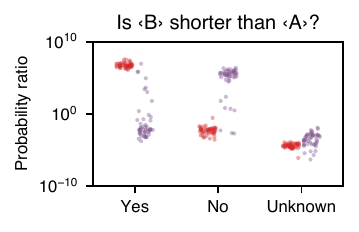}}
        {\includegraphics[width=\linewidth]{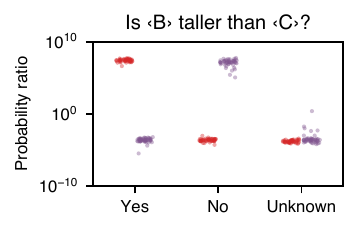}}
        {\includegraphics[width=\linewidth]{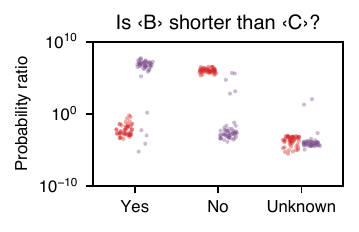}}
        {\includegraphics[width=0.28\textwidth]{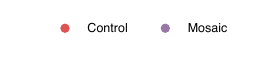}}
    \caption{
        \textbf{Additivity: height comparisons.}
        Results are shown for Gemma-3-27B.
        The control context is ``‹A› is taller than ‹B›. ‹B› is taller than ‹C›'';
        the donor contexts are ``‹D› is taller than ‹E›. ‹E› is taller than ‹F›''
        and ``‹F› is taller than ‹E›. ‹E› is taller than ‹D›''.
        The mosaic was constructed as in main-text Fig.~\figref{fig:additivity}.
    }
    \label{SI-fig:additivity-gemma27b-taller-shorter}
\end{figure*}

\begin{figure*}[!htbp]
    \centering
    \fourpanelrowwithlegend
        {\includegraphics[width=\linewidth]{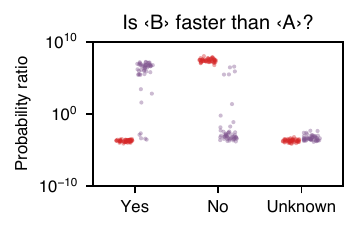}}
        {\includegraphics[width=\linewidth]{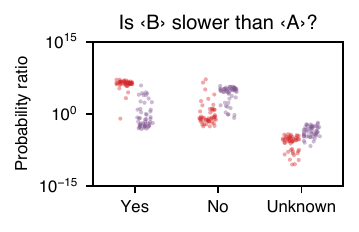}}
        {\includegraphics[width=\linewidth]{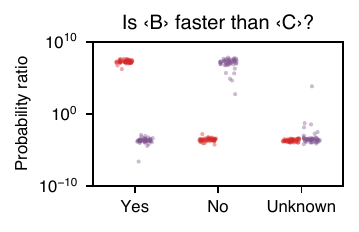}}
        {\includegraphics[width=\linewidth]{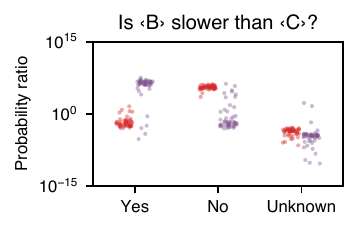}}
        {\includegraphics[width=0.28\textwidth]{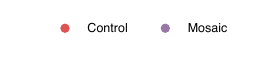}}
    \caption{
        \textbf{Additivity: speed comparisons.}
        Results are shown for Gemma-3-27B.
        The control context is ``‹A› is faster than ‹B›. ‹B› is faster than ‹C›'';
        the donor contexts are ``‹D› is faster than ‹E›. ‹E› is faster than ‹F›''
        and ``‹F› is faster than ‹E›. ‹E› is faster than ‹D›''.
        The mosaic was constructed as in main-text Fig.~\figref{fig:additivity}.
    }
    \label{SI-fig:additivity-gemma27b-faster-slower}
\end{figure*}

\begin{figure*}[!htbp]
    \centering
    \fourpanelrowwithlegend
        {\includegraphics[width=\linewidth]{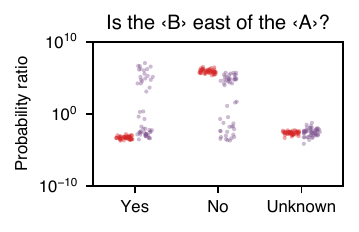}}
        {\includegraphics[width=\linewidth]{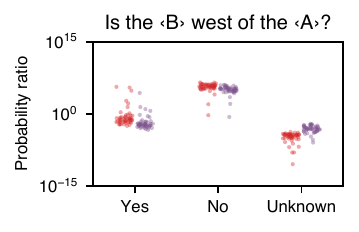}}
        {\includegraphics[width=\linewidth]{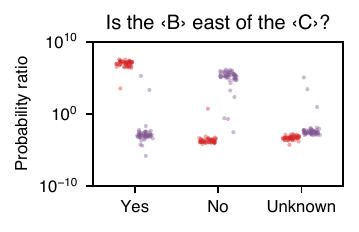}}
        {\includegraphics[width=\linewidth]{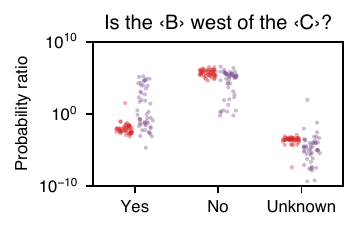}}
        {\includegraphics[width=0.28\textwidth]{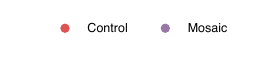}}
    \caption{
        \textbf{Additivity: east--west relationships.}
        Results are shown for Gemma-3-27B.
        The control context is ``The ‹A› is east of the ‹B›. The ‹B› is east of the ‹C›'';
        the donor contexts are ``The ‹D› is east of the ‹E›. The ‹E› is east of the ‹F›''
        and ``The ‹F› is east of the ‹E›. The ‹E› is east of the ‹D›''.
        The mosaic was constructed as in main-text Fig.~\figref{fig:additivity}.
    }
    \label{SI-fig:additivity-gemma27b-east-west}
\end{figure*}

\begin{figure*}[!htbp]
    \centering
    \fourpanelrowwithlegend
        {\includegraphics[width=\linewidth]{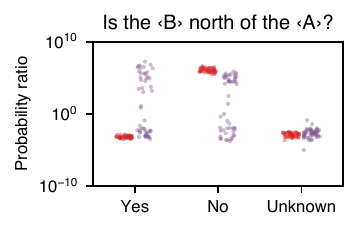}}
        {\includegraphics[width=\linewidth]{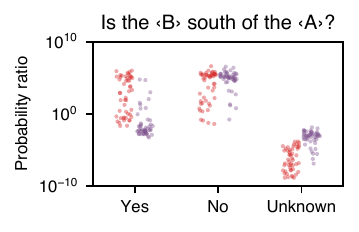}}
        {\includegraphics[width=\linewidth]{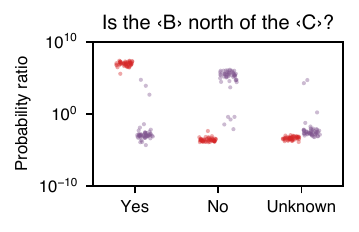}}
        {\includegraphics[width=\linewidth]{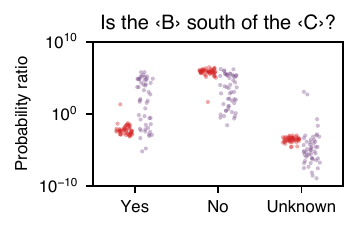}}
        {\includegraphics[width=0.28\textwidth]{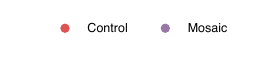}}
    \caption{
        \textbf{Additivity: north--south relationships.}
        Results are shown for Gemma-3-27B.
        The control context is ``The ‹A› is north of the ‹B›. The ‹B› is north of the ‹C›'';
        the donor contexts are ``The ‹D› is north of the ‹E›. The ‹E› is north of the ‹F›''
        and ``The ‹F› is north of the ‹E›. The ‹E› is north of the ‹D›''.
        The mosaic was constructed as in main-text Fig.~\figref{fig:additivity}.
    }
    \label{SI-fig:additivity-gemma27b-north-south}
\end{figure*}

\begin{figure*}[!htbp]
    \centering
    \fourpanelrowwithlegend
        {\includegraphics[width=\linewidth]{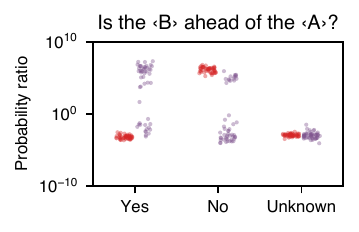}}
        {\includegraphics[width=\linewidth]{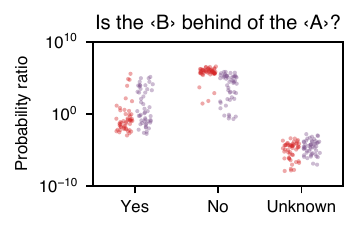}}
        {\includegraphics[width=\linewidth]{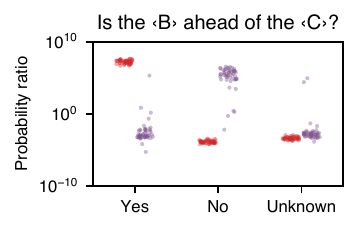}}
        {\includegraphics[width=\linewidth]{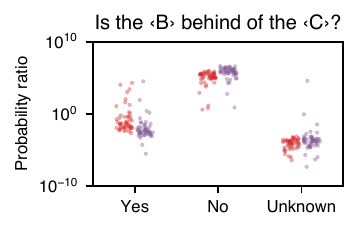}}
        {\includegraphics[width=0.28\textwidth]{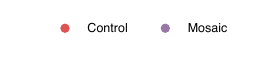}}
    \caption{
        \textbf{Additivity: ahead--behind relationships.}
        Results are shown for Gemma-3-27B.
        The control context is ``The ‹A› is ahead of the ‹B›. The ‹B› is ahead of the ‹C›'';
        the donor contexts are ``The ‹D› is ahead of the ‹E›. The ‹E› is ahead of the ‹F›''
        and ``The ‹F› is ahead of the ‹E›. The ‹E› is ahead of the ‹D›''.
        The mosaic was constructed as in main-text Fig.~\figref{fig:additivity}.
        The wording ``behind of'' is a grammatical error in the prompt template; the intended wording is ``behind''. It is retained here to match the prompts presented to the model.
    }
    \label{SI-fig:additivity-gemma27b-ahead-behind}
\end{figure*}

\begin{figure*}[!htbp]
    \centering
    \fourpanelrowwithlegend
        {\includegraphics[width=\linewidth]{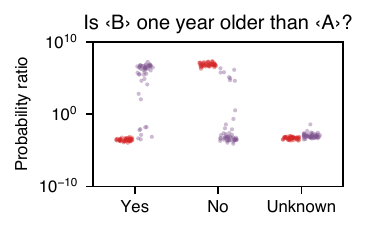}}
        {\includegraphics[width=\linewidth]{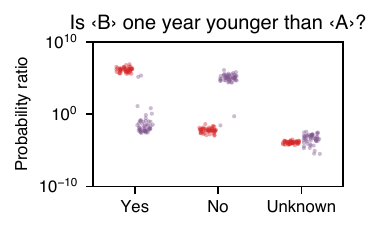}}
        {\includegraphics[width=\linewidth]{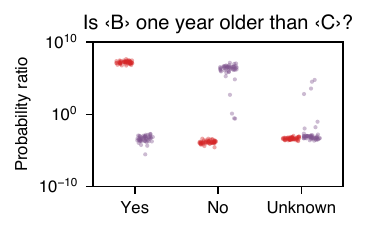}}
        {\includegraphics[width=\linewidth]{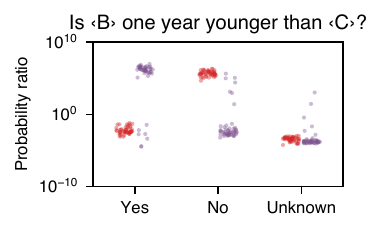}}
        {\includegraphics[width=0.28\textwidth]{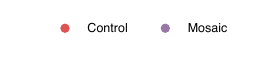}}
    \caption{
        \textbf{Additivity: exact age differences.}
        Results are shown for Gemma-3-27B.
        The control context is ``‹A› is one year older than ‹B›. ‹B› is one year older than ‹C›'';
        the donor contexts are ``‹D› is one year older than ‹E›. ‹E› is one year older than ‹F›''
        and ``‹F› is one year older than ‹E›. ‹E› is one year older than ‹D›''.
        The mosaic was constructed as in main-text Fig.~\figref{fig:additivity}.
    }
    \label{SI-fig:additivity-gemma27b-older-younger-unique-locations-yes-no}
\end{figure*}

\begin{figure*}[!htbp]
    \centering
    \fourpanelrowwithlegend
        {\includegraphics[width=\linewidth]{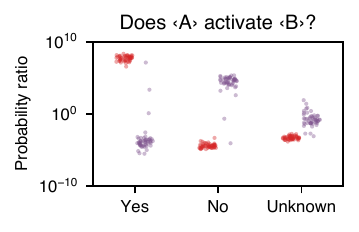}}
        {\includegraphics[width=\linewidth]{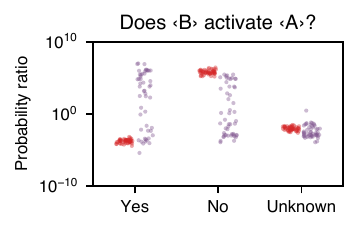}}
        {\includegraphics[width=\linewidth]{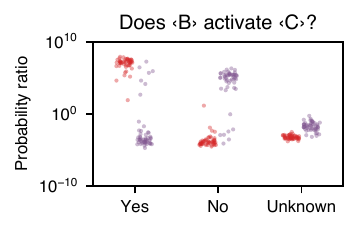}}
        {\includegraphics[width=\linewidth]{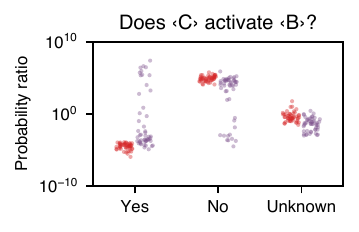}}
        {\includegraphics[width=0.28\textwidth]{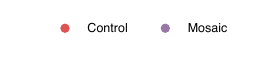}}
    \caption{
        \textbf{Additivity: gene regulatory networks.}
        Results are shown for Gemma-3-27B.
        The control context is ``‹A› activates ‹B›. ‹B› activates ‹C›'';
        the donor contexts are ``‹D› activates ‹E›. ‹E› activates ‹F›''
        and ``‹F› activates ‹E›. ‹E› activates ‹D›''.
        The mosaic was constructed as in main-text Fig.~\figref{fig:additivity}.
    }
    \label{SI-fig:additivity-gemma27b-gene-regulatory-network}
\end{figure*}

\begin{figure*}[!htbp]
    \centering
    \fourpanelrowwithlegend
        {\includegraphics[width=\linewidth]{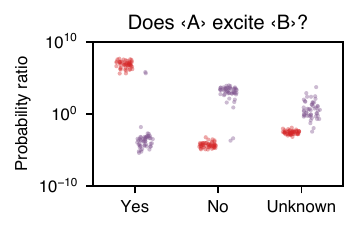}}
        {\includegraphics[width=\linewidth]{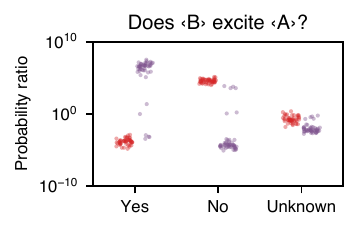}}
        {\includegraphics[width=\linewidth]{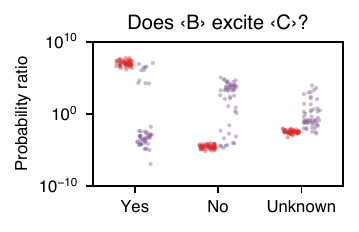}}
        {\includegraphics[width=\linewidth]{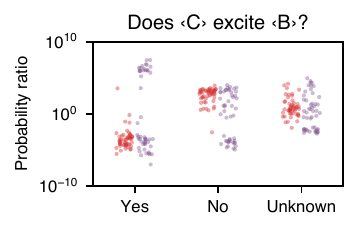}}
        {\includegraphics[width=0.28\textwidth]{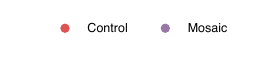}}
    \caption{
        \textbf{Additivity: neural circuits.}
        Results are shown for Gemma-3-27B.
        The control context is ``‹A› makes glutamatergic projections to ‹B›. ‹B› makes glutamatergic projections to ‹C›'';
        the donor contexts are ``‹D› makes glutamatergic projections to ‹E›. ‹E› makes glutamatergic projections to ‹F›''
        and ``‹F› makes glutamatergic projections to ‹E›. ‹E› makes glutamatergic projections to ‹D›''.
        The mosaic was constructed as in main-text Fig.~\figref{fig:additivity}.
    }
    \label{SI-fig:additivity-gemma27b-neural-circuit}
\end{figure*}

\begin{figure*}[!htbp]
    \centering
    \twopanelrow
        {\includegraphics[width=\linewidth]{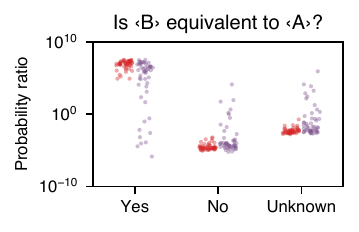}}
        {\includegraphics[width=\linewidth]{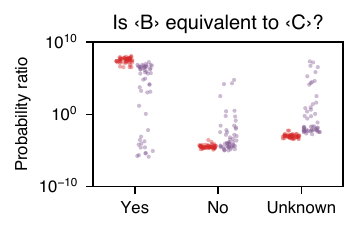}}
        {\includegraphics[width=0.28\textwidth]{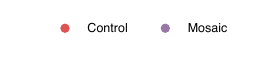}}
    \caption{\textbf{Additivity: propositional equivalence.}
        Results are shown for Gemma-3-27B.
        The control context is ``‹A› is equivalent to ‹B›. ‹B› is equivalent to ‹C›'';
        the donor contexts are ``‹D› is equivalent to ‹E›. ‹E› is equivalent to ‹F›''
        and ``‹F› is equivalent to ‹E›. ‹E› is equivalent to ‹D›''.
        The mosaic was constructed as in main-text Fig.~\figref{fig:additivity}. Because exchanging entities ``‹A›'' and ``‹C›'' leaves the equivalence relationships unchanged, these panels cannot distinguish whether the two entities have swapped roles. We nevertheless include them for completeness.
    }
    \label{SI-fig:additivity-gemma27b-proposition-equivalence}
\end{figure*}

\begin{figure*}[!htbp]
    \centering
    \twopanelrow
        {\includegraphics[width=\linewidth]{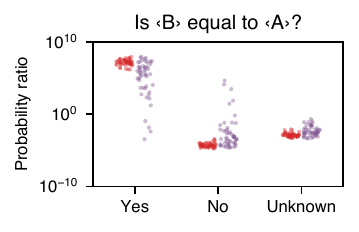}}
        {\includegraphics[width=\linewidth]{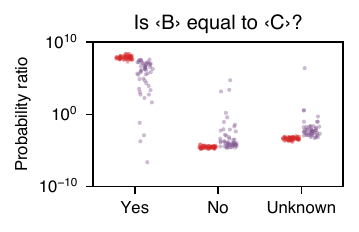}}
        {\includegraphics[width=0.28\textwidth]{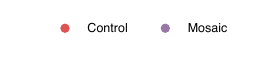}}
    \caption{\textbf{Additivity: variable equality.}
        Results are shown for Gemma-3-27B.
        The control context is ``‹A› is equal to ‹B›. ‹B› is equal to ‹C›'';
        the donor contexts are ``‹D› is equal to ‹E›. ‹E› is equal to ‹F›''
        and ``‹F› is equal to ‹E›. ‹E› is equal to ‹D›''.
        The mosaic was constructed as in main-text Fig.~\figref{fig:additivity}. Because exchanging entities ``‹A›'' and ``‹C›'' leaves the equivalence relationships unchanged, these panels cannot distinguish whether the two entities have swapped roles. We nevertheless include them for completeness.
    }
    \label{SI-fig:additivity-gemma27b-variable-equivalence}
\end{figure*}
