# Supplementary material for: Cognitive Maps in Large Language Models
Source: arXiv:2610.25596 source file (2026-11-06)
Supplement: Supplementary file 18 [file behavior.tex]

\subsection{Behavior and generalization across tasks}

\begin{figure*}[!htbp]
    \centering
    \behaviorpanelswithlegend
        {\includegraphics[width=\linewidth]{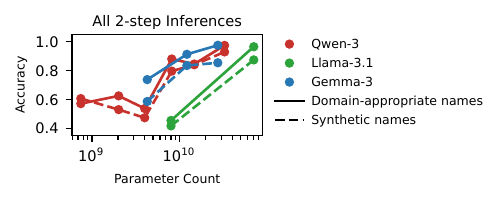}}
        {\includegraphics[width=0.27\textwidth]{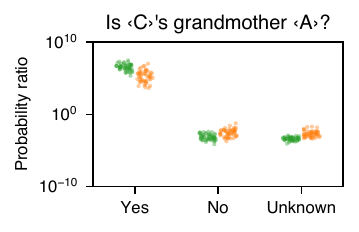}}
        {\includegraphics[width=0.18\textwidth]{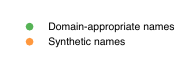}}
    \caption{
        \textbf{Behavior and generalization: family trees.}
        \textbf{A}, Accuracy on a selected set of two-hop queries
        plotted against model parameter count for all models studied.
        \textbf{B}, Gemma-3-27B responses to the indicated query.
        The context is ``‹A› has daughter ‹B›. ‹B› has daughter ‹C›''.
        Responses are shown for both domain-appropriate (green) and
        synthetic (orange) names.
    }
    \label{SI-fig:behavior-family-tree-yes-no}
\end{figure*}

\begin{figure*}[!htbp]
    \centering
    \behaviorpanelswithlegend
        {\includegraphics[width=\linewidth]{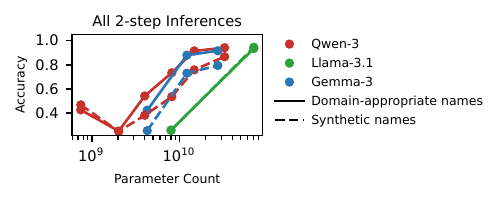}}
        {\includegraphics[width=0.27\textwidth]{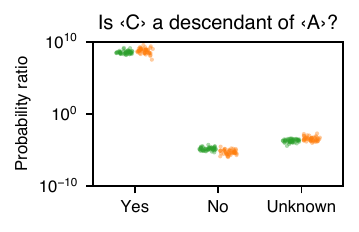}}
        {\includegraphics[width=0.18\textwidth]{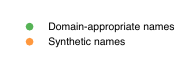}}
    \caption{
        \textbf{Behavior and generalization: ancestor--descendant relationships.}
        \textbf{A}, Accuracy on a selected set of two-hop queries
        plotted against model parameter count for all models studied.
        \textbf{B}, Gemma-3-27B responses to the indicated query.
        The context is ``‹A› has daughter ‹B›. ‹B› has daughter ‹C›''.
        Responses are shown for both domain-appropriate (green) and synthetic (orange) names.
    }
    \label{SI-fig:behavior-family-trees-descendant-ancestor}
\end{figure*}

\begin{figure*}[!htbp]
    \centering
    \behaviorpanelswithlegend
        {\includegraphics[width=\linewidth]{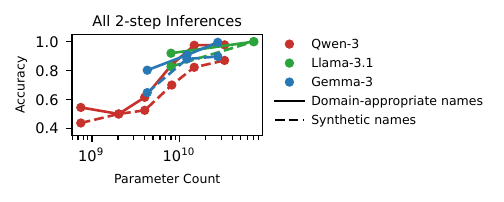}}
        {\includegraphics[width=0.27\textwidth]{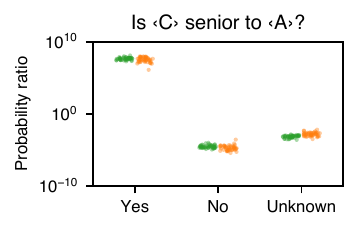}}
        {\includegraphics[width=0.18\textwidth]{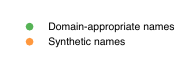}}
    \caption{
        \textbf{Behavior and generalization: company hierarchies.}
        \textbf{A}, Accuracy on a selected set of two-hop queries
        plotted against model parameter count for all models studied.
        \textbf{B}, Gemma-3-27B responses to the indicated query.
        The context is ``‹A›'s boss is ‹B›. ‹B›'s boss is ‹C›''.
        Responses are shown for both domain-appropriate (green) and synthetic (orange) names.
    }
    \label{SI-fig:behavior-company-structure}
\end{figure*}

\begin{figure*}[!htbp]
    \centering
    \behaviorpanelswithlegend
        {\includegraphics[width=\linewidth]{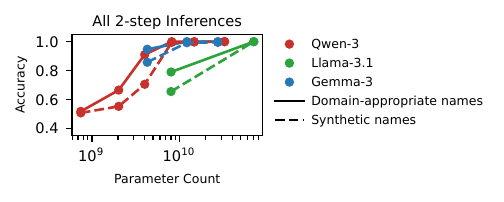}}
        {\includegraphics[width=0.27\textwidth]{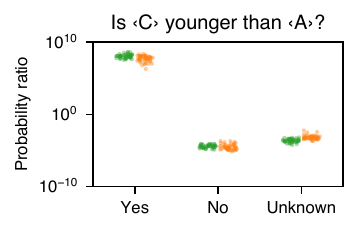}}
        {\includegraphics[width=0.18\textwidth]{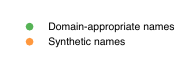}}
    \caption{
        \textbf{Behavior and generalization: age comparisons.}
        \textbf{A}, Accuracy on a selected set of two-hop queries
        plotted against model parameter count for all models studied.
        \textbf{B}, Gemma-3-27B responses to the indicated query.
        The context is ``‹A› is older than ‹B›. ‹B› is older than ‹C›''.
        Responses are shown for both domain-appropriate (green) and synthetic (orange) names.
    }
    \label{SI-fig:behavior-older-younger}
\end{figure*}

\begin{figure*}[!htbp]
    \centering
    \behaviorpanelswithlegend
        {\includegraphics[width=\linewidth]{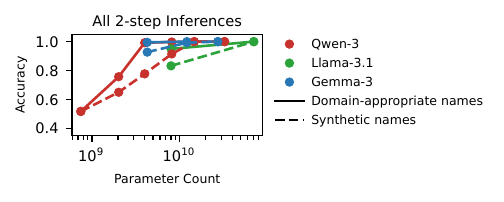}}
        {\includegraphics[width=0.27\textwidth]{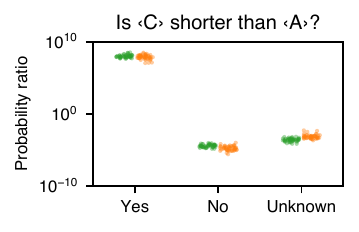}}
        {\includegraphics[width=0.18\textwidth]{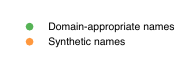}}
    \caption{
        \textbf{Behavior and generalization: height comparisons.}
        \textbf{A}, Accuracy on a selected set of two-hop queries
        plotted against model parameter count for all models studied.
        \textbf{B}, Gemma-3-27B responses to the indicated query.
        The context is ``‹A› is taller than ‹B›. ‹B› is taller than ‹C›''.
        Responses are shown for both domain-appropriate (green) and synthetic (orange) names.
    }
    \label{SI-fig:behavior-taller-shorter}
\end{figure*}

\begin{figure*}[!htbp]
    \centering
    \behaviorpanelswithlegend
        {\includegraphics[width=\linewidth]{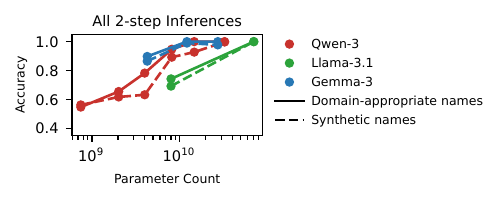}}
        {\includegraphics[width=0.27\textwidth]{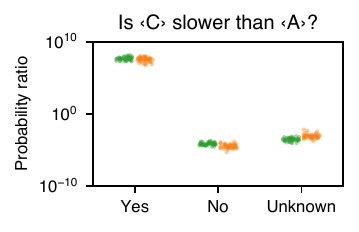}}
        {\includegraphics[width=0.18\textwidth]{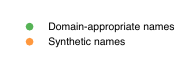}}
    \caption{
        \textbf{Behavior and generalization: speed comparisons.}
        \textbf{A}, Accuracy on a selected set of two-hop queries
        plotted against model parameter count for all models studied.
        \textbf{B}, Gemma-3-27B responses to the indicated query.
        The context is ``‹A› is faster than ‹B›. ‹B› is faster than ‹C›''.
        Responses are shown for both domain-appropriate (green) and synthetic (orange) names.
    }
    \label{SI-fig:behavior-faster-slower}
\end{figure*}

\begin{figure*}[!htbp]
    \centering
    \behaviorpanelswithlegend
        {\includegraphics[width=\linewidth]{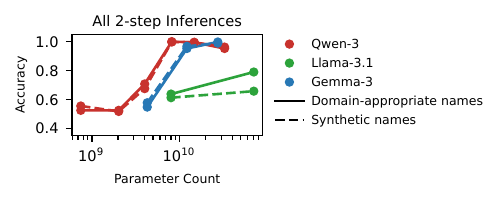}}
        {\includegraphics[width=0.27\textwidth]{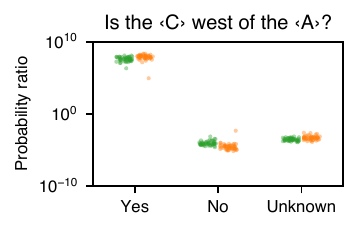}}
        {\includegraphics[width=0.18\textwidth]{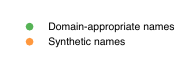}}
    \caption{
        \textbf{Behavior and generalization: east--west relationships.}
        \textbf{A}, Accuracy on a selected set of two-hop queries
        plotted against model parameter count for all models studied.
        \textbf{B}, Gemma-3-27B responses to the indicated query.
        The context is ``The ‹A› is east of the ‹B›. The ‹B› is east of the ‹C›''.
        Responses are shown for both domain-appropriate (green) and synthetic (orange) names.
    }
    \label{SI-fig:behavior-east-west}
\end{figure*}

\begin{figure*}[!htbp]
    \centering
    \behaviorpanelswithlegend
        {\includegraphics[width=\linewidth]{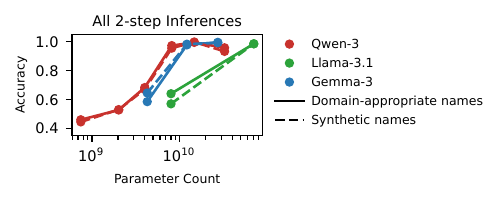}}
        {\includegraphics[width=0.27\textwidth]{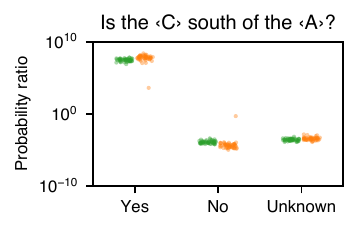}}
        {\includegraphics[width=0.18\textwidth]{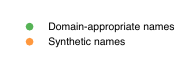}}
    \caption{
        \textbf{Behavior and generalization: north--south relationships.}
        \textbf{A}, Accuracy on a selected set of two-hop queries
        plotted against model parameter count for all models studied.
        \textbf{B}, Gemma-3-27B responses to the indicated query.
        The context is ``The ‹A› is north of the ‹B›. The ‹B› is north of the ‹C›''.
        Responses are shown for both domain-appropriate (green) and synthetic (orange) names.
    }
    \label{SI-fig:behavior-north-south}
\end{figure*}

\begin{figure*}[!htbp]
    \centering
    \behaviorpanelswithlegend
        {\includegraphics[width=\linewidth]{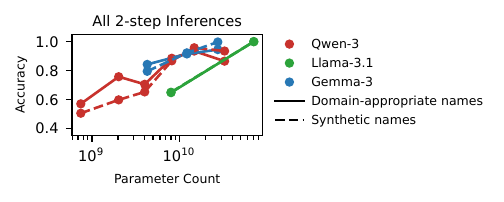}}
        {\includegraphics[width=0.27\textwidth]{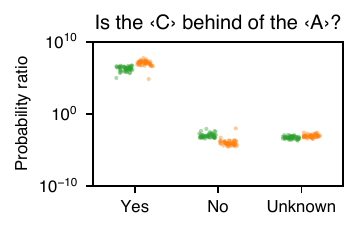}}
        {\includegraphics[width=0.18\textwidth]{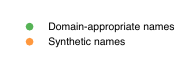}}
    \caption{
        \textbf{Behavior and generalization: ahead--behind relationships.}
        \textbf{A}, Accuracy on a selected set of two-hop queries
        plotted against model parameter count for all models studied.
        \textbf{B}, Gemma-3-27B responses to the indicated query.
        The context is ``The ‹A› is ahead of the ‹B›. The ‹B› is ahead of the ‹C›''.
        The wording ``behind of'' is a grammatical error in the prompt template;
        the intended wording is ``behind''. It is retained here to match the prompts presented to the model.
        Responses are shown for both domain-appropriate (green) and synthetic (orange) names.
    }
    \label{SI-fig:behavior-ahead-behind}
\end{figure*}

\begin{figure*}[!htbp]
    \centering
    \behaviorpanelswithlegend
        {\includegraphics[width=\linewidth]{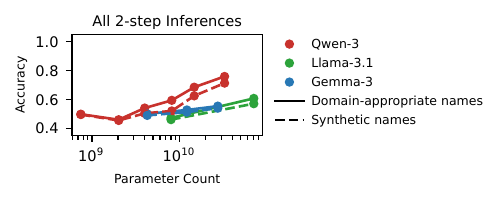}}
        {\includegraphics[width=0.27\textwidth]{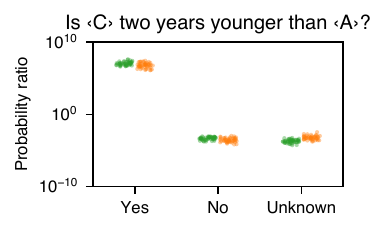}}
        {\includegraphics[width=0.18\textwidth]{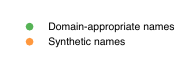}}
    \caption{
        \textbf{Behavior and generalization: exact age differences.}
        \textbf{A}, Accuracy on a selected set of two-hop queries
        plotted against model parameter count for all models studied.
        \textbf{B}, Gemma-3-27B responses to the indicated query.
        The context is ``‹A› is one year older than ‹B›. ‹B› is one year older than ‹C›''.
        Responses are shown for both domain-appropriate (green) and synthetic (orange) names.
    }
    \label{SI-fig:behavior-older-younger-unique-locations-yes-no}
\end{figure*}

\begin{figure*}[!htbp]
    \centering
    \behaviorpanels
        {\includegraphics[width=\linewidth]{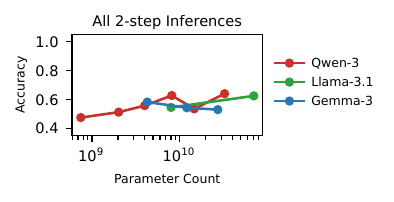}}
        {\includegraphics[width=\linewidth]{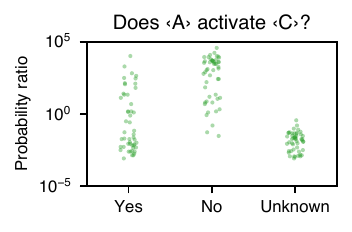}}
    \caption{
        \textbf{Behavior: gene regulatory networks.}
        \textbf{A}, Accuracy on a selected set of two-hop queries
        plotted against model parameter count for all models studied.
        \textbf{B}, Gemma-3-27B responses to the indicated query.
        The context is ``‹A› activates ‹B›. ‹B› activates ‹C›''. 
        For this setting, we did not compare domain-appropriate and synthetic names 
        because we used synthetic names for the names of genes.
    }
    \label{SI-fig:behavior-gene-regulatory-network}
\end{figure*}

\begin{figure*}[!htbp]
    \centering
    \behaviorpanels
        {\includegraphics[width=\linewidth]{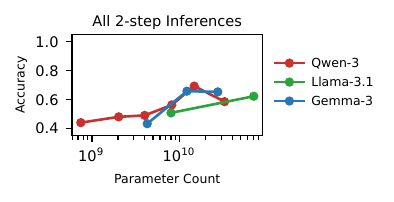}}
        {\includegraphics[width=\linewidth]{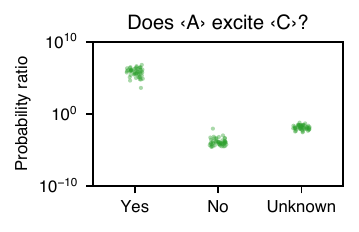}}
    \caption{
        \textbf{Behavior: neural circuits.}
        \textbf{A}, Accuracy on a selected set of two-hop queries
        plotted against model parameter count for all models studied.
        \textbf{B}, Gemma-3-27B responses to the indicated query.
        The context is ``‹A› makes glutamatergic projections to ‹B›. ‹B› makes glutamatergic projections to ‹C›''.
        For this setting, we did not compare domain-appropriate and synthetic names 
        because we used synthetic names for the names of neurons.
    }
    \label{SI-fig:behavior-neural-circuit}
\end{figure*}

\begin{figure*}[!htbp]
    \centering
    \behaviorpanelswithlegend
        {\includegraphics[width=\linewidth]{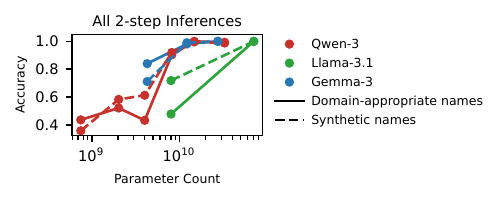}}
        {\includegraphics[width=0.27\textwidth]{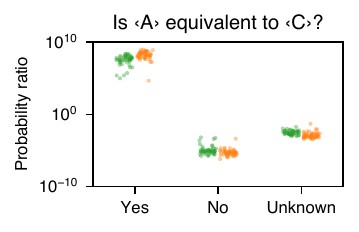}}
        {\includegraphics[width=0.18\textwidth]{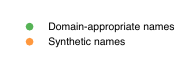}}
    \caption{
        \textbf{Behavior and generalization: propositional equivalence.}
        \textbf{A}, Accuracy on a selected set of two-hop queries
        plotted against model parameter count for all models studied.
        \textbf{B}, Gemma-3-27B responses to the indicated query.
        The context is ``‹A› is equivalent to ‹B›. ‹B› is equivalent to ‹C›''.
        Responses are shown for both domain-appropriate (green) and synthetic (orange) names.
    }
    \label{SI-fig:behavior-proposition-equivalence}
\end{figure*}

\begin{figure*}[!htbp]
    \centering
    \behaviorpanelswithlegend
        {\includegraphics[width=\linewidth]{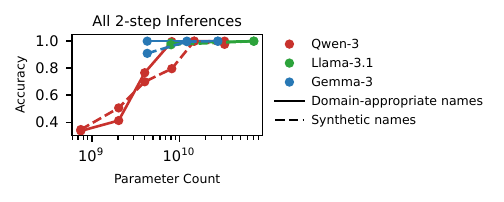}}
        {\includegraphics[width=0.27\textwidth]{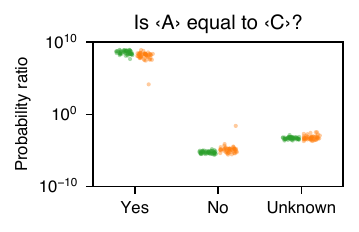}}
        {\includegraphics[width=0.18\textwidth]{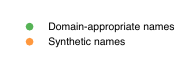}}
    \caption{
        \textbf{Behavior and generalization: variable equality.}
        \textbf{A}, Accuracy on a selected set of two-hop queries
        plotted against model parameter count for all models studied.
        \textbf{B}, Gemma-3-27B responses to the indicated query.
        The context is ``‹A› is equal to ‹B›. ‹B› is equal to ‹C›''.
        Responses are shown for both domain-appropriate (green) and synthetic (orange) names.
    }
    \label{SI-fig:behavior-variable-equivalence}
\end{figure*}
