# Supplementary material for: Cognitive Maps in Large Language Models
Source: arXiv:2610.25596 source file (2026-11-06)
Supplement: Supplementary file 19 [file erasure.tex]

\clearpage

\subsection{Key--value erasure and editing across tasks}

\begin{figure*}[!htbp]
    \centering
    \erasurepanels
        {\includegraphics[width=\linewidth]{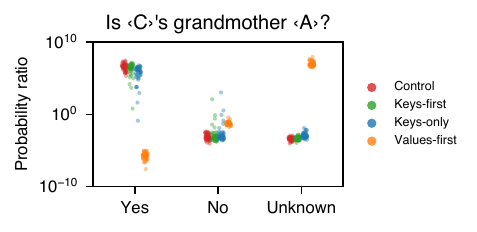}}
        {\includegraphics[width=\linewidth]{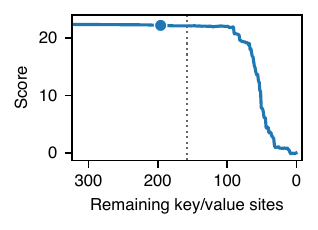}}
        {\includegraphics[width=\linewidth]{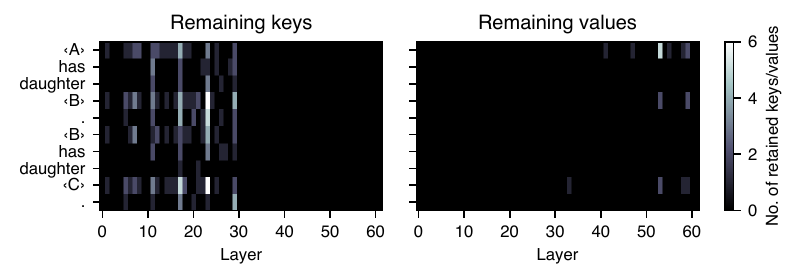}}
        {\includegraphics[width=\linewidth]{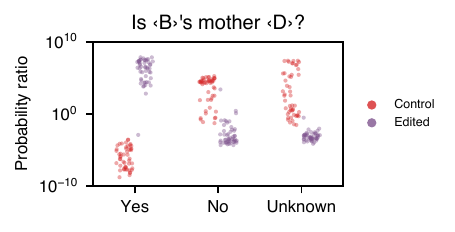}}
        {\includegraphics[width=\linewidth]{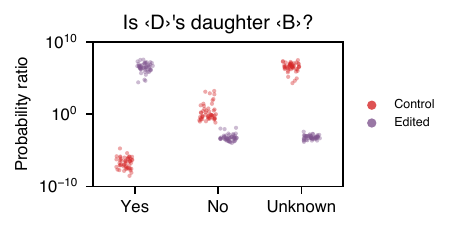}}
    \caption{\textbf{Key--value erasure and editing: family trees.}
        Results are shown for Gemma-3-27B. Procedures follow main-text Fig.~\figref{fig:binding}.
        The control context is ``‹A› has daughter ‹B›. ‹B› has daughter ‹C›'';
        the donor context is ``‹D› has daughter ‹E›. ‹E› has daughter ‹F›''.
        \textbf{A}, Responses for the keys-first, keys-only, and values-first memories.
        \textbf{B}, Final portion of the pruning trajectory.
        \textbf{C}, Distribution of the 176 keys and 20 values retained by this mask,
        together comprising 0.99\% of all key/value sites.
        \textbf{D, E}, Responses before and after replacing selected keys associated
        with the first entity in the control memory with the corresponding donor keys.
    }
    \label{SI-fig:erasure-family-tree-yes-no}
\end{figure*}

\begin{figure*}[!htbp]
    \centering
    \erasurepanels
        {\includegraphics[width=\linewidth]{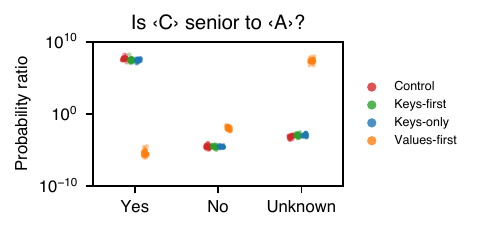}}
        {\includegraphics[width=\linewidth]{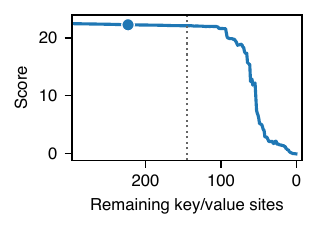}}
        {\includegraphics[width=\linewidth]{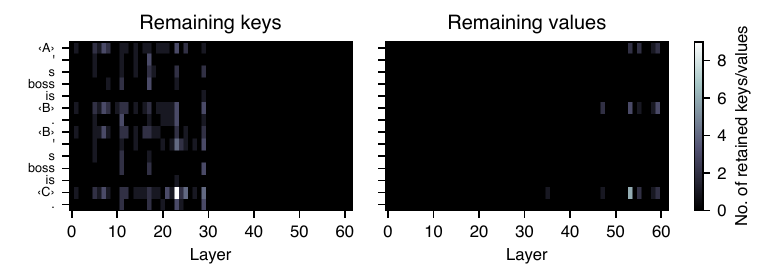}}
        {\includegraphics[width=\linewidth]{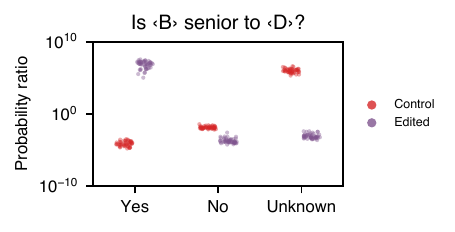}}
        {\includegraphics[width=\linewidth]{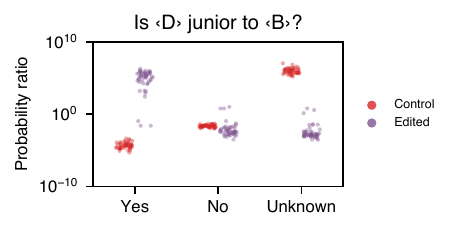}}
    \caption{\textbf{Key--value erasure and editing: company hierarchies.}
        Results are shown for Gemma-3-27B. Procedures follow main-text Fig.~\figref{fig:binding}.
        The control context is ``‹A›'s boss is ‹B›. ‹B›'s boss is ‹C›'';
        the donor context is ``‹D›'s boss is ‹E›. ‹E›'s boss is ‹F›''.
        \textbf{A}, Responses for the keys-first, keys-only, and values-first memories.
        \textbf{B}, Final portion of the pruning trajectory.
        \textbf{C}, Distribution of the 193 keys and 30 values retained by this mask,
        together comprising 0.80\% of all key/value sites.
        \textbf{D, E}, Responses before and after replacing selected keys associated
        with the first entity in the control memory with the corresponding donor keys.
    }
    \label{SI-fig:erasure-company-structure}
\end{figure*}

\begin{figure*}[!htbp]
    \centering
    \erasurepanels
        {\includegraphics[width=\linewidth]{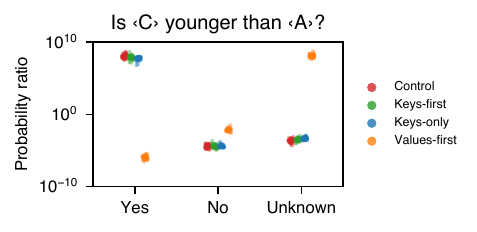}}
        {\includegraphics[width=\linewidth]{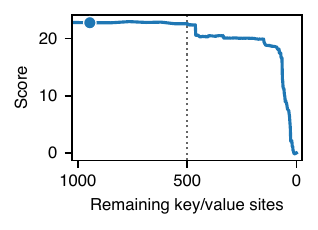}}
        {\includegraphics[width=\linewidth]{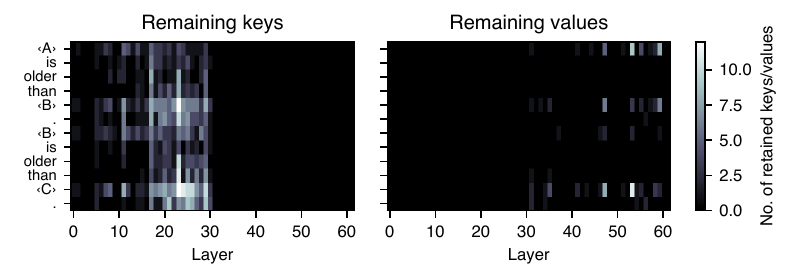}}
        {\includegraphics[width=\linewidth]{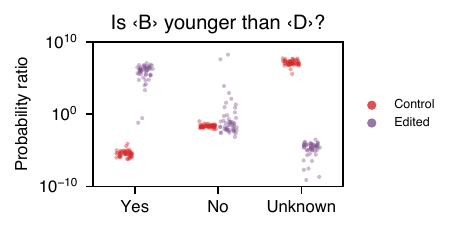}}
        {\includegraphics[width=\linewidth]{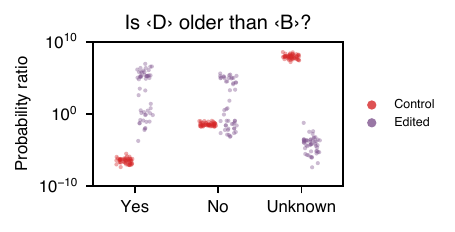}}
    \caption{\textbf{Key--value erasure and editing: age comparisons.}
        Results are shown for Gemma-3-27B. Procedures follow main-text Fig.~\figref{fig:binding}.
        The control context is ``‹A› is older than ‹B›. ‹B› is older than ‹C›'';
        the donor context is ``‹D› is older than ‹E›. ‹E› is older than ‹F›''.
        \textbf{A}, Responses for the keys-first, keys-only, and values-first memories.
        \textbf{B}, Final portion of the pruning trajectory.
        \textbf{C}, Distribution of the 833 keys and 112 values retained by this mask,
        together comprising 3.97\% of all key/value sites.
        \textbf{D, E}, Responses before and after replacing selected keys associated
        with the first entity in the control memory with the corresponding donor keys.
    }
    \label{SI-fig:erasure-older-younger}
\end{figure*}

\begin{figure*}[!htbp]
    \centering
    \erasurepanels
        {\includegraphics[width=\linewidth]{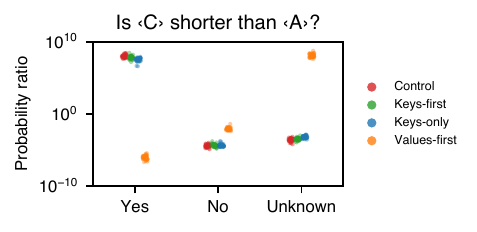}}
        {\includegraphics[width=\linewidth]{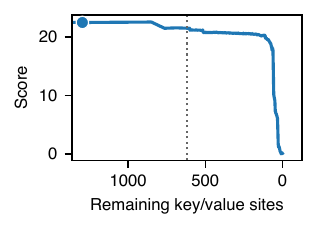}}
        {\includegraphics[width=\linewidth]{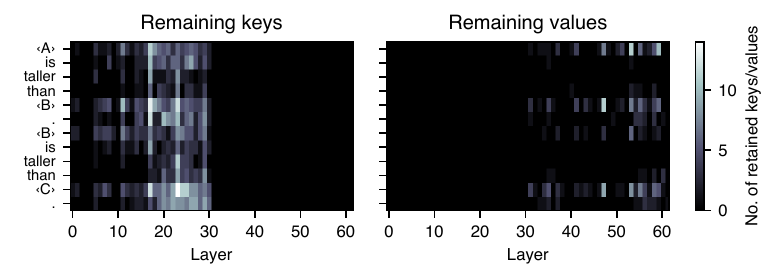}}
        {\includegraphics[width=\linewidth]{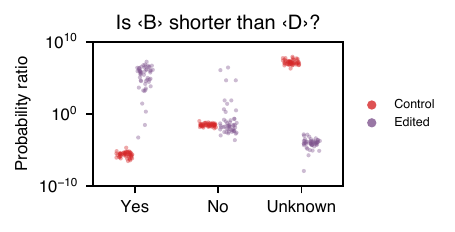}}
        {\includegraphics[width=\linewidth]{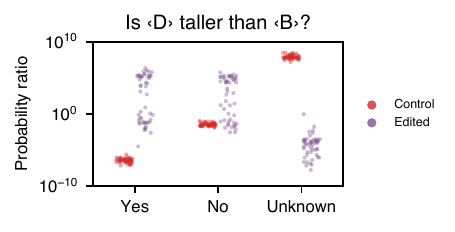}}
    \caption{\textbf{Key--value erasure and editing: height comparisons.}
        Results are shown for Gemma-3-27B. Procedures follow main-text Fig.~\figref{fig:binding}.
        The control context is ``‹A› is taller than ‹B›. ‹B› is taller than ‹C›'';
        the donor context is ``‹D› is taller than ‹E›. ‹E› is taller than ‹F›''.
        \textbf{A}, Responses for the keys-first, keys-only, and values-first memories.
        \textbf{B}, Final portion of the pruning trajectory.
        \textbf{C}, Distribution of the 1,034 keys and 263 values retained by this mask,
        together comprising 5.45\% of all key/value sites.
        \textbf{D, E}, Responses before and after replacing selected keys associated
        with the first entity in the control memory with the corresponding donor keys.
    }
    \label{SI-fig:erasure-taller-shorter}
\end{figure*}

\begin{figure*}[!htbp]
    \centering
    \erasurepanels
        {\includegraphics[width=\linewidth]{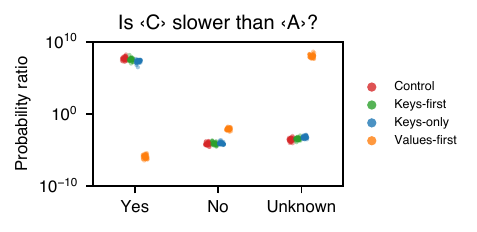}}
        {\includegraphics[width=\linewidth]{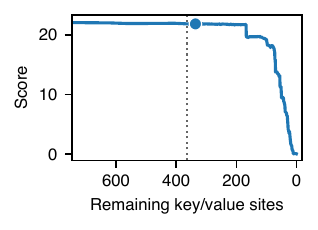}}
        {\includegraphics[width=\linewidth]{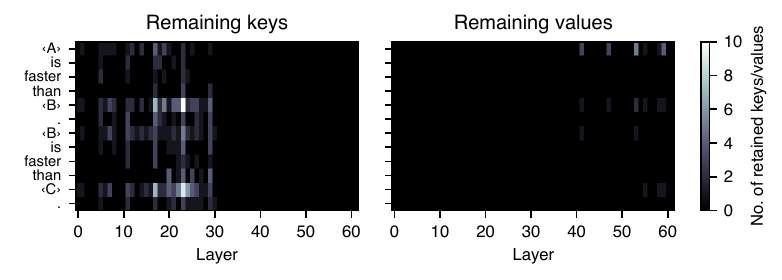}}
        {\includegraphics[width=\linewidth]{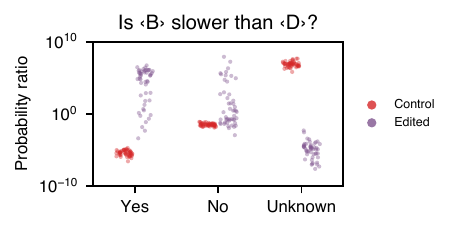}}
        {\includegraphics[width=\linewidth]{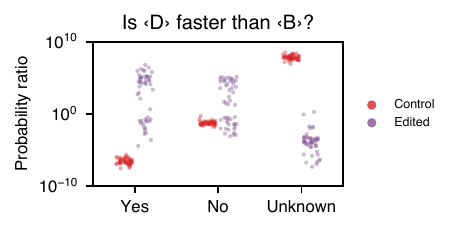}}
    \caption{\textbf{Key--value erasure and editing: speed comparisons.}
        Results are shown for Gemma-3-27B. Procedures follow main-text Fig.~\figref{fig:binding}.
        The control context is ``‹A› is faster than ‹B›. ‹B› is faster than ‹C›'';
        the donor context is ``‹D› is faster than ‹E›. ‹E› is faster than ‹F›''.
        \textbf{A}, Responses for the keys-first, keys-only, and values-first memories.
        \textbf{B}, Final portion of the pruning trajectory.
        \textbf{C}, Distribution of the 307 keys and 29 values retained by this mask,
        together comprising 1.41\% of all key/value sites.
        \textbf{D, E}, Responses before and after replacing selected keys associated
        with the first entity in the control memory with the corresponding donor keys.
    }
    \label{SI-fig:erasure-faster-slower}
\end{figure*}

\begin{figure*}[!htbp]
    \centering
    \erasurepanels
        {\includegraphics[width=\linewidth]{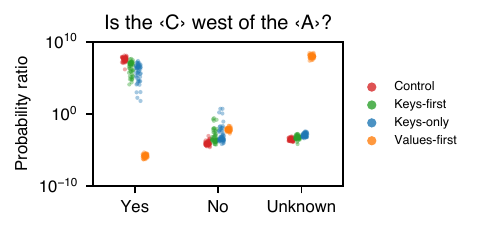}}
        {\includegraphics[width=\linewidth]{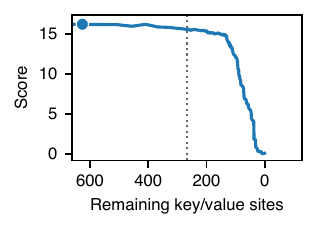}}
        {\includegraphics[width=\linewidth]{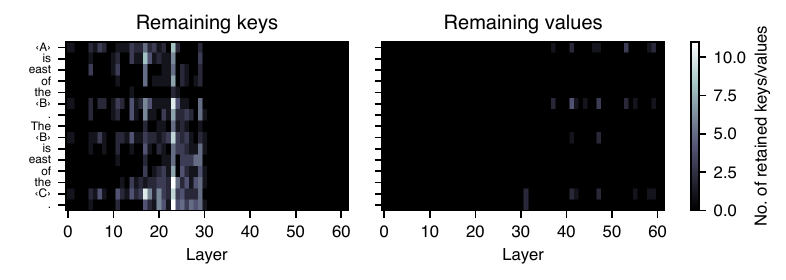}}
        {\includegraphics[width=\linewidth]{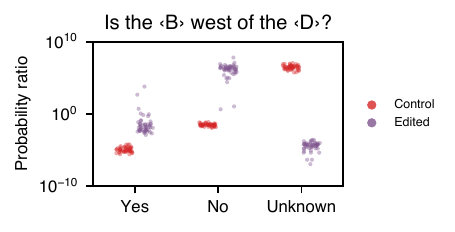}}
        {\includegraphics[width=\linewidth]{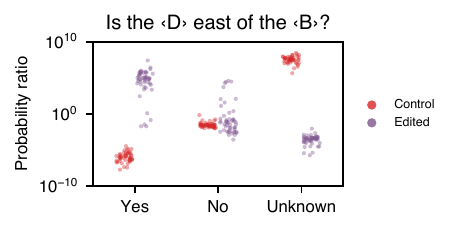}}
    \caption{\textbf{Key--value erasure and editing: east--west relationships.}
        Results are shown for Gemma-3-27B. Procedures follow main-text Fig.~\figref{fig:binding}.
        The control context is ``The ‹A› is east of the ‹B›. The ‹B› is east of the ‹C›'';
        the donor context is ``The ‹D› is east of the ‹E›. The ‹E› is east of the ‹F›''.
        \textbf{A}, Responses for the keys-first, keys-only, and values-first memories.
        \textbf{B}, Final portion of the pruning trajectory.
        \textbf{C}, Distribution of the 585 keys and 41 values retained by this mask,
        together comprising 2.10\% of all key/value sites.
        \textbf{D, E}, Responses before and after replacing selected keys associated
        with the first entity in the control memory with the corresponding donor keys.
    }
    \label{SI-fig:erasure-east-west}
\end{figure*}

\begin{figure*}[!htbp]
    \centering
    \erasurepanels
        {\includegraphics[width=\linewidth]{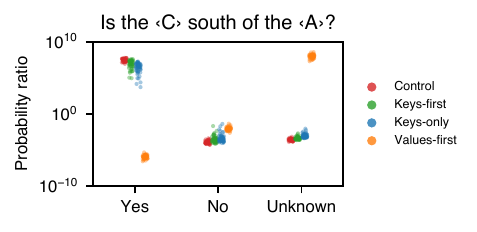}}
        {\includegraphics[width=\linewidth]{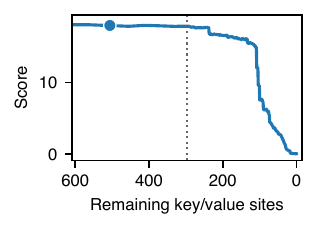}}
        {\includegraphics[width=\linewidth]{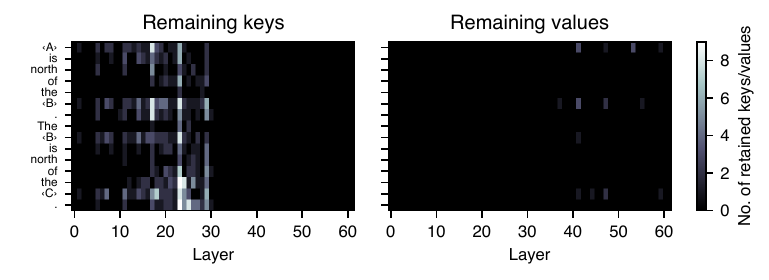}}
        {\includegraphics[width=\linewidth]{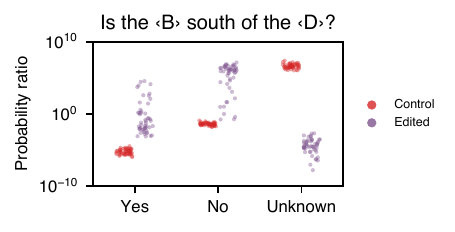}}
        {\includegraphics[width=\linewidth]{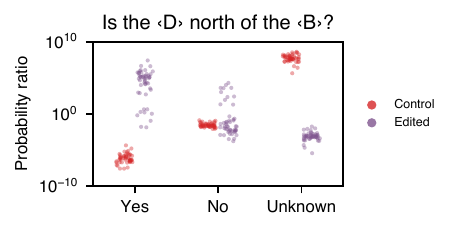}}
    \caption{\textbf{Key--value erasure and editing: north--south relationships.}
        Results are shown for Gemma-3-27B. Procedures follow main-text Fig.~\figref{fig:binding}.
        The control context is ``The ‹A› is north of the ‹B›. The ‹B› is north of the ‹C›'';
        the donor context is ``The ‹D› is north of the ‹E›. The ‹E› is north of the ‹F›''.
        \textbf{A}, Responses for the keys-first, keys-only, and values-first memories.
        \textbf{B}, Final portion of the pruning trajectory.
        \textbf{C}, Distribution of the 485 keys and 21 values retained by this mask,
        together comprising 1.70\% of all key/value sites.
        \textbf{D, E}, Responses before and after replacing selected keys associated
        with the first entity in the control memory with the corresponding donor keys.
    }
    \label{SI-fig:erasure-north-south}
\end{figure*}

\begin{figure*}[!htbp]
    \centering
    \erasurepanels
        {\includegraphics[width=\linewidth]{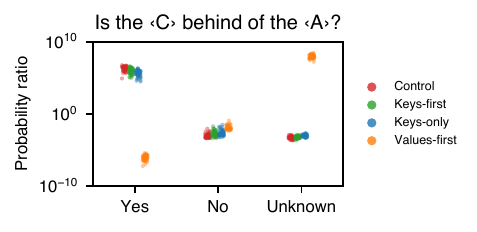}}
        {\includegraphics[width=\linewidth]{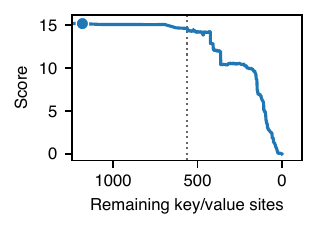}}
        {\includegraphics[width=\linewidth]{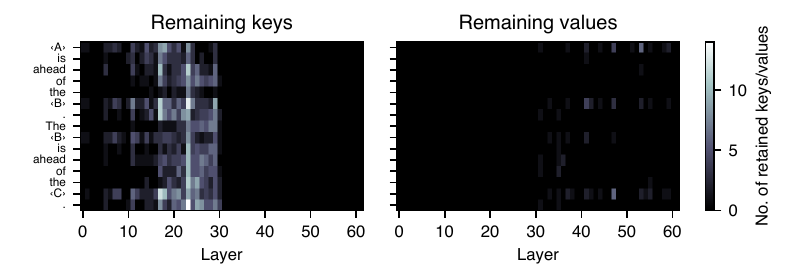}}
        {\includegraphics[width=\linewidth]{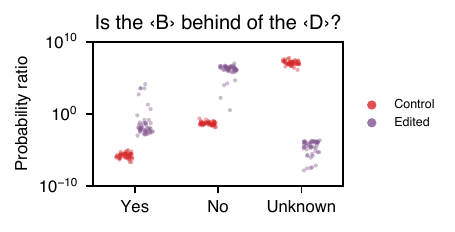}}
        {\includegraphics[width=\linewidth]{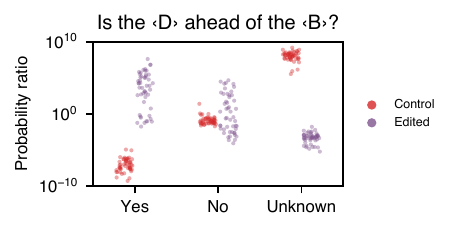}}
    \caption{\textbf{Key--value erasure and editing: ahead--behind relationships.}
        Results are shown for Gemma-3-27B. Procedures follow main-text Fig.~\figref{fig:binding}.
        The control context is ``The ‹A› is ahead of the ‹B›. The ‹B› is ahead of the ‹C›'';
        the donor context is ``The ‹D› is ahead of the ‹E›. The ‹E› is ahead of the ‹F›''.
        \textbf{A}, Responses for the keys-first, keys-only, and values-first memories.
        \textbf{B}, Final portion of the pruning trajectory.
        \textbf{C}, Distribution of the 1104 keys and 79 values retained by this mask,
        together comprising 3.98\% of all key/value sites.
        \textbf{D, E}, Responses before and after replacing selected keys associated
        with the first entity in the control memory with the corresponding donor keys.
        The wording ``behind of'' is a grammatical error in the prompt template; the intended wording is ``behind''. It is retained here to match the prompts presented to the model.
    }
    \label{SI-fig:erasure-ahead-behind}
\end{figure*}

\begin{figure*}[!htbp]
    \centering
    \erasurepanels
        {\includegraphics[width=\linewidth]{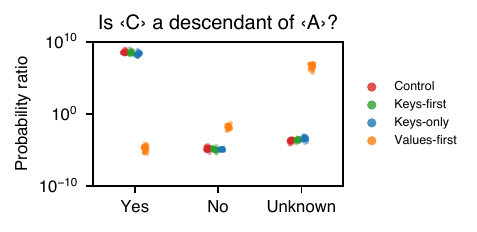}}
        {\includegraphics[width=\linewidth]{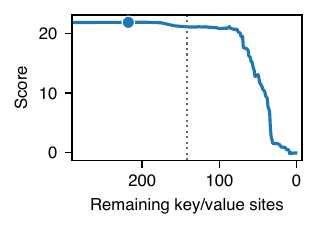}}
        {\includegraphics[width=\linewidth]{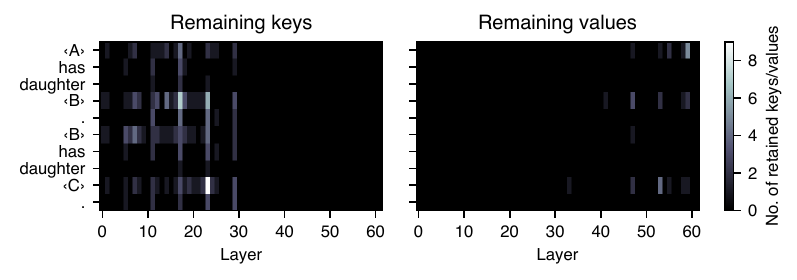}}
        {\includegraphics[width=\linewidth]{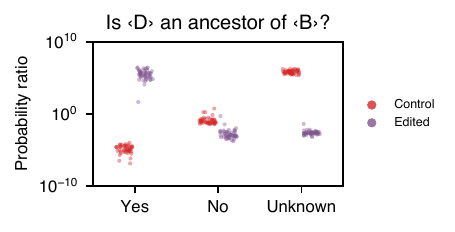}}
        {\includegraphics[width=\linewidth]{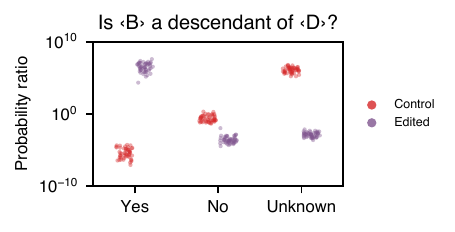}}
    \caption{\textbf{Key--value erasure and editing: ancestor--descendant relationships.}
        Results are shown for Gemma-3-27B. Procedures follow main-text Fig.~\figref{fig:binding}.
        The control context is ``‹A› has daughter ‹B›. ‹B› has daughter ‹C›'';
        the donor context is ``‹D› has daughter ‹E›. ‹E› has daughter ‹F›''.
        \textbf{A}, Responses for the keys-first, keys-only, and values-first memories.
        \textbf{B}, Final portion of the pruning trajectory.
        \textbf{C}, Distribution of the 188 keys and 30 values retained by this mask,
        together comprising 1.10\% of all key/value sites.
        \textbf{D, E}, Responses before and after replacing selected keys associated
        with the first entity in the control memory with the corresponding donor keys.
    }
    \label{SI-fig:erasure-family-trees-descendant-ancestor}
\end{figure*}

\begin{figure*}[!htbp]
    \centering
    \erasurepanels
        {\includegraphics[width=\linewidth]{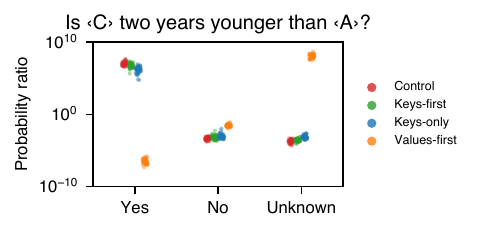}}
        {\includegraphics[width=\linewidth]{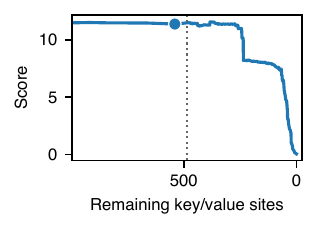}}
        {\includegraphics[width=\linewidth]{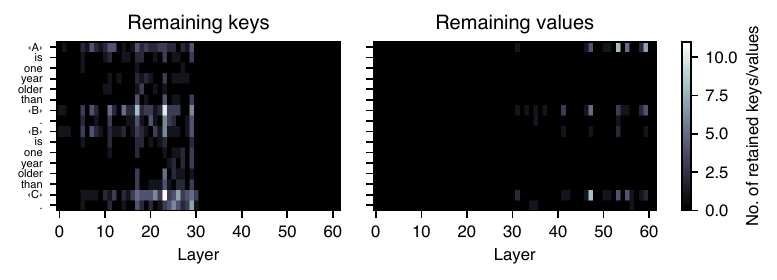}}
        {\includegraphics[width=\linewidth]{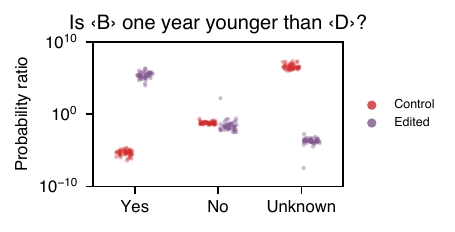}}
        {\includegraphics[width=\linewidth]{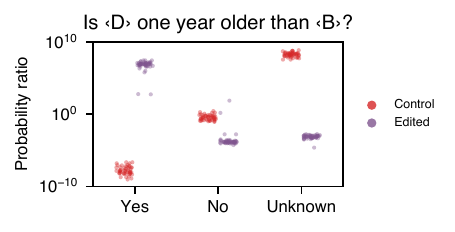}}
    \caption{\textbf{Key--value erasure and editing: exact age differences.}
        Results are shown for Gemma-3-27B. Procedures follow main-text Fig.~\figref{fig:binding}.
        The control context is ``‹A› is one year older than ‹B›. ‹B› is one year older than ‹C›'';
        the donor context is ``‹D› is one year older than ‹E›. ‹E› is one year older than ‹F›''.
        \textbf{A}, Responses for the keys-first, keys-only, and values-first memories.
        \textbf{B}, Final portion of the pruning trajectory.
        \textbf{C}, Distribution of the 449 keys and 91 values retained by this mask,
        together comprising 1.70\% of all key/value sites.
        \textbf{D, E}, Responses before and after replacing selected keys associated
        with the first entity in the control memory with the corresponding donor keys.
    }
    \label{SI-fig:erasure-older-younger-unique-locations-yes-no}
\end{figure*}

\begin{figure*}[!htbp]
    \centering
    \erasurepanels
        {\includegraphics[width=\linewidth]{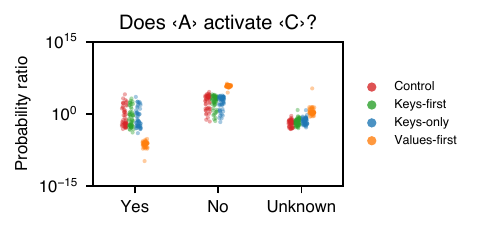}}
        {\includegraphics[width=\linewidth]{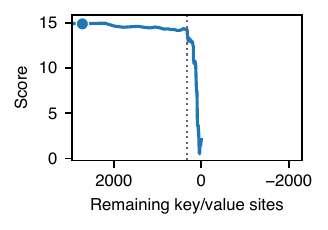}}
        {\includegraphics[width=\linewidth]{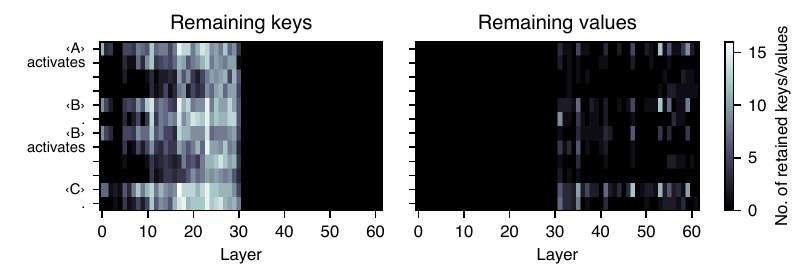}}
        {\includegraphics[width=\linewidth]{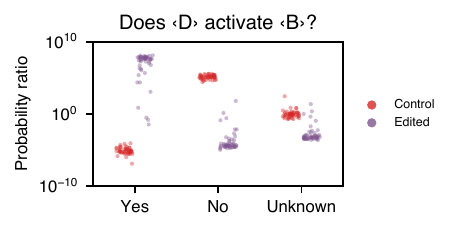}}
        {\includegraphics[width=\linewidth]{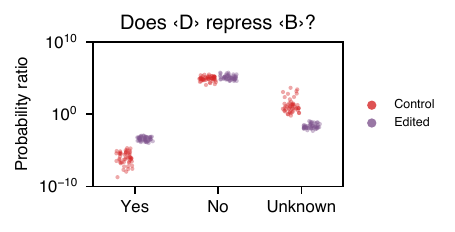}}
    \caption{\textbf{Key--value erasure and editing: gene regulatory networks.}
        Results are shown for Gemma-3-27B. Procedures follow main-text Fig.~\figref{fig:binding}.
        The control context is ``‹A› activates ‹B›. ‹B› activates ‹C›'';
        the donor context is ``‹D› activates ‹E›. ‹E› activates ‹F›''.
        \textbf{A}, Responses for the keys-first, keys-only, and values-first memories.
        \textbf{B}, Final portion of the pruning trajectory.
        \textbf{C}, Distribution of the 2,333 keys and 386 values retained by this mask,
        together comprising 11.42\% of all key/value sites.
        \textbf{D, E}, Responses before and after replacing selected keys associated
        with the first entity in the control memory with the corresponding donor keys.
    }
    \label{SI-fig:erasure-gene-regulatory-network}
\end{figure*}

\begin{figure*}[!htbp]
    \centering
    \erasurepanels
        {\includegraphics[width=\linewidth]{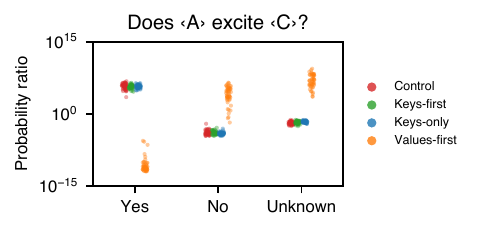}}
        {\includegraphics[width=\linewidth]{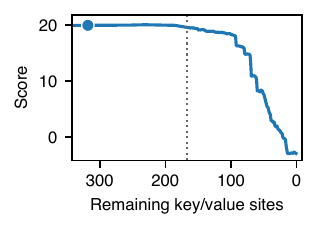}}
        {\includegraphics[width=\linewidth]{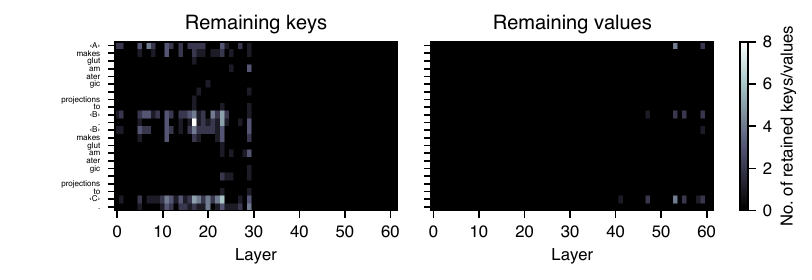}}
        {\includegraphics[width=\linewidth]{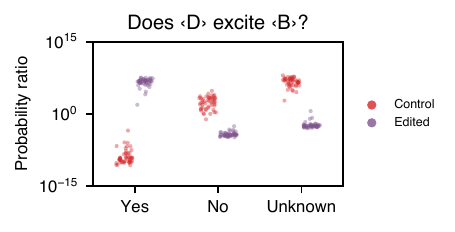}}
        {\includegraphics[width=\linewidth]{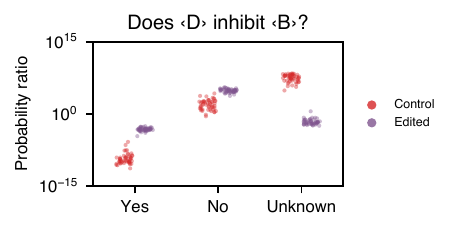}}
    \caption{\textbf{Key--value erasure and editing: neural circuits.}
        Results are shown for Gemma-3-27B. Procedures follow main-text Fig.~\figref{fig:binding}.
        The control context is ``‹A› makes glutamatergic projections to ‹B›. ‹B› makes glutamatergic projections to ‹C›'';
        the donor context is ``‹D› makes glutamatergic projections to ‹E›. ‹E› makes glutamatergic projections to ‹F›''.
        \textbf{A}, Responses for the keys-first, keys-only, and values-first memories.
        \textbf{B}, Final portion of the pruning trajectory.
        \textbf{C}, Distribution of the 292 keys and 26 values retained by this mask,
        together comprising 0.73\% of all key/value sites.
        \textbf{D, E}, Responses before and after replacing selected keys associated
        with the first entity in the control memory with the corresponding donor keys.
    }
    \label{SI-fig:erasure-neural-circuit}
\end{figure*}

\begin{figure*}[!htbp]
    \centering
    \erasurepanels
        {\includegraphics[width=\linewidth]{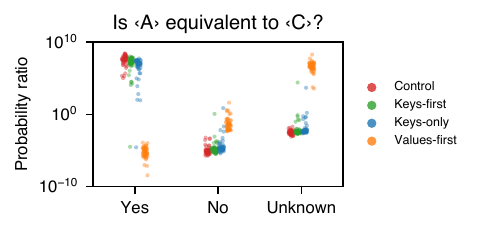}}
        {\includegraphics[width=\linewidth]{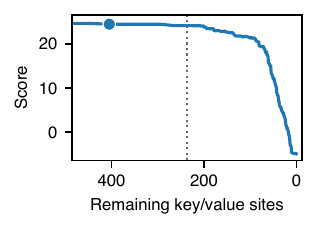}}
        {\includegraphics[width=\linewidth]{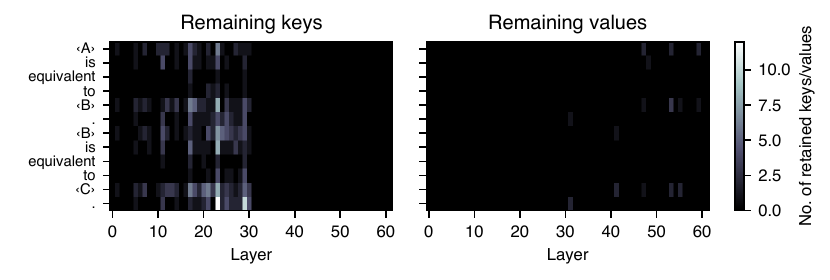}}
        {\includegraphics[width=\linewidth]{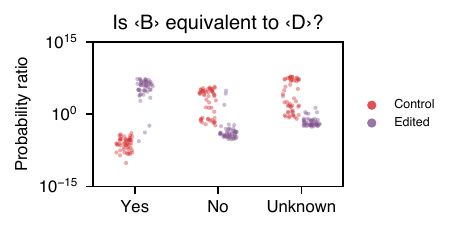}}
        {\includegraphics[width=\linewidth]{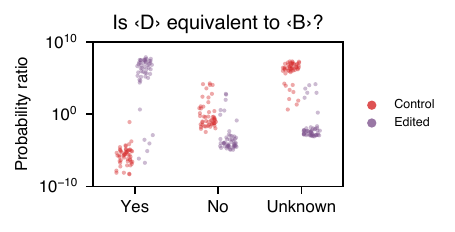}}
    \caption{\textbf{Key--value erasure and editing: propositional equivalence.}
        Results are shown for Gemma-3-27B. Procedures follow main-text Fig.~\figref{fig:binding}.
        The control context is ``‹A› is equivalent to ‹B›. ‹B› is equivalent to ‹C›'';
        the donor context is ``‹D› is equivalent to ‹E›. ‹E› is equivalent to ‹F›''.
        \textbf{A}, Responses for the keys-first, keys-only, and values-first memories.
        \textbf{B}, Final portion of the pruning trajectory.
        \textbf{C}, Distribution of the 381 keys and 24 values retained by this mask,
        together comprising 1.70\% of all key/value sites.
        \textbf{D, E}, Responses before and after replacing selected keys associated
        with the first entity in the control memory with the corresponding donor keys.
    }
    \label{SI-fig:erasure-proposition-equivalence}
\end{figure*}

\begin{figure*}[!htbp]
    \centering
    \erasurepanels
        {\includegraphics[width=\linewidth]{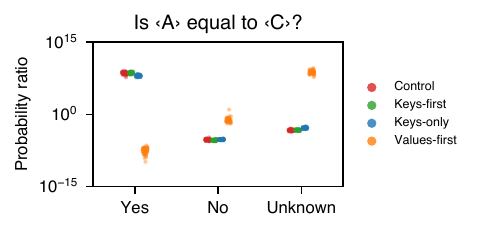}}
        {\includegraphics[width=\linewidth]{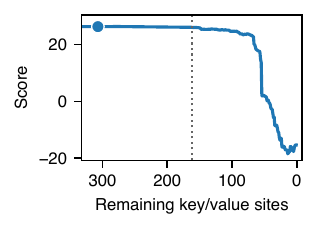}}
        {\includegraphics[width=\linewidth]{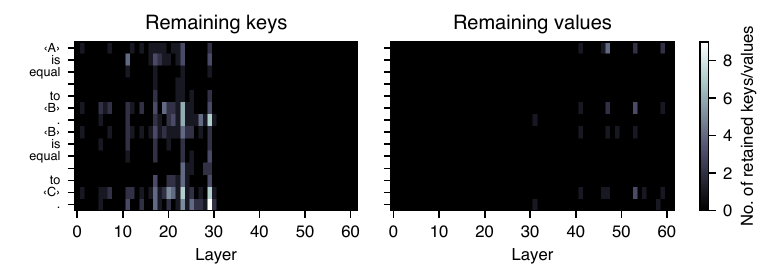}}
        {\includegraphics[width=\linewidth]{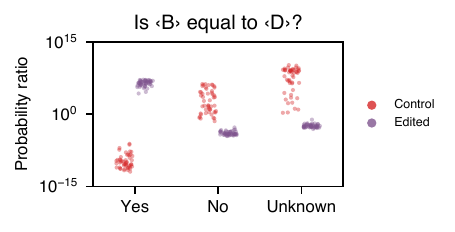}}
        {\includegraphics[width=\linewidth]{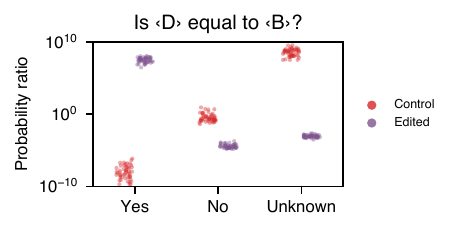}}
    \caption{\textbf{Key--value erasure and editing: variable equality.}
        Results are shown for Gemma-3-27B. Procedures follow main-text Fig.~\figref{fig:binding}.
        The control context is ``‹A› is equal to ‹B›. ‹B› is equal to ‹C›'';
        the donor context is ``‹D› is equal to ‹E›. ‹E› is equal to ‹F›''.
        \textbf{A}, Responses for the keys-first, keys-only, and values-first memories.
        \textbf{B}, Final portion of the pruning trajectory.
        \textbf{C}, Distribution of the 275 keys and 32 values retained by this mask,
        together comprising 1.11\% of all key/value sites.
        \textbf{D, E}, Responses before and after replacing selected keys associated
        with the first entity in the control memory with the corresponding donor keys.
    }
    \label{SI-fig:erasure-variable-equivalence}
\end{figure*}
