# Supplementary material for: Cognitive Maps in Large Language Models
Source: arXiv:2610.25596 source file (2026-11-06)
Supplement: Supplementary file 20 [file retrospective_prospective.tex]

\clearpage

\subsection{Retrospective and prospective information across tasks}

\begin{figure*}[!htbp]
    \centering
    \fourpanelrowwithlegend
        {\includegraphics[width=\linewidth]{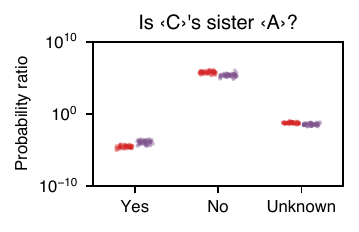}}
        {\includegraphics[width=\linewidth]{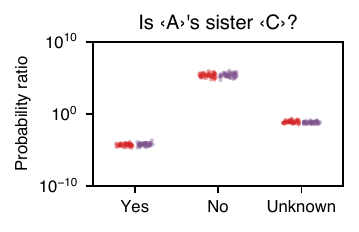}}
        {\includegraphics[width=\linewidth]{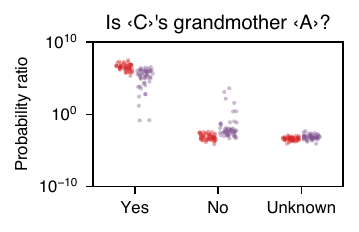}}
        {\includegraphics[width=\linewidth]{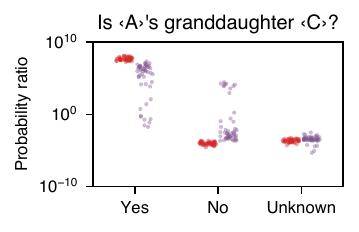}}
        {\includegraphics[width=0.28\textwidth]{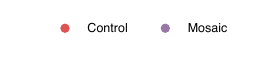}}
    \caption{\textbf{Retrospective and prospective information: family trees.}
        Results are shown for Gemma-3-27B.
        The control context is ``‹A› has daughter ‹B›. ‹B› has daughter ‹C›'';
        the donor context is ``‹A› has mother ‹B›. ‹B› has daughter ‹C›''.
        The mosaic was constructed as in main-text Fig.~\figref{fig:composition}.
    }
    \label{SI-fig:retrospective-prospective-family-tree-yes-no}
\end{figure*}

\begin{figure*}[!htbp]
    \centering
    \fourpanelrowwithlegend
        {\includegraphics[width=\linewidth]{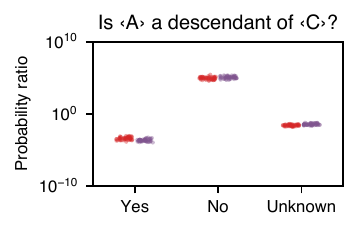}}
        {\includegraphics[width=\linewidth]{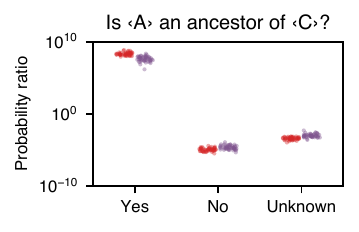}}
        {\includegraphics[width=\linewidth]{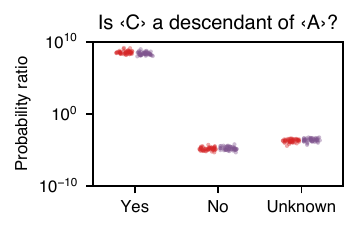}}
        {\includegraphics[width=\linewidth]{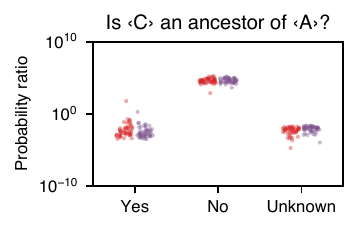}}
        {\includegraphics[width=0.28\textwidth]{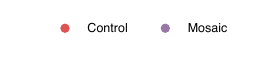}}
    \caption{\textbf{Retrospective and prospective information: ancestor--descendant relationships.}
        Results are shown for Gemma-3-27B.
        The control context is ``‹A› has daughter ‹B›. ‹B› has daughter ‹C›'';
        the donor context is ``‹A› has mother ‹B›. ‹B› has daughter ‹C›''.
        The mosaic was constructed as in main-text Fig.~\figref{fig:composition}.
    }
    \label{SI-fig:retrospective-prospective-family-trees-descendant-ancestor}
\end{figure*}

\begin{figure*}[!htbp]
    \centering
    \fourpanelrowwithlegend
        {\includegraphics[width=\linewidth]{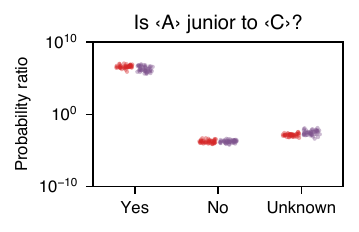}}
        {\includegraphics[width=\linewidth]{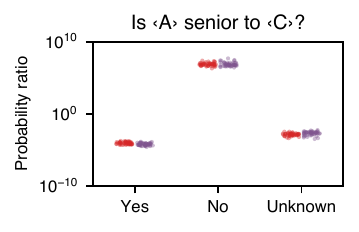}}
        {\includegraphics[width=\linewidth]{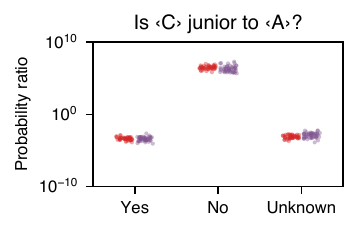}}
        {\includegraphics[width=\linewidth]{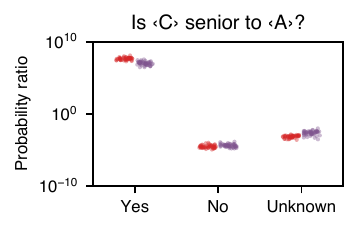}}
        {\includegraphics[width=0.28\textwidth]{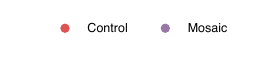}}
    \caption{\textbf{Retrospective and prospective information: company hierarchies.}
        Results are shown for Gemma-3-27B.
        The control context is ``‹A›'s boss is ‹B›. ‹B›'s boss is ‹C›'';
        the donor context is ``‹A›'s employee is ‹B›. ‹B›'s boss is ‹C›''.
        The mosaic was constructed as in main-text Fig.~\figref{fig:composition}.
    }
    \label{SI-fig:retrospective-prospective-company-structure}
\end{figure*}

\begin{figure*}[!htbp]
    \centering
    \fourpanelrowwithlegend
        {\includegraphics[width=\linewidth]{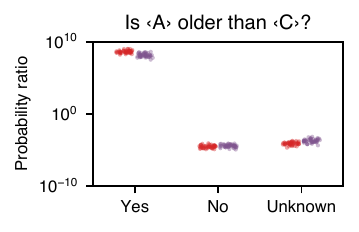}}
        {\includegraphics[width=\linewidth]{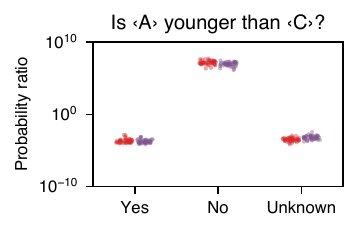}}
        {\includegraphics[width=\linewidth]{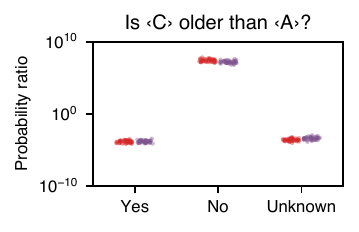}}
        {\includegraphics[width=\linewidth]{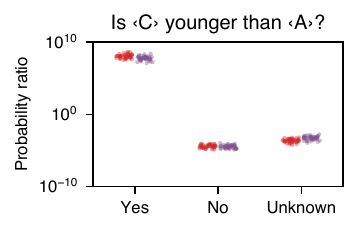}}
        {\includegraphics[width=0.28\textwidth]{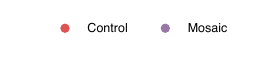}}
    \caption{\textbf{Retrospective and prospective information: age comparisons.}
        Results are shown for Gemma-3-27B.
        The control context is ``‹A› is older than ‹B›. ‹B› is older than ‹C›'';
        the donor context is ``‹A› is younger than ‹B›. ‹B› is older than ‹C›''.
        The mosaic was constructed as in main-text Fig.~\figref{fig:composition}.
    }
    \label{SI-fig:retrospective-prospective-older-younger}
\end{figure*}

\begin{figure*}[!htbp]
    \centering
    \fourpanelrowwithlegend
        {\includegraphics[width=\linewidth]{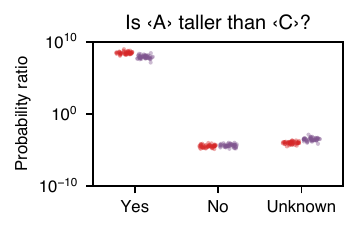}}
        {\includegraphics[width=\linewidth]{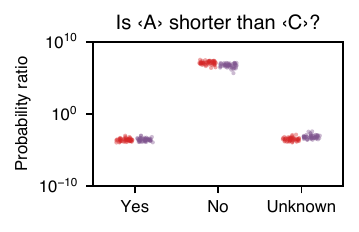}}
        {\includegraphics[width=\linewidth]{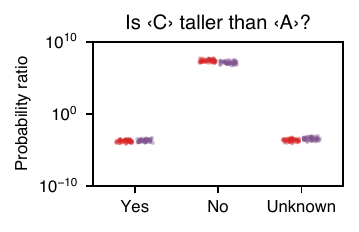}}
        {\includegraphics[width=\linewidth]{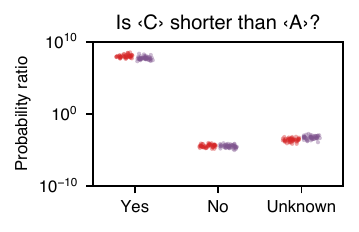}}
        {\includegraphics[width=0.28\textwidth]{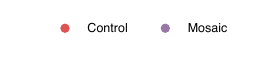}}
    \caption{\textbf{Retrospective and prospective information: height comparisons.}
        Results are shown for Gemma-3-27B.
        The control context is ``‹A› is taller than ‹B›. ‹B› is taller than ‹C›'';
        the donor context is ``‹A› is shorter than ‹B›. ‹B› is taller than ‹C›''.
        The mosaic was constructed as in main-text Fig.~\figref{fig:composition}.
    }
    \label{SI-fig:retrospective-prospective-taller-shorter}
\end{figure*}

\begin{figure*}[!htbp]
    \centering
    \fourpanelrowwithlegend
        {\includegraphics[width=\linewidth]{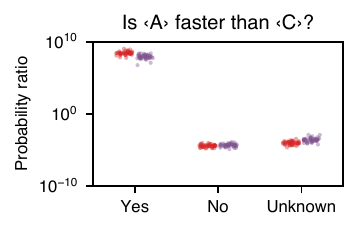}}
        {\includegraphics[width=\linewidth]{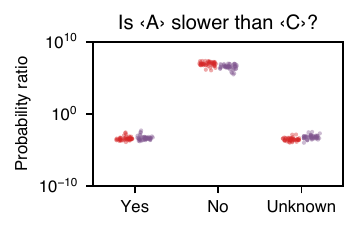}}
        {\includegraphics[width=\linewidth]{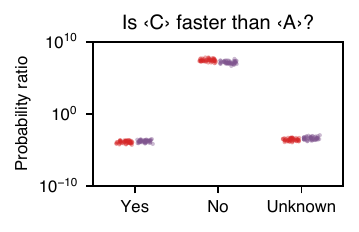}}
        {\includegraphics[width=\linewidth]{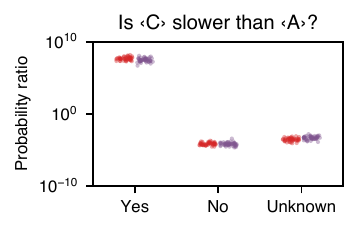}}
        {\includegraphics[width=0.28\textwidth]{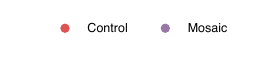}}
    \caption{\textbf{Retrospective and prospective information: speed comparisons.}
        Results are shown for Gemma-3-27B.
        The control context is ``‹A› is faster than ‹B›. ‹B› is faster than ‹C›'';
        the donor context is ``‹A› is slower than ‹B›. ‹B› is faster than ‹C›''.
        The mosaic was constructed as in main-text Fig.~\figref{fig:composition}.
    }
    \label{SI-fig:retrospective-prospective-faster-slower}
\end{figure*}

\begin{figure*}[!htbp]
    \centering
    \fourpanelrowwithlegend
        {\includegraphics[width=\linewidth]{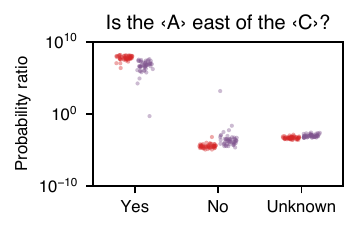}}
        {\includegraphics[width=\linewidth]{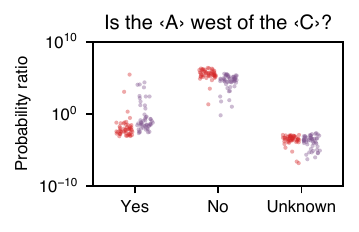}}
        {\includegraphics[width=\linewidth]{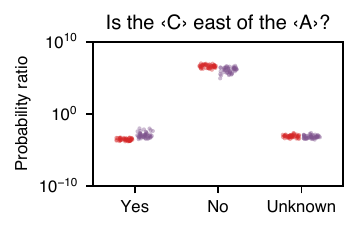}}
        {\includegraphics[width=\linewidth]{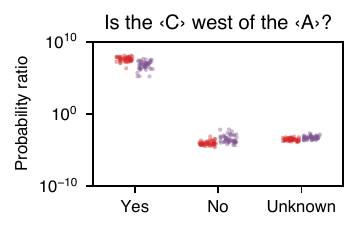}}
        {\includegraphics[width=0.28\textwidth]{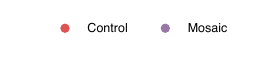}}
    \caption{\textbf{Retrospective and prospective information: east--west relationships.}
        Results are shown for Gemma-3-27B.
        The control context is ``The ‹A› is east of the ‹B›. The ‹B› is east of the ‹C›'';
        the donor context is ``The ‹A› is west of the ‹B›. The ‹B› is east of the ‹C›''.
        The mosaic was constructed as in main-text Fig.~\figref{fig:composition}.
    }
    \label{SI-fig:retrospective-prospective-east-west}
\end{figure*}

\begin{figure*}[!htbp]
    \centering
    \fourpanelrowwithlegend
        {\includegraphics[width=\linewidth]{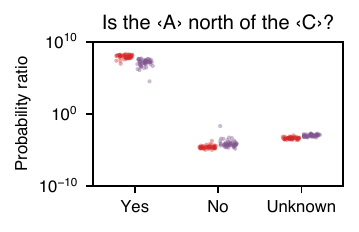}}
        {\includegraphics[width=\linewidth]{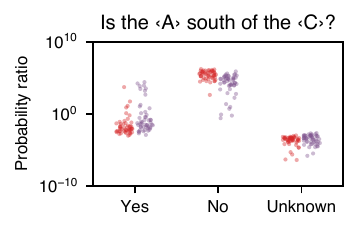}}
        {\includegraphics[width=\linewidth]{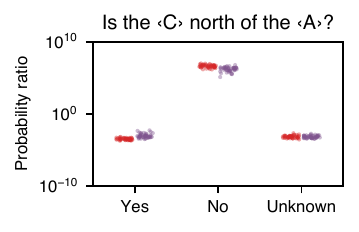}}
        {\includegraphics[width=\linewidth]{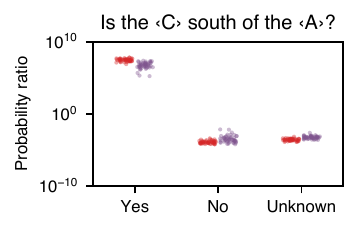}}
        {\includegraphics[width=0.28\textwidth]{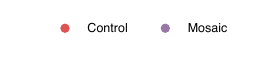}}
    \caption{\textbf{Retrospective and prospective information: north--south relationships.}
        Results are shown for Gemma-3-27B.
        The control context is ``The ‹A› is north of the ‹B›. The ‹B› is north of the ‹C›'';
        the donor context is ``The ‹A› is south of the ‹B›. The ‹B› is north of the ‹C›''.
        The mosaic was constructed as in main-text Fig.~\figref{fig:composition}.
    }
    \label{SI-fig:retrospective-prospective-north-south}
\end{figure*}

\begin{figure*}[!htbp]
    \centering
    \fourpanelrowwithlegend
        {\includegraphics[width=\linewidth]{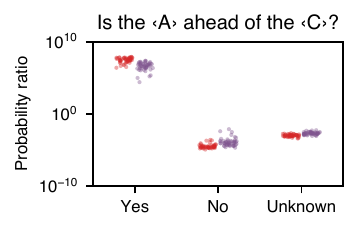}}
        {\includegraphics[width=\linewidth]{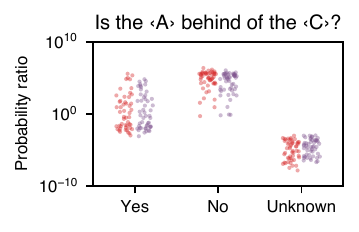}}
        {\includegraphics[width=\linewidth]{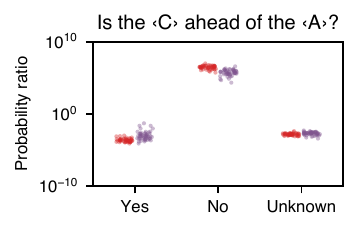}}
        {\includegraphics[width=\linewidth]{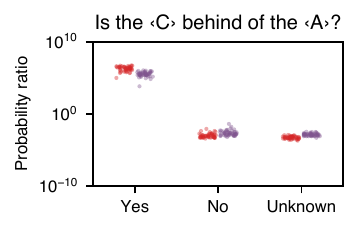}}
        {\includegraphics[width=0.28\textwidth]{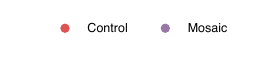}}
    \caption{\textbf{Retrospective and prospective information: ahead--behind relationships.}
        Results are shown for Gemma-3-27B.
        The control context is ``The ‹A› is ahead of the ‹B›. The ‹B› is ahead of the ‹C›'';
        the donor context is ``The ‹A› is behind of the ‹B›. The ‹B› is ahead of the ‹C›''.
        The mosaic was constructed as in main-text Fig.~\figref{fig:composition}. The wording ``behind of'' is a grammatical
        error in the prompt template; the intended wording is ``behind''.
        It is retained here to match the prompts presented to the model.
    }
    \label{SI-fig:retrospective-prospective-ahead-behind}

\end{figure*}

\begin{figure*}[!htbp]
    \centering
    \fourpanelrowwithlegend
        {\includegraphics[width=\linewidth]{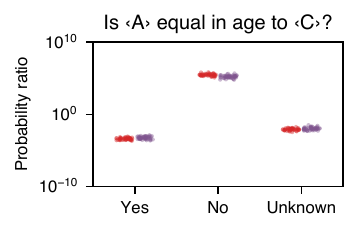}}
        {\includegraphics[width=\linewidth]{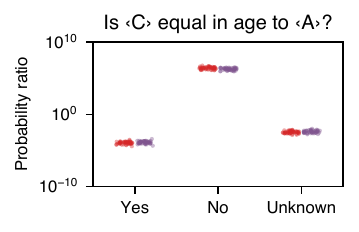}}
        {\includegraphics[width=\linewidth]{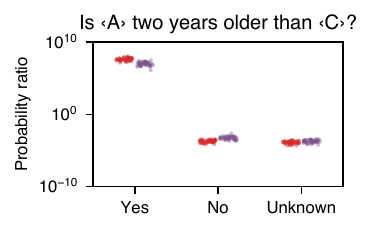}}
        {\includegraphics[width=\linewidth]{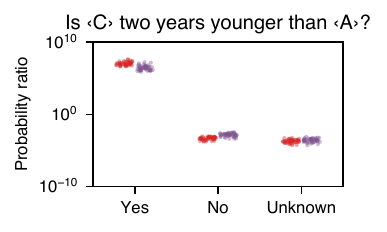}}
        {\includegraphics[width=0.28\textwidth]{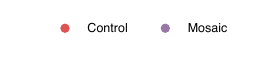}}
    \caption{\textbf{Retrospective and prospective information: exact age differences.}
        Results are shown for Gemma-3-27B.
        The control context is ``‹A› is one year older than ‹B›. ‹B› is one year older than ‹C›'';
        the donor context is ``‹A› is one year younger than ‹B›. ‹B› is one year older than ‹C›''.
        The mosaic was constructed as in main-text Fig.~\figref{fig:composition}.
    }
    \label{SI-fig:retrospective-prospective-older-younger-unique-locations-yes-no}
\end{figure*}

\begin{figure*}[!htbp]
    \centering
    \twopanelrow
        {\includegraphics[width=\linewidth]{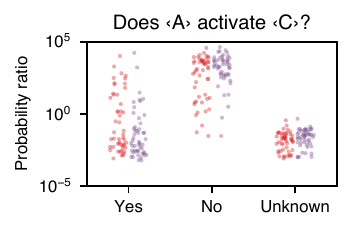}}
        {\includegraphics[width=\linewidth]{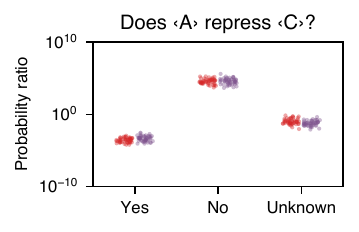}}
        {\includegraphics[width=0.28\textwidth]{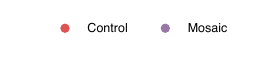}}
    \caption{\textbf{Retrospective and prospective information: gene regulatory networks.}
        Results are shown for Gemma-3-27B.
        The control context is ``‹A› activates ‹B›. ‹B› activates ‹C›'';
        the donor context is ``‹A› represses ‹B›. ‹B› activates ‹C›''.
        The mosaic was constructed as in main-text Fig.~\figref{fig:composition}.
    }
    \label{SI-fig:retrospective-prospective-gene-regulatory-network}
\end{figure*}

\begin{figure*}[!htbp]
    \centering
    \twopanelrow
        {\includegraphics[width=\linewidth]{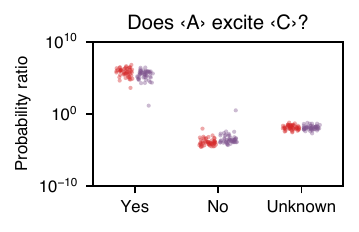}}
        {\includegraphics[width=\linewidth]{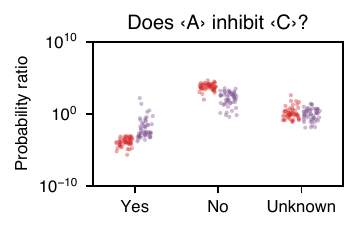}}
        {\includegraphics[width=0.28\textwidth]{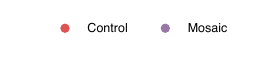}}
    \caption{\textbf{Retrospective and prospective information: neural circuits.}
        Results are shown for Gemma-3-27B.
        The control context is ``‹A› makes glutamatergic projections to ‹B›. ‹B› makes glutamatergic projections to ‹C›'';
        the donor context is ``‹A› makes GABAergic projections to ‹B›. ‹B› makes glutamatergic projections to ‹C›''.
        The mosaic was constructed as in main-text Fig.~\figref{fig:composition}.
    }
    \label{SI-fig:retrospective-prospective-neural-circuit}
\end{figure*}

\begin{figure*}[!htbp]
    \centering
    \twopanelrow
        {\includegraphics[width=\linewidth]{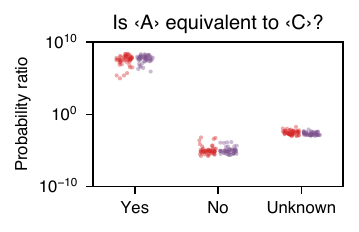}}
        {\includegraphics[width=\linewidth]{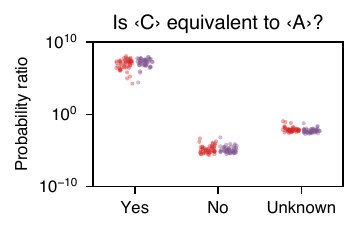}}
        {\includegraphics[width=0.28\textwidth]{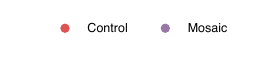}}
    \caption{\textbf{Retrospective and prospective information: propositional equivalence.}
        Results are shown for Gemma-3-27B.
        The control context is ``‹A› is equivalent to ‹B›. ‹B› is equivalent to ‹C›'';
        the donor context is ``‹A› is incompatible with ‹B›. ‹B› is equivalent to ‹C›''.
        The mosaic was constructed as in main-text Fig.~\figref{fig:composition}.
    }
    \label{SI-fig:retrospective-prospective-proposition-equivalence}
\end{figure*}

\begin{figure*}[!htbp]
    \centering
    \twopanelrow
        {\includegraphics[width=\linewidth]{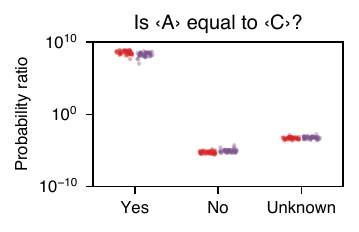}}
        {\includegraphics[width=\linewidth]{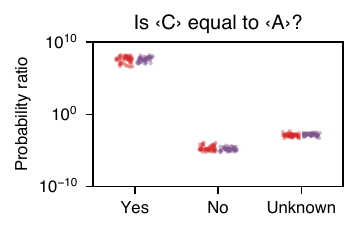}}
        {\includegraphics[width=0.28\textwidth]{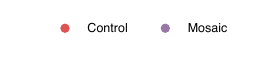}}
    \caption{\textbf{Retrospective and prospective information: variable equality.}
        Results are shown for Gemma-3-27B.
        The control context is ``‹A› is equal to ‹B›. ‹B› is equal to ‹C›'';
        the donor context is ``‹A› is not equal to ‹B›. ‹B› is equal to ‹C›''.
        The mosaic was constructed as in main-text Fig.~\figref{fig:composition}.
    }
    \label{SI-fig:retrospective-prospective-variable-equivalence}
\end{figure*}
