# Supplementary material for: Cognitive Maps in Large Language Models
Source: arXiv:2610.25596 source file (2026-11-06)
Supplement: Supplementary file 21 [file separability.tex]

\clearpage

\subsection{Identity--structure separability across tasks}

\begin{figure*}[!htbp]
    \centering
    \sixpanelgrid
        {\includegraphics[width=\linewidth]{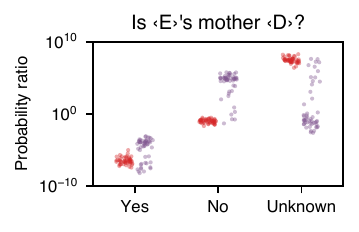}}
        {\includegraphics[width=\linewidth]{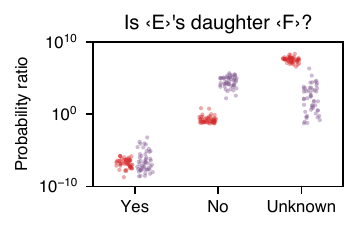}}
        {\includegraphics[width=\linewidth]{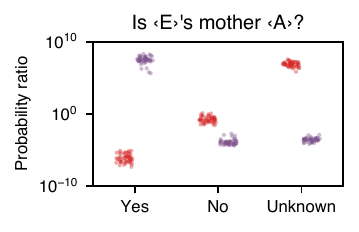}}
        {\includegraphics[width=\linewidth]{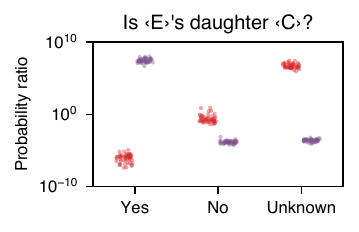}}
        {\includegraphics[width=\linewidth]{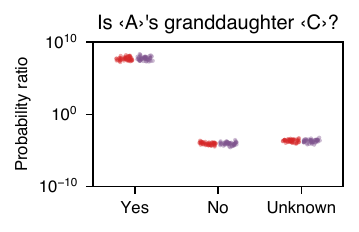}}
        {\includegraphics[width=\linewidth]{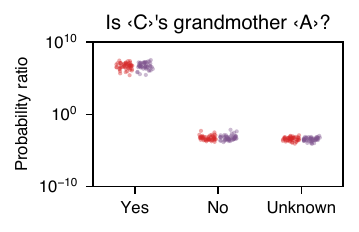}}
        {\includegraphics[width=0.28\textwidth]{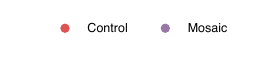}}
    \caption{
        \textbf{Identity--structure separability: family trees.}
        Results are shown for Gemma-3-27B.
        The control context is ``‹A› has daughter ‹B›. ‹B› has daughter ‹C›'';
        the donor context is ``‹D› has daughter ‹E›. ‹E› has daughter ‹F›''.
        The mosaic was constructed as in main-text Fig.~\figref{fig:separability}.
    }
    \label{SI-fig:separability-gemma27b-family-tree-yes-no}
\end{figure*}

\begin{figure*}[!htbp]
    \centering
    \sixpanelgrid
        {\includegraphics[width=\linewidth]{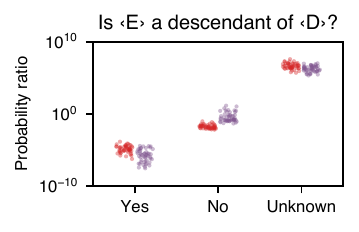}}
        {\includegraphics[width=\linewidth]{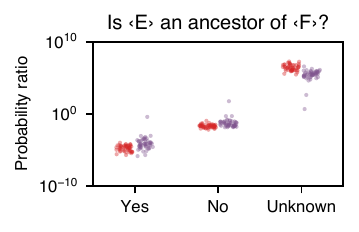}}
        {\includegraphics[width=\linewidth]{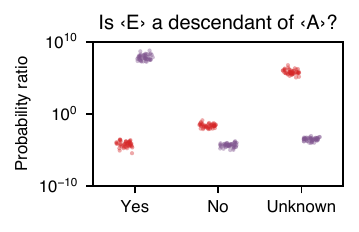}}
        {\includegraphics[width=\linewidth]{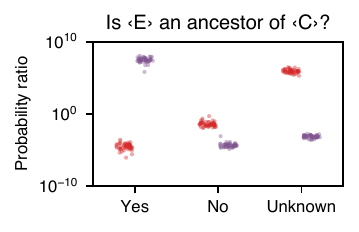}}
        {\includegraphics[width=\linewidth]{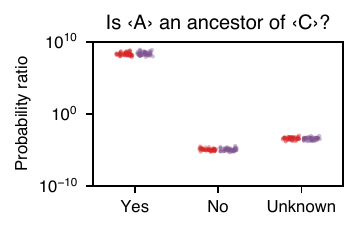}}
        {\includegraphics[width=\linewidth]{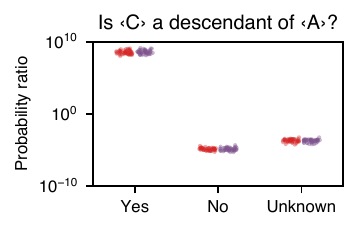}}
        {\includegraphics[width=0.28\textwidth]{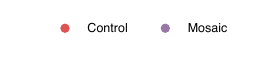}}
    \caption{
        \textbf{Identity--structure separability: ancestor--descendant relationships.}
        Results are shown for Gemma-3-27B.
        The control context is ``‹A› has daughter ‹B›. ‹B› has daughter ‹C›'';
        the donor context is ``‹D› has daughter ‹E›. ‹E› has daughter ‹F›''.
        The mosaic was constructed as in main-text Fig.~\figref{fig:separability}.
    }
    \label{SI-fig:separability-gemma27b-family-trees-descendant-ancestor}
\end{figure*}

\begin{figure*}[!htbp]
    \centering
    \sixpanelgrid
        {\includegraphics[width=\linewidth]{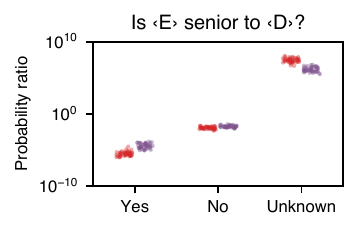}}
        {\includegraphics[width=\linewidth]{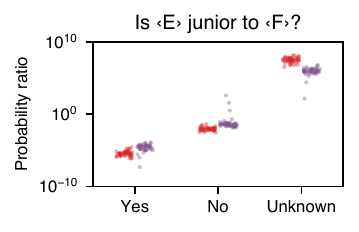}}
        {\includegraphics[width=\linewidth]{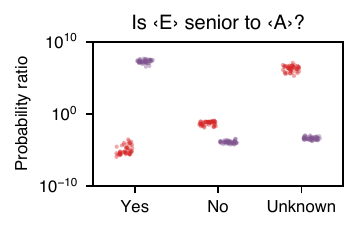}}
        {\includegraphics[width=\linewidth]{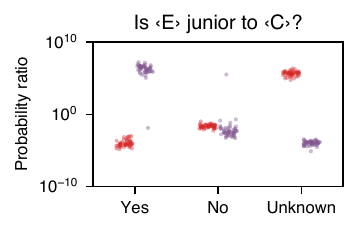}}
        {\includegraphics[width=\linewidth]{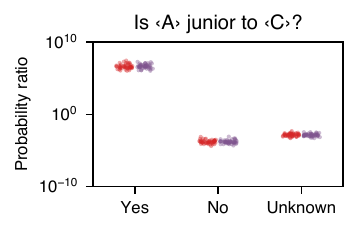}}
        {\includegraphics[width=\linewidth]{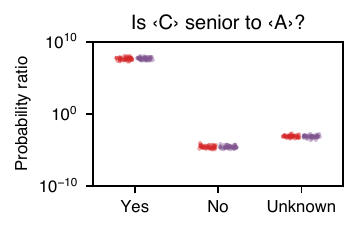}}
        {\includegraphics[width=0.28\textwidth]{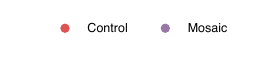}}
    \caption{
        \textbf{Identity--structure separability: company hierarchies.}
        Results are shown for Gemma-3-27B.
        The control context is ``‹A›'s boss is ‹B›. ‹B›'s boss is ‹C›'';
        the donor context is ``‹D›'s boss is ‹E›. ‹E›'s boss is ‹F›''.
        The mosaic was constructed as in main-text Fig.~\figref{fig:separability}.
    }
    \label{SI-fig:separability-gemma27b-company-structure}
\end{figure*}

\begin{figure*}[!htbp]
    \centering
    \sixpanelgrid
        {\includegraphics[width=\linewidth]{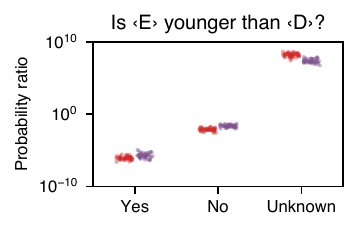}}
        {\includegraphics[width=\linewidth]{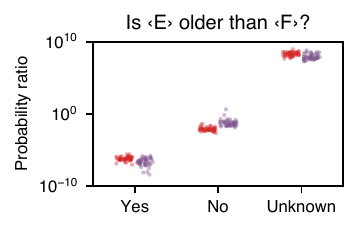}}
        {\includegraphics[width=\linewidth]{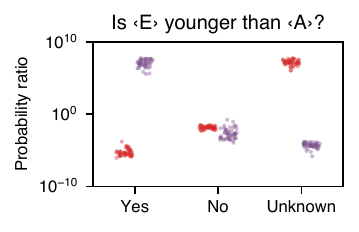}}
        {\includegraphics[width=\linewidth]{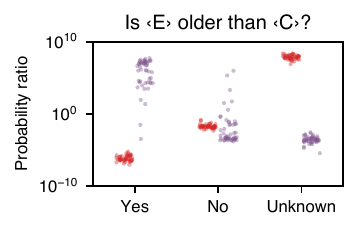}}
        {\includegraphics[width=\linewidth]{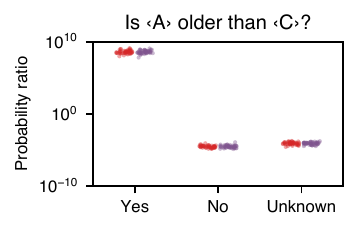}}
        {\includegraphics[width=\linewidth]{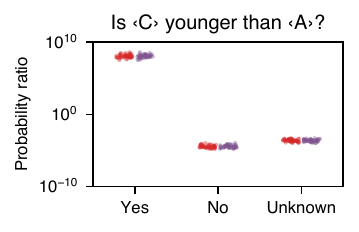}}
        {\includegraphics[width=0.28\textwidth]{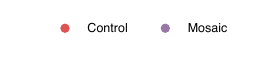}}
    \caption{
        \textbf{Identity--structure separability: age comparisons.}
        Results are shown for Gemma-3-27B.
        The control context is ``‹A› is older than ‹B›. ‹B› is older than ‹C›'';
        the donor context is ``‹D› is older than ‹E›. ‹E› is older than ‹F›''.
        The mosaic was constructed as in main-text Fig.~\figref{fig:separability}.
    }
    \label{SI-fig:separability-gemma27b-older-younger}
\end{figure*}

\begin{figure*}[!htbp]
    \centering
    \sixpanelgrid
        {\includegraphics[width=\linewidth]{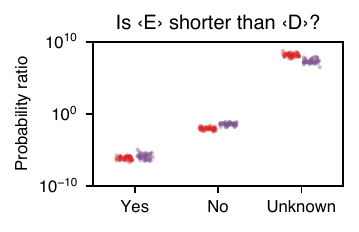}}
        {\includegraphics[width=\linewidth]{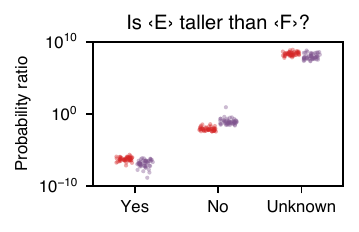}}
        {\includegraphics[width=\linewidth]{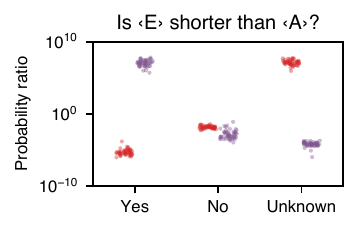}}
        {\includegraphics[width=\linewidth]{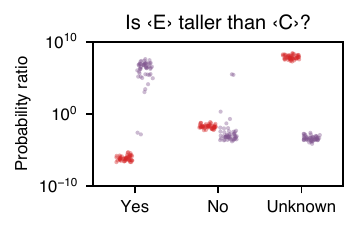}}
        {\includegraphics[width=\linewidth]{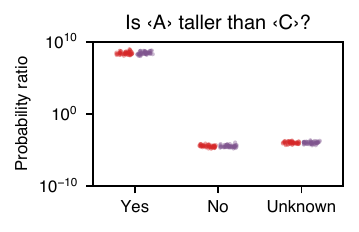}}
        {\includegraphics[width=\linewidth]{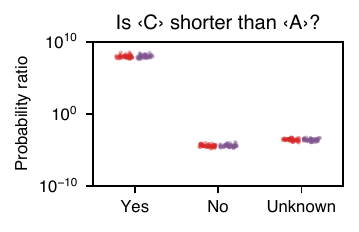}}
        {\includegraphics[width=0.28\textwidth]{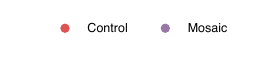}}
    \caption{
        \textbf{Identity--structure separability: height comparisons.}
        Results are shown for Gemma-3-27B.
        The control context is ``‹A› is taller than ‹B›. ‹B› is taller than ‹C›'';
        the donor context is ``‹D› is taller than ‹E›. ‹E› is taller than ‹F›''.
        The mosaic was constructed as in main-text Fig.~\figref{fig:separability}.
    }
    \label{SI-fig:separability-gemma27b-taller-shorter}
\end{figure*}

\begin{figure*}[!htbp]
    \centering
    \sixpanelgrid
        {\includegraphics[width=\linewidth]{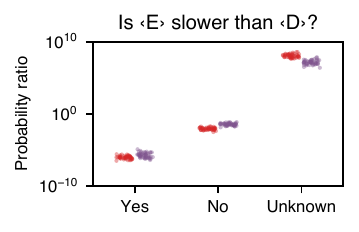}}
        {\includegraphics[width=\linewidth]{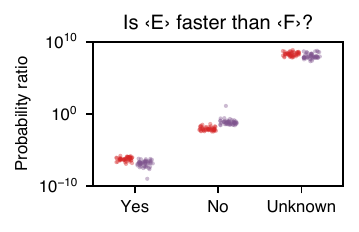}}
        {\includegraphics[width=\linewidth]{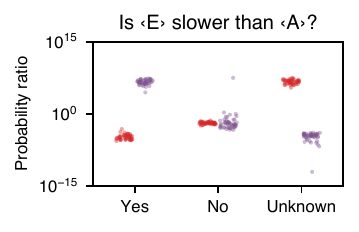}}
        {\includegraphics[width=\linewidth]{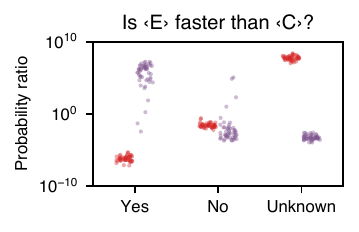}}
        {\includegraphics[width=\linewidth]{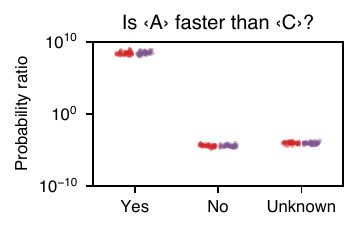}}
        {\includegraphics[width=\linewidth]{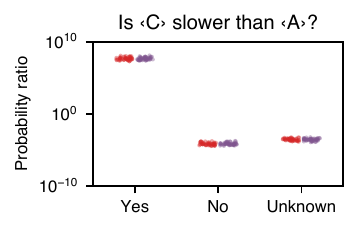}}
        {\includegraphics[width=0.28\textwidth]{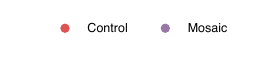}}
    \caption{
        \textbf{Identity--structure separability: speed comparisons.}
        Results are shown for Gemma-3-27B.
        The control context is ``‹A› is faster than ‹B›. ‹B› is faster than ‹C›'';
        the donor context is ``‹D› is faster than ‹E›. ‹E› is faster than ‹F›''.
        The mosaic was constructed as in main-text Fig.~\figref{fig:separability}.
    }
    \label{SI-fig:separability-gemma27b-faster-slower}
\end{figure*}

\begin{figure*}[!htbp]
    \centering
    \sixpanelgrid
        {\includegraphics[width=\linewidth]{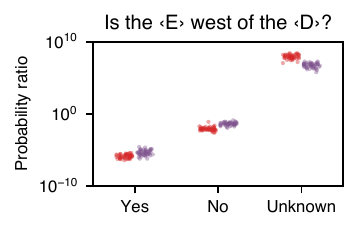}}
        {\includegraphics[width=\linewidth]{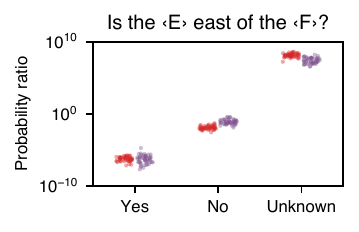}}
        {\includegraphics[width=\linewidth]{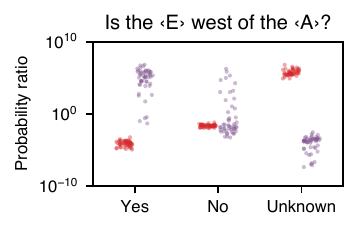}}
        {\includegraphics[width=\linewidth]{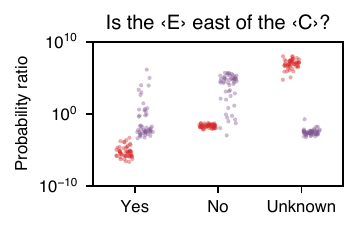}}
        {\includegraphics[width=\linewidth]{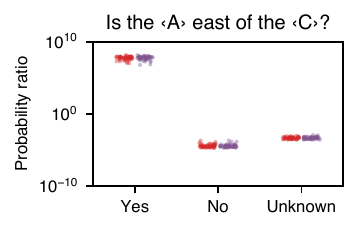}}
        {\includegraphics[width=\linewidth]{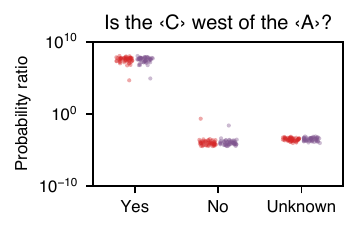}}
        {\includegraphics[width=0.28\textwidth]{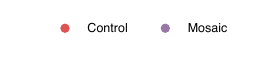}}
    \caption{
        \textbf{Identity--structure separability: east--west relationships.}
        Results are shown for Gemma-3-27B.
        The control context is ``The ‹A› is east of the ‹B›. The ‹B› is east of the ‹C›'';
        the donor context is ``The ‹D› is east of the ‹E›. The ‹E› is east of the ‹F›''.
        The mosaic was constructed as in main-text Fig.~\figref{fig:separability}.
    }
    \label{SI-fig:separability-gemma27b-east-west}
\end{figure*}

\begin{figure*}[!htbp]
    \centering
    \sixpanelgrid
        {\includegraphics[width=\linewidth]{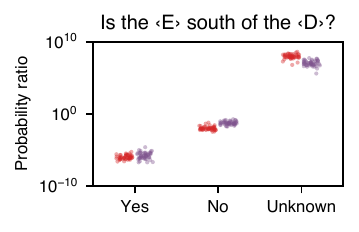}}
        {\includegraphics[width=\linewidth]{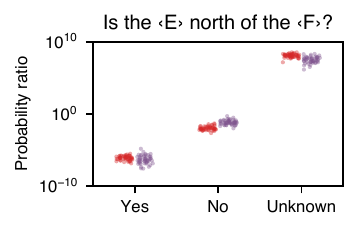}}
        {\includegraphics[width=\linewidth]{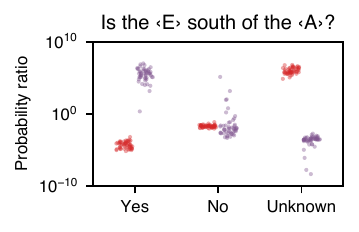}}
        {\includegraphics[width=\linewidth]{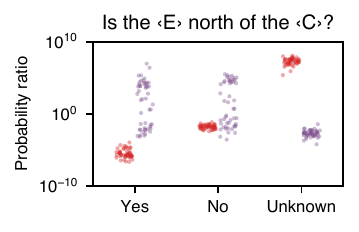}}
        {\includegraphics[width=\linewidth]{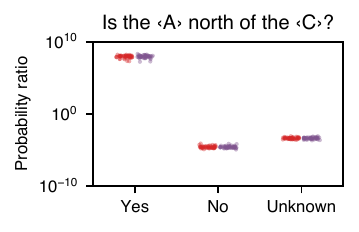}}
        {\includegraphics[width=\linewidth]{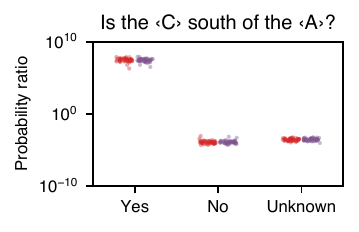}}
        {\includegraphics[width=0.28\textwidth]{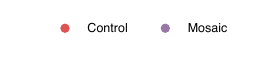}}
    \caption{
        \textbf{Identity--structure separability: north--south relationships.}
        Results are shown for Gemma-3-27B.
        The control context is ``The ‹A› is north of the ‹B›. The ‹B› is north of the ‹C›'';
        the donor context is ``The ‹D› is north of the ‹E›. The ‹E› is north of the ‹F›''.
        The mosaic was constructed as in main-text Fig.~\figref{fig:separability}.
    }
    \label{SI-fig:separability-gemma27b-north-south}
\end{figure*}

\begin{figure*}[!htbp]
    \centering
    \sixpanelgrid
        {\includegraphics[width=\linewidth]{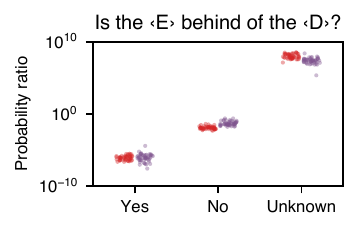}}
        {\includegraphics[width=\linewidth]{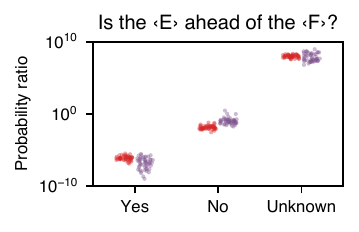}}
        {\includegraphics[width=\linewidth]{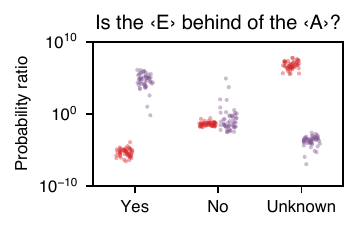}}
        {\includegraphics[width=\linewidth]{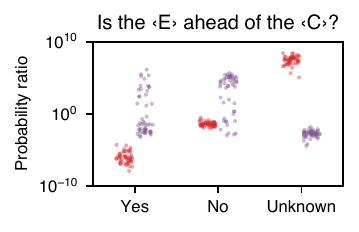}}
        {\includegraphics[width=\linewidth]{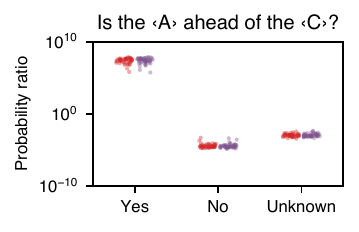}}
        {\includegraphics[width=\linewidth]{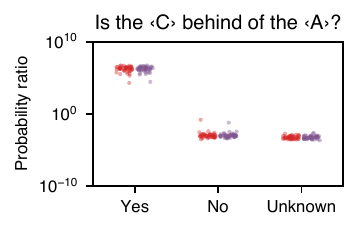}}
        {\includegraphics[width=0.28\textwidth]{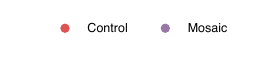}}
    \caption{
        \textbf{Identity--structure separability: ahead--behind relationships.}
        Results are shown for Gemma-3-27B.
        The control context is ``The ‹A› is ahead of the ‹B›. The ‹B› is ahead of the ‹C›'';
        the donor context is ``The ‹D› is ahead of the ‹E›. The ‹E› is ahead of the ‹F›''.
        The mosaic was constructed as in main-text Fig.~\figref{fig:separability}. The wording ‘behind of’ is a grammatical error in the prompt template; the intended wording is ‘behind’. It is retained here to match the prompts presented to the model.
    }
    \label{SI-fig:separability-gemma27b-ahead-behind}
\end{figure*}

\begin{figure*}[!htbp]
    \centering
    \sixpanelgrid
        {\includegraphics[width=\linewidth]{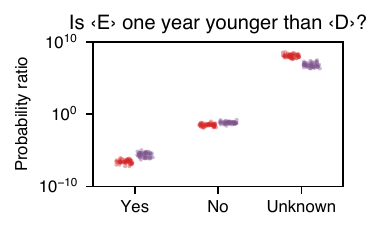}}
        {\includegraphics[width=\linewidth]{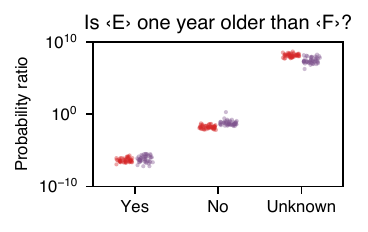}}
        {\includegraphics[width=\linewidth]{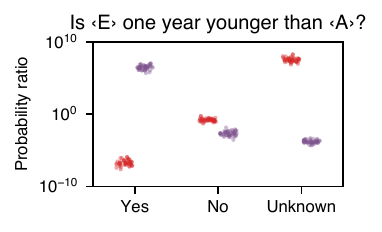}}
        {\includegraphics[width=\linewidth]{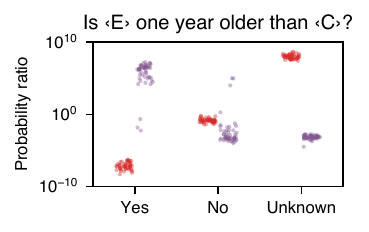}}
        {\includegraphics[width=\linewidth]{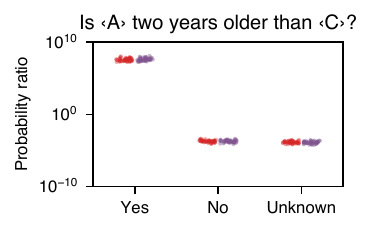}}
        {\includegraphics[width=\linewidth]{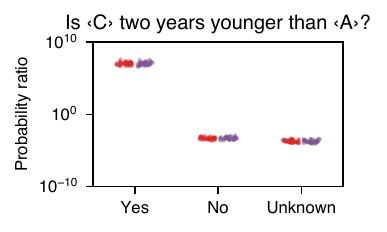}}
        {\includegraphics[width=0.28\textwidth]{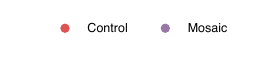}}
    \caption{
        \textbf{Identity--structure separability: exact age differences.}
        Results are shown for Gemma-3-27B.
        The control context is ``‹A› is one year older than ‹B›. ‹B› is one year older than ‹C›'';
        the donor context is ``‹D› is one year older than ‹E›. ‹E› is one year older than ‹F›''.
        The mosaic was constructed as in main-text Fig.~\figref{fig:separability}.
    }
    \label{SI-fig:separability-gemma27b-older-younger-unique-locations-yes-no}
\end{figure*}

\begin{figure*}[!htbp]
    \centering
    \fivepanelgrid
        {\includegraphics[width=\linewidth]{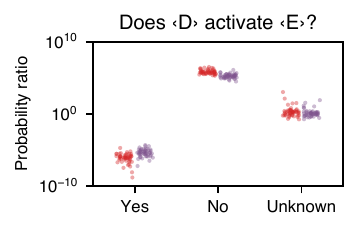}}
        {\includegraphics[width=\linewidth]{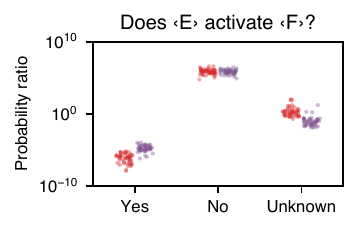}}
        {\includegraphics[width=\linewidth]{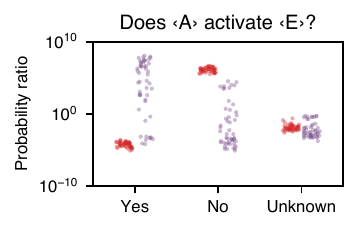}}
        {\includegraphics[width=\linewidth]{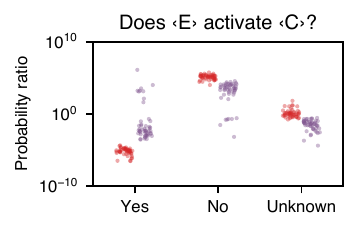}}
        {\includegraphics[width=\linewidth]{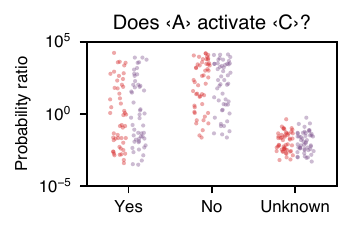}}
        {\includegraphics[width=0.28\textwidth]{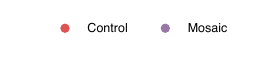}}
    \caption{
        \textbf{Identity--structure separability: gene regulatory networks.}
        Results are shown for Gemma-3-27B.
        The control context is ``‹A› activates ‹B›. ‹B› activates ‹C›'';
        the donor context is ``‹D› activates ‹E›. ‹E› activates ‹F›''.
        The mosaic was constructed as in main-text Fig.~\figref{fig:separability}.
    }
    \label{SI-fig:separability-gemma27b-gene-regulatory-network}
\end{figure*}

\begin{figure*}[!htbp]
    \centering
    \fivepanelgrid
        {\includegraphics[width=\linewidth]{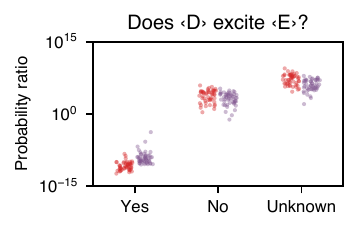}}
        {\includegraphics[width=\linewidth]{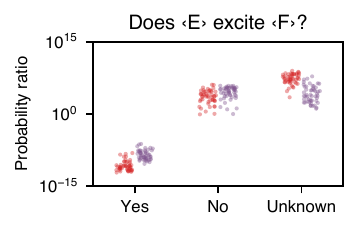}}
        {\includegraphics[width=\linewidth]{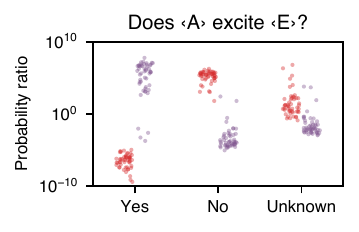}}
        {\includegraphics[width=\linewidth]{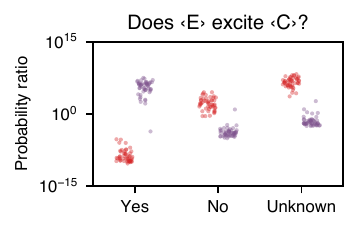}}
        {\includegraphics[width=\linewidth]{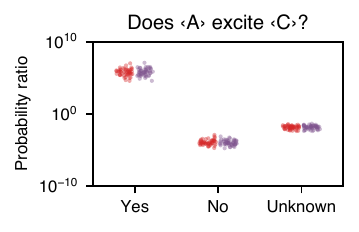}}
        {\includegraphics[width=0.28\textwidth]{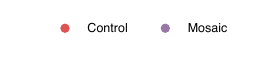}}
    \caption{
        \textbf{Identity--structure separability: neural circuits.}
        Results are shown for Gemma-3-27B.
        The control context is ``‹A› makes glutamatergic projections to ‹B›. ‹B› makes glutamatergic projections to ‹C›'';
        the donor context is ``‹D› makes glutamatergic projections to ‹E›. ‹E› makes glutamatergic projections to ‹F›''.
        The mosaic was constructed as in main-text Fig.~\figref{fig:separability}.
    }
    \label{SI-fig:separability-gemma27b-neural-circuit}
\end{figure*}

\begin{figure*}[!htbp]
    \centering
    \sixpanelgrid
        {\includegraphics[width=\linewidth]{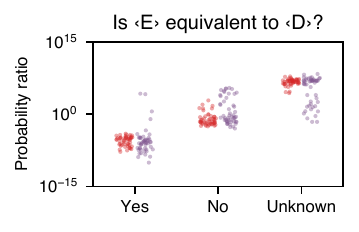}}
        {\includegraphics[width=\linewidth]{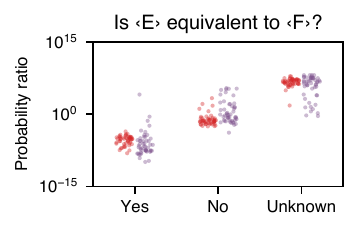}}
        {\includegraphics[width=\linewidth]{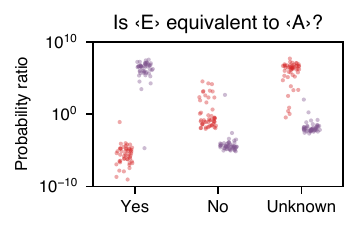}}
        {\includegraphics[width=\linewidth]{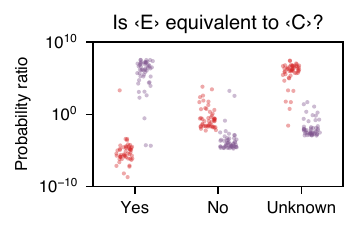}}
        {\includegraphics[width=\linewidth]{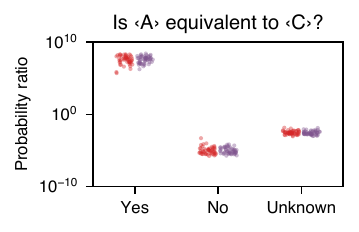}}
        {\includegraphics[width=\linewidth]{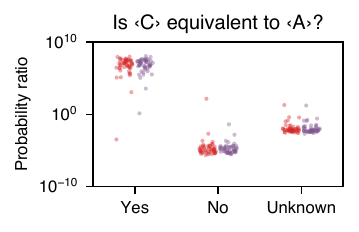}}
        {\includegraphics[width=0.28\textwidth]{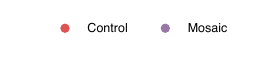}}
    \caption{
        \textbf{Identity--structure separability: propositional equivalence.}
        Results are shown for Gemma-3-27B.
        The control context is ``‹A› is equivalent to ‹B›. ‹B› is equivalent to ‹C›'';
        the donor context is ``‹D› is equivalent to ‹E›. ‹E› is equivalent to ‹F›''.
        The mosaic was constructed as in main-text Fig.~\figref{fig:separability}.
    }
    \label{SI-fig:separability-gemma27b-proposition-equivalence}
\end{figure*}

\begin{figure*}[!htbp]
    \centering
    \sixpanelgrid
        {\includegraphics[width=\linewidth]{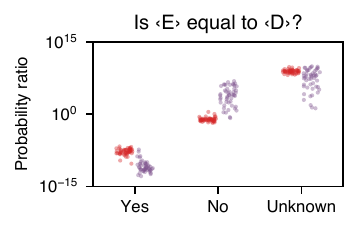}}
        {\includegraphics[width=\linewidth]{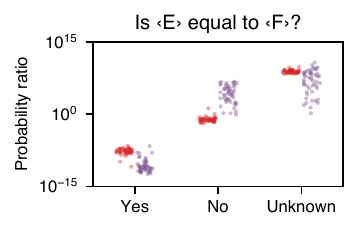}}
        {\includegraphics[width=\linewidth]{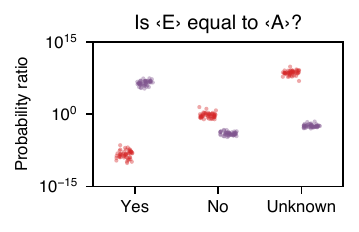}}
        {\includegraphics[width=\linewidth]{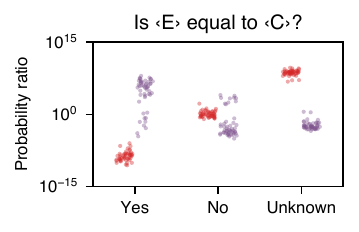}}
        {\includegraphics[width=\linewidth]{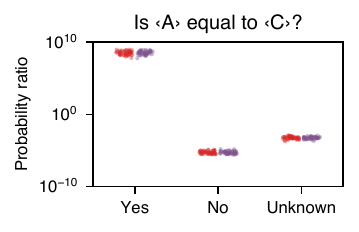}}
        {\includegraphics[width=\linewidth]{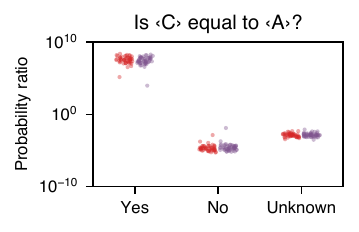}}
        {\includegraphics[width=0.28\textwidth]{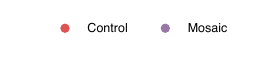}}
    \caption{
        \textbf{Identity--structure separability: variable equality.}
        Results are shown for Gemma-3-27B.
        The control context is ``‹A› is equal to ‹B›. ‹B› is equal to ‹C›'';
        the donor context is ``‹D› is equal to ‹E›. ‹E› is equal to ‹F›''.
        The mosaic was constructed as in main-text Fig.~\figref{fig:separability}.
    }
    \label{SI-fig:separability-gemma27b-variable-equivalence}
\end{figure*}
