# Supplementary material for: Cognitive Maps in Large Language Models
Source: arXiv:2610.25596 source file (2026-11-06)
Supplement: Supplementary file 22 [file supplement.tex]

\onecolumngrid
\clearpage
\makeatletter
\@booleanfalse\twocolumn@sw
\onecolumn@grid@setup
\let\set@footnotewidth\set@footnotewidth@one
\let\compose@footnotes\compose@footnotes@one
\makeatother
\setcounter{section}{0}
\setcounter{subsection}{0}
\setcounter{equation}{0}
\setcounter{figure}{0}
\setcounter{table}{0}
\setcounter{footnote}{0}
\renewcommand{\thefigure}{S\arabic{figure}}
\renewcommand{\theHsection}{SI.\arabic{section}}
\renewcommand{\theHequation}{SI.\arabic{equation}}
\renewcommand{\theHfigure}{SI.\arabic{figure}}
\renewcommand{\theHtable}{SI.\arabic{table}}
\input{supplementary/figure_macros}
\makeatletter
\let\submission@addcontentsline\addcontentsline
\renewcommand{\addcontentsline}[3]{%
  \def\submission@ext{#1}\def\submission@toc{toc}%
  \ifx\submission@ext\submission@toc
    \submission@addcontentsline{sitoc}{#2}{#3}%
  \else
    \submission@addcontentsline{#1}{#2}{#3}%
  \fi
}
\let\submission@starttoc\@starttoc
\let\submission@addtocontents\addtocontents
\renewcommand{\addtocontents}[2]{%
  \def\submission@ext{#1}\def\submission@toc{toc}%
  \ifx\submission@ext\submission@toc
    \submission@addtocontents{sitoc}{#2}%
  \else
    \submission@addtocontents{#1}{#2}%
  \fi
}
\def\@starttoc#1{%
  \def\submission@ext{#1}\def\submission@toc{toc}%
  \ifx\submission@ext\submission@toc
    \submission@starttoc{sitoc}%
  \else
    \submission@starttoc{#1}%
  \fi
}
\makeatother
\pdfbookmark[0]{Supplementary Information}{supplementary-information}
\begin{center}
{\large\bfseries Supplementary Information}
\end{center}
\begingroup
\makeatletter
\let\l@subsection\@gobbletwo
\let\l@subsubsection\@gobbletwo
\makeatother
\tableofcontents
\endgroup
\newpage

\input{supplementary/sections/01_transformer_background}
\input{supplementary/sections/02_mosaic_experiments}
\input{supplementary/sections/03_methods}
\input{supplementary/sections/04_positional_controls}
\input{supplementary/sections/05_prospective_retrospective_more}
\input{supplementary/sections/06_pruning_trajectories}
\input{supplementary/sections/07_who_is_vs_yes_no}
\input{supplementary/sections/08_prompt_templates}
\input{supplementary/sections/09_all_tasks}
\input{supplementary/sections/10_all_models}

\clearpage
\renewcommand{\bibsection}{\section*{References}}
\begingroup
\let\submissionlabel\label
\renewcommand{\label}[1]{\submissionlabel{SI-#1}}
\input{supplementary/references}
\endgroup
